# Supplementary material for: CoHABIT: Complementary Evaluation of Furniture Layouts through Spatial Rules and Household Routines
Source: arXiv:2611.29494 source file (2026-11-22)
Supplement: Supplementary file 1 [file appendix.tex]

\makeatletter
\let\cohabit@addcontentsline\addcontentsline
\renewcommand{\addcontentsline}[3]{\ifstrequal{#1}{toc}{\cohabit@addcontentsline{apptoc}{#2}{#3}}{\cohabit@addcontentsline{#1}{#2}{#3}}}
\makeatother
\twocolumn[{\centering\Large\bfseries Supplementary Material\par\vspace{16pt}}]
\suppressfloats[t]
\setcounter{figure}{0}
\setcounter{table}{0}
\setcounter{equation}{0}
\renewcommand{\thefigure}{S\arabic{figure}}
\renewcommand{\thetable}{S\arabic{table}}
\renewcommand{\theequation}{S\arabic{equation}}
\renewcommand{\theHfigure}{supp.\arabic{figure}}
\renewcommand{\theHtable}{supp.\arabic{table}}
\renewcommand{\theHequation}{supp.\arabic{equation}}
\setcounter{tocdepth}{1}
{\small\makeatletter\@starttoc{apptoc}\makeatother}
\appendix
\setcounter{dbltopnumber}{2}
\renewcommand{\dbltopfraction}{.92}
\renewcommand{\textfraction}{.05}
\input{supplement_sections/a_setup}
\FloatBarrier
\input{supplement_sections/b_static}
\FloatBarrier
\input{supplement_sections/c_dynamic}
\FloatBarrier
\input{supplement_sections/d_paired_quality}
\FloatBarrier
\input{supplement_sections/e_data}
\FloatBarrier
\input{supplement_sections/f_evidence}

\clearpage
\makeatletter
\global\@colroom\textheight
\global\vsize\textheight
\makeatother
\input{supplement_sections/j_final_results}
\input{supplement_sections/k_illustrative_layouts}
