# Supplementary material for: CoHABIT: Complementary Evaluation of Furniture Layouts through Spatial Rules and Household Routines
Source: arXiv:2611.29494 source file (2026-11-22)
Supplement: Supplementary file 2 [file a_setup.tex]

\section{Assessment Inputs and Interpretation}
\label{app:evidence_boundaries}\label{app:reporting_model}\label{app:framework}
A layout $\mathcal{L}=(\Omega,\{B_j,\alpha_j,z_j,\mathcal A_j\}_j,\mathcal D)$ contains metric rooms, furniture footprints, facing, height, affordances and openings. Household $H$ declares movement, reach and carrying capabilities; a scenario fixes original semantic needs, dependencies, releases, deadlines and shared resources. Each matched furnishing comparison preserves envelope, inventory, household, physical starts, original needs, thresholds and exogenous random draws. A profile intervention changes the declared profile while holding the furnishings fixed.
\input{figure_tex/pipeline}

\subsection{Profiles and population}
\label{app:resident-profiles}
The rich furnishing corpus uses standard+fast and standard+wide-clearance households. Daily kitchen comparisons use standard+standard and standard+slow. The reference gallery uses the rich-corpus profiles. Each furnishing pair retains its original ordered household. The static perturbation study instead uses a fixed 0.25\,m navigation radius and 0.10\,m grid.
\begin{table}[t]\centering\small
\caption{Profiles used in the reported cohorts. Lengths are metres; speed is m/s. Each resident carries one portable object. Int. denotes interaction reach.}
\label{tab:resident-profiles}
\begin{tabular}{@{}lrrrrr@{}}\toprule
Profile & Radius & Speed & Reach & Int. & Height\\\midrule
Standard & .25 & 1.20 & 1.50 & .85 & 1.72\\
Fast & .25 & 1.55 & 1.50 & .85 & 1.72\\
Wide-clearance & .40 & .90 & 1.40 & .85 & 1.65\\
Slow & .28 & .65 & 1.40 & .80 & 1.70\\\bottomrule
\end{tabular}\end{table}
Fast changes speed only. Wide-clearance changes radius, speed, reach and stored height together; its contrast is a compound capability intervention. NAV radius determines graph clearance, speed determines traversal duration and reach determines height eligibility. These quantities parameterize the logical simulation. Daily kitchen comparisons replace B's standard profile with the slow capability bundle while holding resident A standard. This intervention jointly changes radius, speed, reach, interaction reach and stored height.

\begin{figure*}[t]\centering
\includegraphics[width=\textwidth]{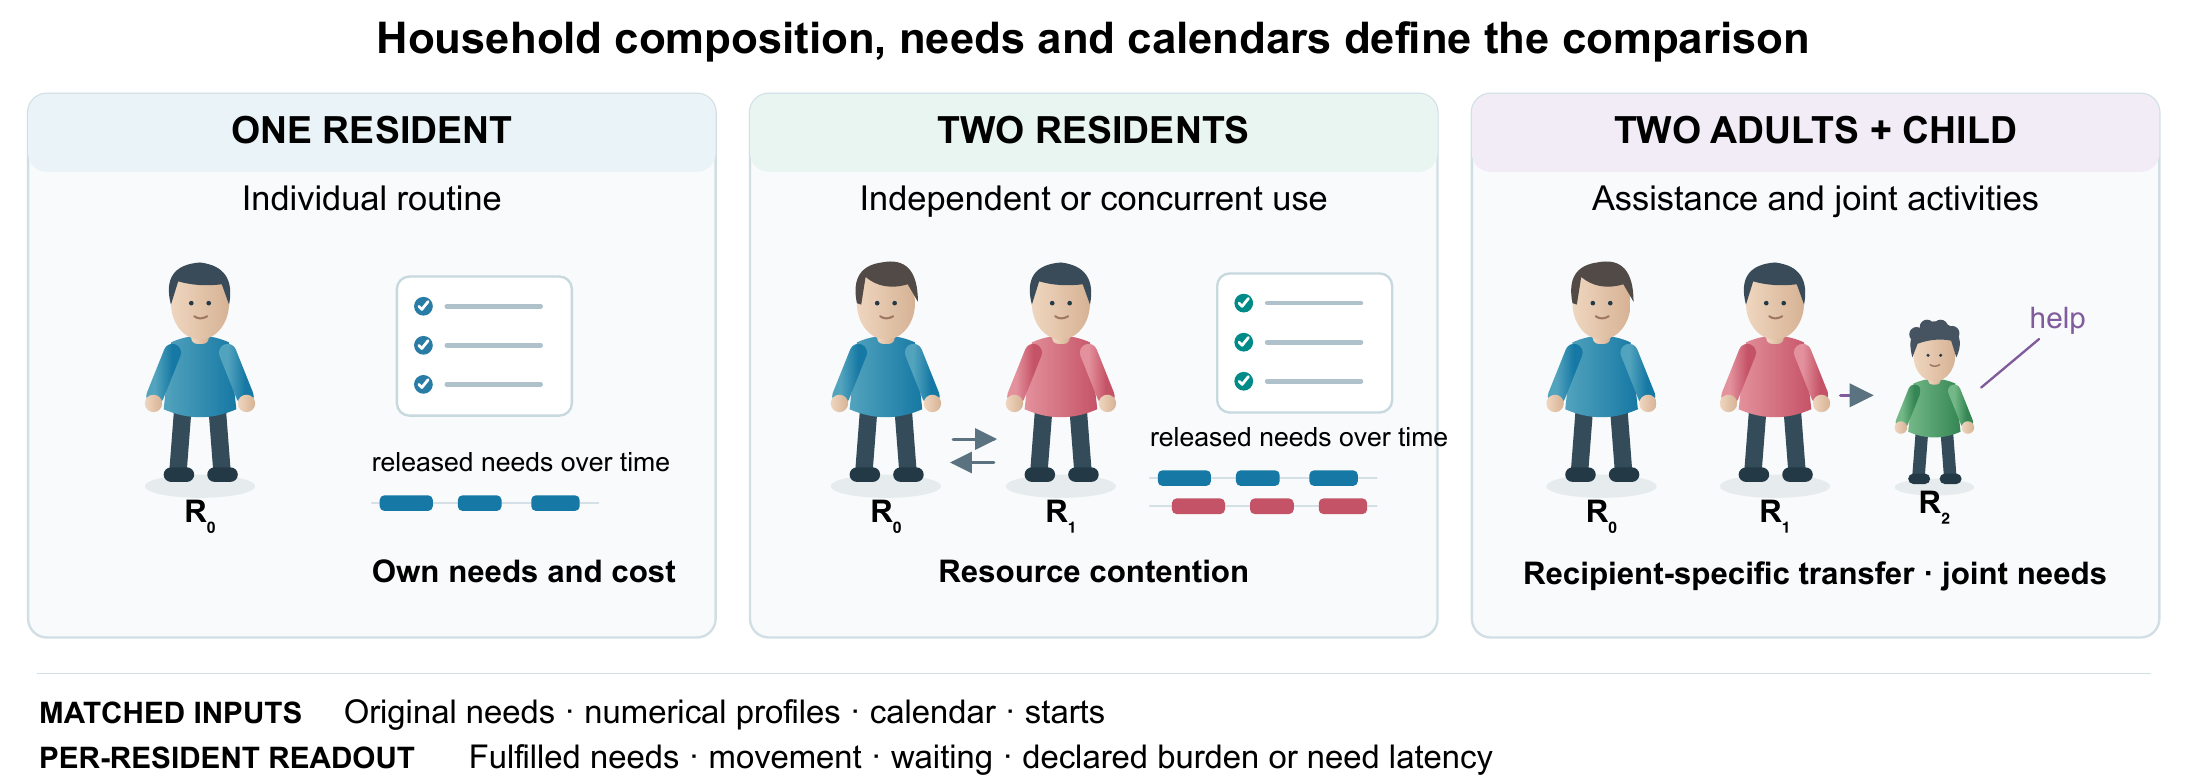}
\caption{\textbf{Declared household compositions and comparison inputs.} Solo and two-resident furnishing contexts are separate from the two-adult-plus-child family series. Each comparison fixes original needs, numerical profiles, calendars and starts, and preserves individual outcomes and costs. Characters and calendar bars schematically identify resident roles and request timing; numerical parameters define the simulated capabilities.}
\label{fig:household-compositions}
\end{figure*}

\subsection{Criteria, needs and verdicts}
Static findings retain criterion identity, applicability, value and affected objects. Dynamic findings retain each resident's original required, met, independently verified-unmet and unresolved needs, together with distance, instrumental time, waiting, deadlines and conflicts. A semantic need is an AND of its required predicates; actions and needs have distinct denominators.

An applicable unavailable criterion is $\bot$; an inapplicable criterion is NA. Coverage is the measured applicable fraction and is undefined for an empty denominator. Each missing value retains its explicit availability state. A positive feasibility verdict requires every original required need and fixed cost limit to be verified. A supported adverse verdict requires a necessity certificate or justified cost attribution under competent execution. Policy loops and unsupported bindings remain unresolved unless independent adverse evidence applies.

The optional certification gate conjoins required geometry with verified dynamic conditions: supported failure prevails, positive requires both branches positive, otherwise the verdict is unknown. G, E, F and D remain separate reports; required failures determine the feasibility gate independently of preferences.
