# Supplementary material for: CoHABIT: Complementary Evaluation of Furniture Layouts through Spatial Rules and Household Routines
Source: arXiv:2611.29494 source file (2026-11-22)
Supplement: Supplementary file 3 [file b_static.tex]

\section{Static Criteria and Perturbation Evidence}
\label{app:static_track}
\label{app:hanfu}

\begin{figure*}[tp]\centering
\includegraphics[width=\textwidth]{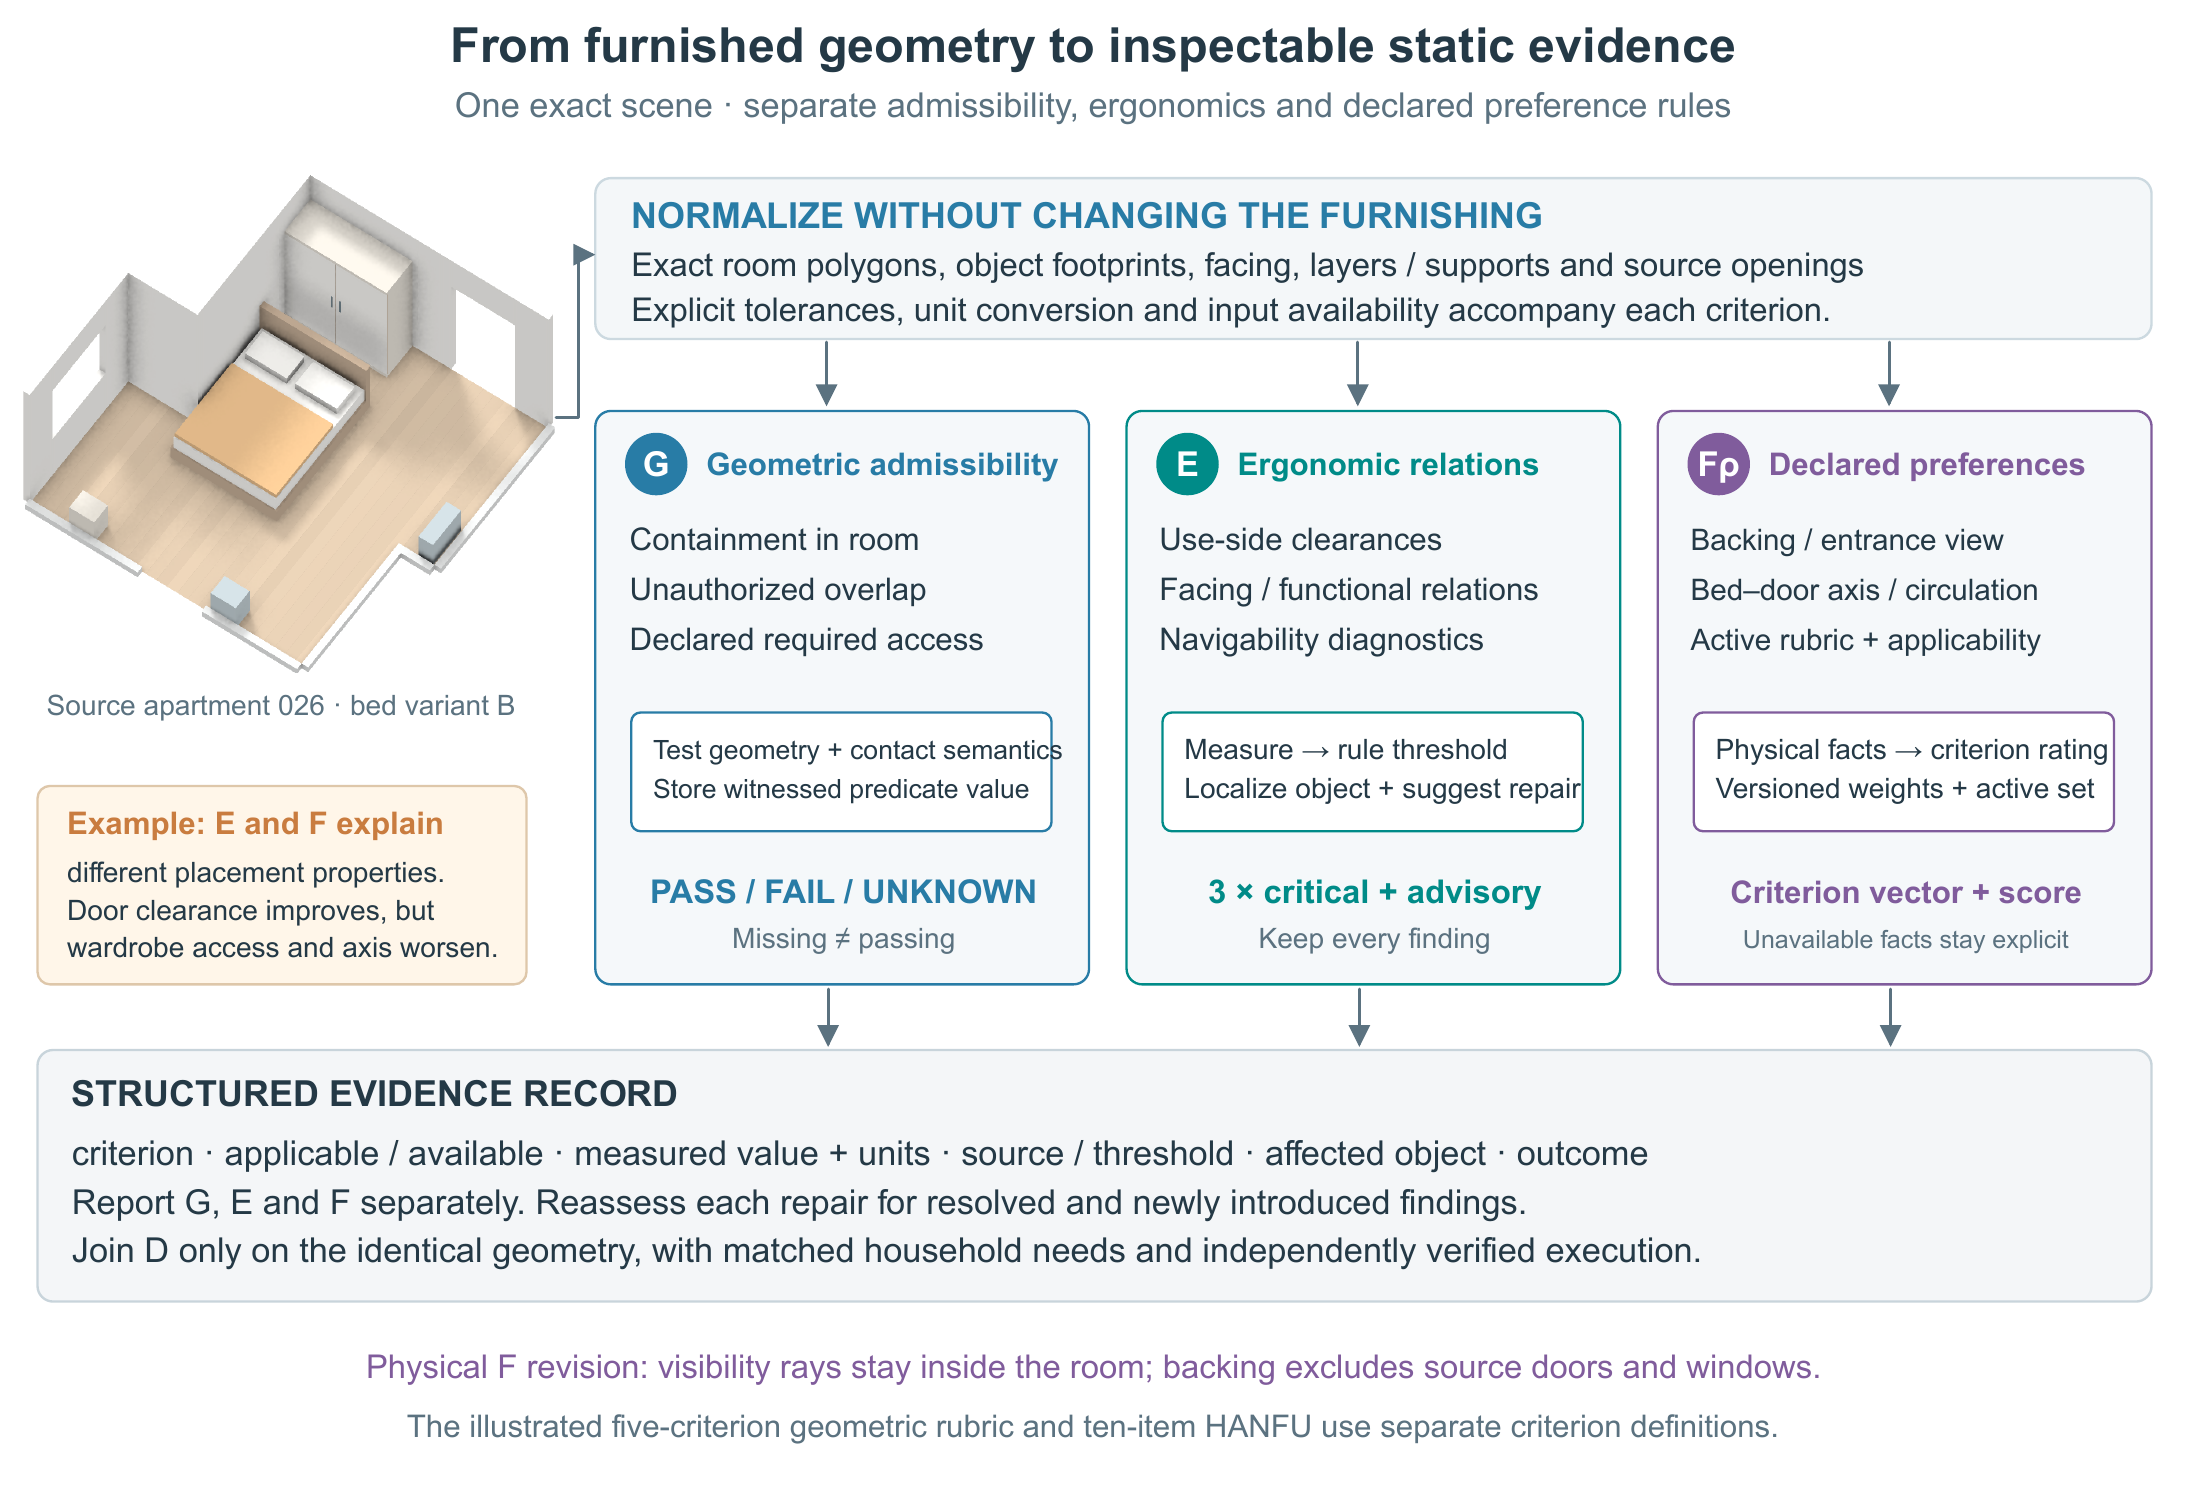}
\caption{\textbf{Static assessment preserves the source and meaning of every criterion.} The source-derived bedroom view shows the tested rotation/translation case. The evaluator retains coordinates and facing, measures geometric and use-side relations, and reports availability and localized witnesses. Required predicates, recommendations and optional spatial preferences remain distinct. The depicted physical preference checks refer to the five-criterion geometric implementation used in our experiments; the complete ten-criterion HANFU rubric is defined below.}
\label{fig:static-algorithm}
\end{figure*}

\subsection{Geometry, ergonomic rules and missing criteria}
For observed metric geometry, example hard predicates are
\begin{align}
h^{\rm inside}_j&=\ind[B_j\subseteq\Omega_{\rm room(j)}],\nonumber\\
h^{\rm overlap}_{jk}&=\ind[\operatorname{area}(B_j\cap B_k)\leq\epsilon_{jk}],
\label{eq:geometric-predicates}
\end{align}
where the overlap test excludes permitted support and containment contacts. Tolerances and contact semantics are declared. Facing-dependent access envelopes use $\alpha_j$ to distinguish orientations with identical footprints. An operational-clearance criterion needs a declared use direction and body profile, together with a sourced threshold. Numerical ergonomic criteria require explicit thresholds, applicability and source references; illustrative drawings supply geometric context.

For measurement $c_j(\mathcal{L},p)$, a declared map gives $s_j=\psi_j(c_j;p)$. A possible clearance map is $\psi_j(d;p)=\operatorname{clip}(d/\eta_j(p), 0, 1)$, but $\eta_j(p)$ still requires grounding. An ordinal $K_j$-level preference can use $(c_j-1)/(K_j-1)$. Each normalized score retains its criterion-specific meaning.

Record applicability $a_j$ and availability $m_j$ using the missingness conventions in Appendix~A. For a nonempty set $\mathcal H_p$ of applicable required hard checks,
\begin{equation}
G_{\rm req}=\begin{cases}
\mathrm{FAIL},&\exists j\in\mathcal H_p:m_j=1,\ h_j=0,\\
\mathrm{PASS},&\forall j\in\mathcal H_p:m_j=1,\ h_j=1,\\
\mathrm{UNKNOWN},&\text{otherwise}.
\end{cases}
\label{eq:hard-status}
\end{equation}
An unspecified check set is UNKNOWN. Criterion coverage is $\sum_ja_jm_j/\sum_ja_j$, unavailable when the denominator is empty. Unknown values retain a distinct status. Hard failures receive localized diagnoses; soft ergonomic deficits and preferences remain inspectable. Comparisons among passing layouts use the same criterion and household contract and retain tradeoffs.

\input{supplement_sections/b_static_methods}

\subsection{Static controls and edits}
The static set contains 50 furnished controls with six edits each: shift, $180^\circ$ orientation change, door blocking, overlap, wall crossing and combined edits. Thus it contains 350 scenes and 300 control--edit pairs. Apartments have 4--8 rooms, 17--35 objects and 44.01--100\,m$^2$ area. They derive from 19 source layouts in 11 outer-contour families. The supplied split has 37/5/8 controls across 8/1/2 train/validation/test families.

These data were collected for static assessment. Their furnishing briefs specify static design conditions; dynamic residents use separately declared simulator profiles. Edit labels specify intended local degradation relative to the selected controls. Some edits introduce several defects. An evaluator should therefore report pair preference, ties and object-level diagnosis separately. Local finding detection and aggregate pair ordering are evaluated separately.

\begin{table}[t]\centering\small
\caption{Audit of supplied static annotations; each row has 50 scenes. Counts report scenes with at least one stored violation.}
\label{tab:static}
\begin{tabular}{@{}lrrr@{}}\toprule
Edit & Overlap & Opening & Outside\\\midrule
Control &0&0&0\\
Shift &50&2&0\\
Orientation $180^\circ$ &0&0&0\\
Door block &0&50&0\\
Overlap &50&10&0\\
Wall crossing &9&4&50\\
Combined &50&39&0\\\bottomrule
\end{tabular}\end{table}
All 50 orientation edits preserve the three geometry checks in Table~\ref{tab:static}. Their stored front-blocking diagnostic increases from .3170 to .3700 on average (paired difference +.0530). This quantifies orientation-sensitive use-side access at unchanged footprints.

\input{supplement_sections/b_static_results}

\subsection{Optional preference criteria}
HANFU is the spatial-preference rubric of CoHABIT, complementing its physical-feasibility assessment. Combining scores requires compatible context and criterion meanings.
\begin{table}[t]\centering\small
\caption{CoHABIT's ten-criterion HANFU rubric. Each rating uses explicitly supplied contextual attributes.}
\begin{tabularx}{\linewidth}{@{}lYl@{}}\toprule
ID & Criterion & Scale\\\midrule
F1 & Bed commanding position & 1--4\\
F2 & Desk commanding position & 1--4\\
F3 & Sofa commanding position & 1--3\\
F4 & Bagua alignment & 1--4\\
F5 & Kitchen positioning & 1--4\\
F6 & Directed-corner/alignment avoidance & 1--3\\
F7 & Door--bed alignment & 1--2\\
F8 & Mirror placement & 1--2\\
F9 & Elemental balance & 1--3\\
F10 & Yin--yang zoning & 1--3\\\bottomrule
\end{tabularx}\end{table}
Commanding-position criteria require orientation, entrance and backing geometry; directional criteria need compass bearing and declared sectors; mirror and material criteria need corresponding attributes. Incompatible legacy meanings, especially F5, prevent criterion-level comparison across implementations.

For fixed active, applicable criteria $\mathcal A_p$ and declared nonnegative weights, an optional summary requires every active rating:
\begin{equation}
F_p(\mathcal{L})=\frac{\sum_{c\in\mathcal A_p}w_c(s_c-1)}{\sum_{c\in\mathcal A_p}w_c(K_c-1)}.
\end{equation}
A missing active rating or zero denominator yields an unavailable scalar while preserving the fixed active set. Reports retain the vector, active set, missingness and coverage. Changing that set changes the interpretation. The five-criterion results above measure agreement with that rubric and its synthetic targets; HANFU retains its own criterion definitions.

\begin{center}
\includegraphics[width=\linewidth]{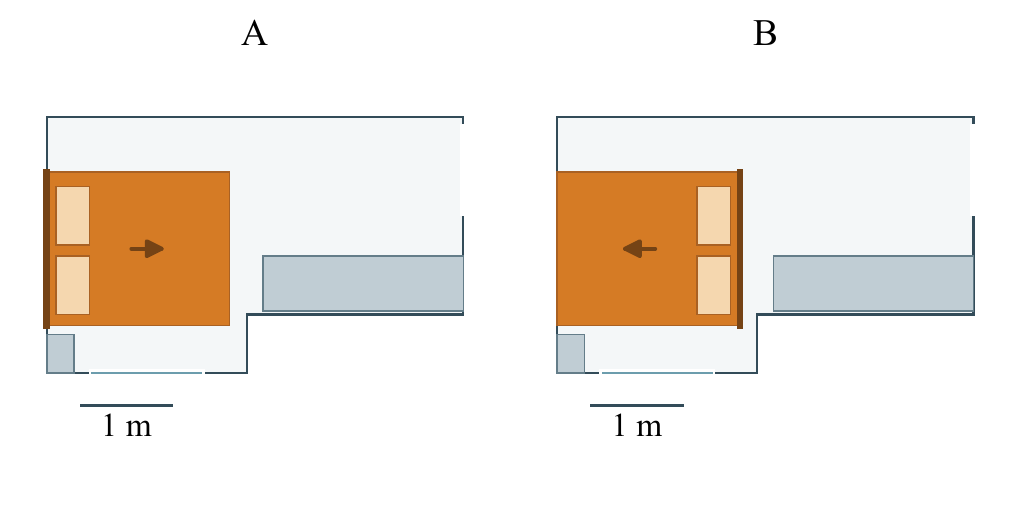}
\captionof{figure}{\textbf{The source geometry behind the main-paper headboard example.} A $180^\circ$ bed rotation preserves every furniture footprint, room and opening of the eight-room control. The explicit F1 headboard-support subrule changes: oriented rear-edge contact with the solid room boundary falls from 1.68\,m to zero (openings excluded; $10^{-6}$\,m tolerance). This local geometric witness is separate from ordinal five-criterion ratings and the 48-pair comparison.}
\label{fig:headboard-source}
\end{center}

\paragraph{Motivating example: clearance and routine completion.}
Figure~\ref{fig:chair-clearance-3d} shows the same apartment before and after a furnishing intervention: the critic's dining-chair clearance decreases from 0.64 to 0.44\,m. The implemented 0.60-m chair-use threshold is satisfied only in A; neither meets its 0.80-m recommendation for passage behind a seated person. Both layouts complete the declared routines (Appendix~H), while the reduced clearance changes the space available for using the chair. This motivates complementary spatial and temporal assessment on the same furnishings. Figure~\ref{fig:vlm-access-3d} provides complementary sink-facing and door-zone examples.
\begin{figure*}[tp]\centering
\begin{minipage}{.48\textwidth}\centering
\textbf{A: wider chair-use clearance}\\
\includegraphics[width=\linewidth]{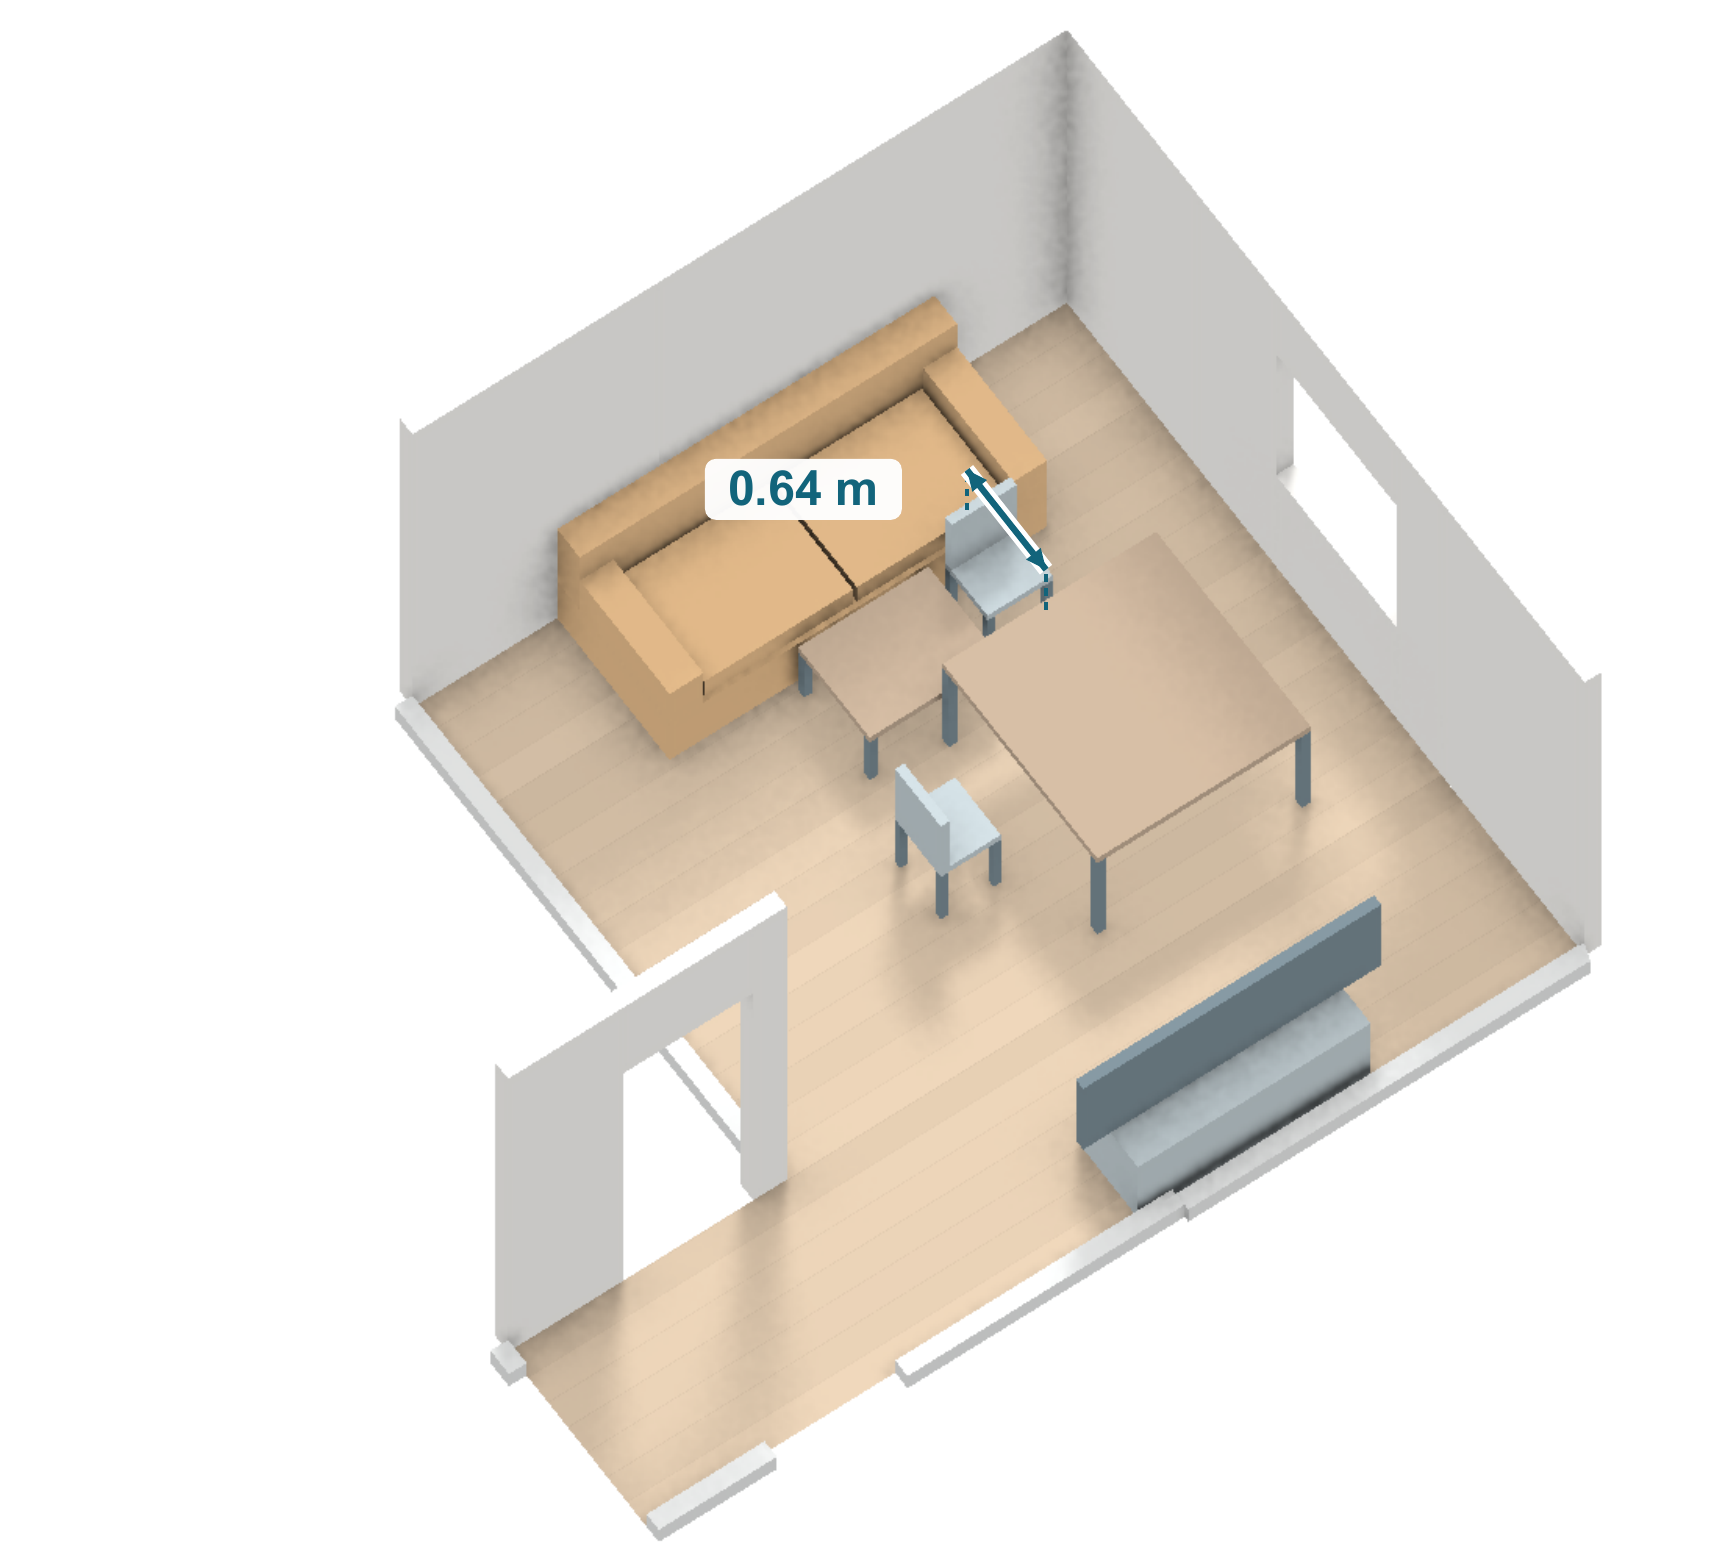}\\
Measured clearance: 0.64\,m
\end{minipage}\hfill
\begin{minipage}{.48\textwidth}\centering
\textbf{B: narrower chair-use clearance}\\
\includegraphics[width=\linewidth]{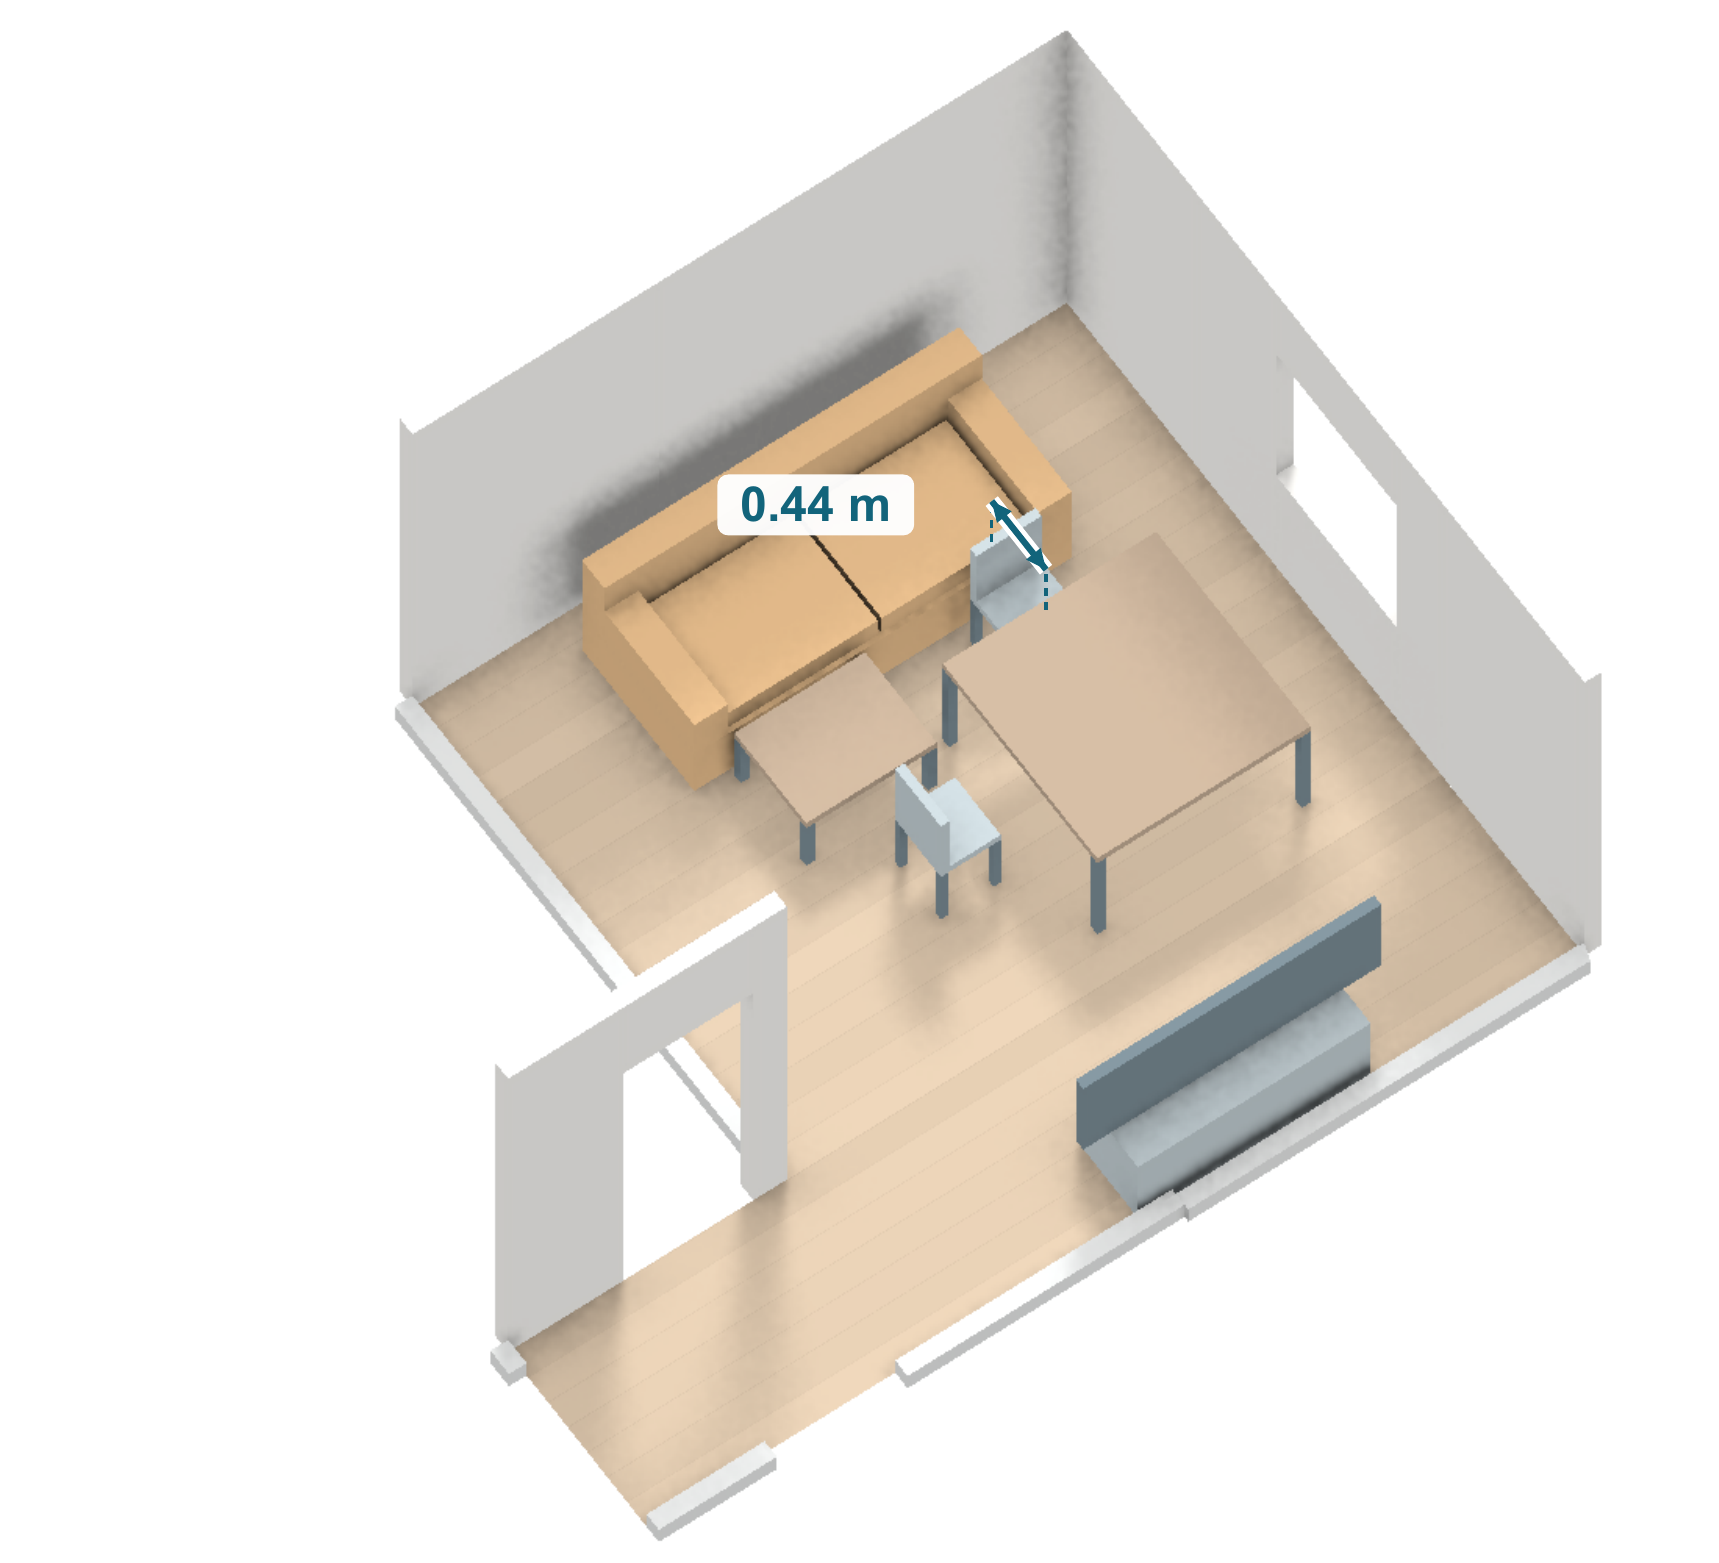}\\
Measured clearance: 0.44\,m
\end{minipage}
\caption{\textbf{Geometric clearance adds information beyond completed routines.} Source-bound 3D views of apartment 026 under the living-room intervention in Appendix~H. Dimension arrows mark the table-edge-to-sofa clearance across the chair-use zone; 0.64\,m in A meets the implemented 0.60-m chair-use threshold, whereas 0.44\,m in B does not. The 0.80-m recommendation for passage behind a seated person is unmet in both. The camera, scale and lighting are shared; footprints and orientations follow the evaluated JSON, while materials and heights are illustrative. Both variants complete the household routine; the narrower chair-use space illustrates the additional information supplied by ergonomic checks.}
\label{fig:chair-clearance-3d}
\end{figure*}
