# Supplementary material for: CoHABIT: Complementary Evaluation of Furniture Layouts through Spatial Rules and Household Routines
Source: arXiv:2611.29494 source file (2026-11-22)
Supplement: Supplementary file 4 [file b_static_methods.tex]

\subsection{From geometric measurements to criterion reports}
Figure~\ref{fig:static-algorithm} traces the implemented measurements from furnished geometry to separate G, E and preference records. Algorithm~1 makes applicability, availability and the original rubric explicit. $G$ is computed from the required checks only, whereas $E$ aggregates all findings of the geometry/ergonomics critic, including recommendations. Proposed repairs are evaluated as new layouts, checking both resolved and newly introduced findings.



\begin{table*}[t]\centering\small
\begin{tabularx}{\textwidth}{@{}rY@{}}\toprule
\multicolumn{2}{@{}l}{\textbf{Algorithm 1. Static criteria with explicit availability}}\\\midrule
\textbf{Input}&Furnished geometry $\mathcal{L}$, household $H$, preference rubric $\rho$, criterion registry $\mathcal R$.\\
\textbf{Output}&Separate reports $G,E,F_\rho$ and localized evidence records $\mathcal Z$.\\\midrule
1&$\widehat{\mathcal{L}}\gets\operatorname{Normalize}(\mathcal{L})$; retain coordinates, facing, supports and source-opening correspondence.\\
2&$\mathcal Z\gets\varnothing$.\\
3&\textbf{for each} criterion $r\in\mathcal R$ \textbf{do}\\
4&\quad Determine applicability from $(\widehat{\mathcal{L}},H,\rho)$; record inactive criteria without scoring them.\\
5&\quad \textbf{if} required attributes are unavailable, append an unavailable record and \textbf{continue}.\\
6&\quad $m_r\gets\operatorname{Measure}_r(\widehat{\mathcal{L}},H)$ with declared units and geometry tolerances.\\
7&\quad $v_r\gets\operatorname{Evaluate}_r(m_r;\rho)$; retain the measured fact, rule source and affected objects.\\
8&\quad Append $(r,m_r,v_r,\mathrm{source},\mathrm{availability},\mathrm{witness})$ to $\mathcal Z$.\\
9&$G\gets\operatorname{RequiredVerdict}(\mathcal Z)$ using only records of required checks: verified failure dominates; otherwise missing required evidence yields UNKNOWN.\\
10&$E\gets3n_{\mathrm{critical}}+n_{\mathrm{advisory}}$ over geometry/ergonomics findings in $\mathcal Z$, including hard checks and recommendations; retain the full finding list.\\
11&$F_\rho\gets\operatorname{PreferenceReadout}(\mathcal Z;\rho)$ with fixed active criteria and versioned aggregation.\\
12&\textbf{return} $(G,E,F_\rho,\mathcal Z)$; a proposed repair must be evaluated as a new layout.\\\bottomrule
\end{tabularx}
\end{table*}
