# Supplementary material for: CoHABIT: Complementary Evaluation of Furniture Layouts through Spatial Rules and Household Routines
Source: arXiv:2611.29494 source file (2026-11-22)
Supplement: Supplementary file 5 [file b_static_results.tex]

\subsection{Static comparison protocol}
\label{app:static_archive_evidence}
\textbf{Reported} values are archive summaries; \textbf{rechecked} values are recomputed from individual records; \textbf{post-hoc} comparisons reuse the inspected pairs. Pair accuracy awards one for preferring the control, one half for a tie and zero otherwise. Strict correctness excludes ties. Detection counts new critical findings; localization checks the changed object; repair counts removed findings. These are distinct targets.

The selected corpus contains 50 furnished controls from 19 source layouts and 11 contour families, with six edits per control. The training/validation/test splits contain 222/30/48 pairs, 37/5/8 controls and 8/1/2 contour families. The test controls come from three source layouts; six controls share one contour family and two share the other. Counts refer to the selected controls.

The geometry/ergonomics critic ranks by $3n_{\rm critical}+n_{\rm advisory}$, lower being better. SceneEval~\cite{tam2026sceneeval} and SceneSmith~\cite{pfaff2026scenesmith} supply the archived baseline comparisons. The VLM judge uses the recorded gemini-4-argon endpoint (alias argon) to view plans with icons and randomized A/B order. The static--VLM cascade queries its judge when the rule-score gap is below three, approximately 20\% of pairs. It combines two static instruments.

\subsection{Reported ranking, localization and repair}
Tables~\ref{tab:static-full-ranking} and~\ref{tab:static-by-kind} give the full comparison and edit-specific values.
\begin{table}[t]\centering\small
\setlength{\tabcolsep}{3pt}
\caption{\textbf{Reported} pair accuracy (half-credit ties) and strict correctness. All: 300 pairs; Test: 48 pairs. Unreported strict values use --.}
\label{tab:static-full-ranking}
\begin{tabular}{@{}lrrr@{}}\toprule
Method & All & Test & Strict (all)\\\midrule
Geometry/ergonomics & .917 & .958 & .883\\
SceneEval COL & .770 & .771 & .543\\
SceneEval OOB & .555 & .542 & .110\\
NAV 0.2\,m & .408 & .312 & .287\\
NAV 0.6\,m & .478 & .583 & .373\\
ACC side table & .667 & .625 & .573\\
ACC VLM sides & .627 & .521 & .563\\
Door zones & .663 & .698 & .337\\
Window zones & .500 & .500 & .000\\
SceneSmith reach 0.3\,m & .547 & .479 & .307\\
SceneSmith reach 0.6\,m & .572 & .635 & .350\\\midrule
Reimpl. collision fraction & .778 & .771 & .557\\
Reimpl. out-of-bounds & .555 & .542 & .110\\
Reimpl. overlap rate & .778 & .771 & .560\\
Reimpl. orientation & .605 & .667 & .220\\
Reimpl. reachable rate & .637 & .604 & .347\\\midrule
VLM judge & .948 & .948 & \NM\\
Static--VLM cascade & .983 & .990 & \NM\\\bottomrule
\end{tabular}\end{table}

Table~\ref{tab:static-full-ranking} evaluates all instruments on the six local-edit types; the baseline methods originate in generator-comparison settings. A finding can be detected while other penalties reverse the aggregate ranking. The critic reports .98 finding detection, .917 half-credit pair accuracy and .883 strict pair accuracy, each with its stated target. Table~\ref{tab:static-by-kind} uses the same half-credit metric in every cell. The window-zone baseline ties every pair: half-credit accuracy .500 with strict correctness .000.

\begin{table}[t]\centering\small
\setlength{\tabcolsep}{3pt}
\caption{\textbf{Reported} half-credit accuracy by edit, 50 pairs per row. Cascade combines the rule critic with the same VLM judge.}
\label{tab:static-by-kind}
\begin{tabular}{@{}lrrr@{}}\toprule
Edit & Rules & VLM & Cascade\\\midrule
Shift & .88 & .96 & \textbf{.98}\\
Rotation & .95 & .78 & \textbf{.96}\\
Door block & .95 & .98 & \textbf{1.00}\\
Overlap & .85 & \textbf{1.00} & \textbf{1.00}\\
Wall crossing & .87 & \textbf{.99} & .96\\
Combined & \textbf{1.00} & .98 & \textbf{1.00}\\\bottomrule
\end{tabular}\end{table}

\paragraph{Error mechanisms in preserved examples.}
On rotations, rules improve on the VLM judge from .78 to .95 and the cascade reaches .96. Figures~\ref{fig:vlm-access-3d}--\ref{fig:vlm-overlap-3d} reconstruct four preserved comparisons: working-side orientation, door-zone obstruction, a table/chair intersection, and sofa/table overlaps. The first three show how local geometric measurements explain individual disagreements between rules and the visual judge. The fourth separates diagnosis from ranking: the critic detects overlaps but its aggregate penalty prefers the edit. These selected examples explain mechanisms; category frequencies are reported in Table~\ref{tab:static-by-kind}. Use-side clearance has no separately scored category beyond these rotation examples. The displacement-dose test below evaluates the rule critic only.

\input{figure_tex/vlm_examples_3d}

\paragraph{External-query cost.}
The local rule critic makes no external API requests. At the recorded approximately 20\% judge-call rate, the cascade uses about 80\% fewer requests than judging every pair. Historical archive estimates are approximately \$0.008 per pair for the VLM judge and \$0.0015 for its cascade. Five saved examples retain per-response charges of \$0.00638--0.00792. These recorded estimates and response charges characterize historical API expense; matched local CPU cost is outside this comparison.

\paragraph{Reported uncertainty.}
The archived bootstrap uses 4,000 resamples of the 50 generated controls, carrying all six edits with each selected control (random seed 0). Its reported 95\% intervals are critic .917 [.888,.945], VLM judge .948 [.927,.967] and cascade .983 [.970,.993]. These intervals, reproduced in the main table where available, describe variation over generated controls, conditional on the selected source geometry; they include training and validation controls. Controls are resampled with their six edits; source layouts and contour families are not resampling units. Table~\ref{tab:static-paired-ci} preserves the archived paired differences. The 48-pair test gives a descriptive comparison of observed scores on two held-out contour families.

\begin{table}[t]\centering\small
\caption{\textbf{Reported} paired differences on 300 pairs, with 95\% intervals resampling the 50 generated controls. See the stated conditional uncertainty scope.}
\label{tab:static-paired-ci}
\begin{tabular}{@{}lrr@{}}\toprule
Comparison & Difference & 95\% interval\\\midrule
Critic minus VLM & $-.032$ & [$-.065,.002$]\\
Cascade minus VLM & $+.035$ & [.017,.055]\\\bottomrule
\end{tabular}\end{table}

The critic--VLM difference interval spans zero. The cascade--VLM interval is positive under the stated control-level resampling. The recorded strict-correctness McNemar tests operate at pair level. Probabilities displayed as zero are rounded values. These pair-level summaries leave geometry-clustered significance unevaluated.

\paragraph{Reported object-level diagnosis and repair.}
New findings name the changed item in 243/250 single-defect pairs. A new critical finding appears in 294/300 pairs; these pairs yield 560 new findings, of which 64\% reportedly have an automatic fix. Three rounds remove 422/560 findings (75.36\%; Table~\ref{tab:static-repair}). The reported 16\% repair-regression figure is retained as a summary statistic with an unspecified event denominator. Each repaired layout requires a full reassessment of resolved and newly introduced findings. The 141/273 slide-summary count and 422/560 finding count describe separate runs and are reported separately.

\begin{table}[t]\centering\small
\caption{\textbf{Reported} new findings and removals after three rounds. The counting unit is an individual finding.}
\label{tab:static-repair}
\begin{tabular}{@{}lrr@{}}\toprule
Edit & New findings & Removed\\\midrule
Shift & 93 & 82\\
Rotation & 47 & 47\\
Door block & 82 & 77\\
Overlap & 85 & 41\\
Wall crossing & 71 & 42\\
Combined & 182 & 133\\\midrule
\textbf{Total} & 560 & \textbf{422}\\\bottomrule
\end{tabular}\end{table}

\subsection{Post-hoc check selection and score diagnostics}
\label{app:static_posthoc}
The ablation tables separate check selection, individual contributions and scalar weighting; their common limitation is reuse of the inspected pairs.
\textbf{Exploratory analysis on the inspected pairs.} The hard-plus-orientation subset in Table~\ref{tab:static-posthoc} was selected on these pairs. Its .983 overall and .990 test-subset scores therefore describe post-hoc performance on reused data. Here ``hard'' denotes implemented collision, out-of-bounds and door/window checks; required resident conditions have a separate definition. The scalar assigns critical severity to some recommendations, including gaps; household applicability is specified separately. The archive retained the gap check despite its adverse ranking delta. Recommendation checks require further grounding even when they improve synthetic edit ranking.

\begin{table}[t]\centering\small
\caption{\textbf{Post-hoc reported diagnostics} on the same 300 pairs; half-credit ties. The selected subset also reports .990 on the reused 48-pair test subset, without independent selection.}
\label{tab:static-posthoc}
\begin{tabular}{@{}lrr@{}}\toprule
Findings scored & All & Rotation (50)\\\midrule
Hard checks only & .912 & .50\\
Recommendations only & .618 & .95\\
Orientation only & .662 & .95\\
Hard plus orientation (selected) & \textbf{.983} & .95\\
All checks (main comparison) & .917 & .95\\\bottomrule
\end{tabular}\end{table}

Reported leave-one-check-out changes in pair accuracy are collision $-.108$, opening clearance $-.092$, orientation $-.075$, out-of-bounds $-.062$, bed access $-.003$, door reachability $-.002$, dining-chair space $+.005$, navigability $+.007$ and gap violations $+.062$; the other nine checks change the rounded score by zero. A zero delta records unchanged aggregate accuracy on these interventions. Critical:advisory weights 1: 1, 2: 1, 3: 1, 5: 1 and 10: 1 give .862, .905, .917, .917 and .917; critical-only scoring gives .930. These same-data diagnostics measure sensitivity to aggregation and preexisting control penalties; validation of alternative weights requires a separate selection-and-test protocol.

\subsection{Reported judge stability and findings assistance}
Repeated-judge results cover a 90-pair subset (Table~\ref{tab:static-repeats}). Similar aggregate accuracy can coexist with changes in individual verdicts.

\begin{table}[t]\centering\small
\caption{\textbf{Reported} repeat stability. Agreement is the fraction retaining the same verdict across the listed repeats.}
\label{tab:static-repeats}
\begin{tabular}{@{}lrrl@{}}\toprule
Judge & Pairs & Repeats & Accuracy; agreement\\\midrule
VLM judge & 90 & 2 & .944, .933; .978\\\bottomrule
\end{tabular}\end{table}

Providing critical findings defines an additional prompt condition under the same evaluation labels. The reported matched-subset results are in Table~\ref{tab:static-findings}. The all-pair subsets differ from 300 and their test slices differ from 48. Orientation accuracy changes from .793 to .939 (41 pairs). On the 42-pair test slice, the aggregate score remains unchanged. On the all-pair matched subset, cascade accuracy decreases from .9826 to .9807 with findings assistance. Repeat and assisted-prompt results use the saved summary statistics.

\begin{table}[t]\centering\small
\caption{\textbf{Reported} findings-assisted judge accuracy and ties on matched subsets. Test rows are nested subsets of the corresponding all rows.}
\label{tab:static-findings}
\begin{tabular}{@{}llrrr@{}}\toprule
Judge & Subset ($n$) & Base & Findings & Ties, base$\to$new\\\midrule
VLM & All (259) & .9498 & .9826 & 18$\to$5\\
VLM & Test (42) & \textbf{.9524} & \textbf{.9524} & 4$\to$2\\\bottomrule
\end{tabular}\end{table}

\subsection{Arithmetic recheck: shift-dose records}
We independently recomputed Table~\ref{tab:static-dose} from 200 supplied individual records: the same 50 controls at each of four displacement magnitudes. This recheck verifies arithmetic and denominators of the saved checker outputs. Pair ordering reflects displacement alongside all other scored penalties. Target objects and directions are selected using overlap at the largest tested displacement. The displacement-dose evaluation covers the rule critic.

\begin{table}[t]\centering\small
\caption{\textbf{Arithmetic rechecked from saved checker outputs}. Each magnitude has 50 pairs; accuracy credits ties by one half, detection counts a new critical finding.}
\label{tab:static-dose}
\begin{tabular}{@{}lrr@{}}\toprule
Displacement & Pair accuracy & Detection\\\midrule
0.05\,m & .77 & .56\\
0.10\,m & .86 & .82\\
0.20\,m & \textbf{.93} & \textbf{.98}\\
0.40\,m & .92 & \textbf{.98}\\\bottomrule
\end{tabular}\end{table}

\subsection{Preference experiments and criterion definitions}
\label{app:five_criterion_preferences}
The five-criterion spatial-preference rubric defines F1 backing support, F3 entrance view, F5 circulation, F7 angle exposure and F10 density. These criterion definitions and results are reported separately from the complete HANFU rubric below. Its results measure agreement with synthetic interventions under those definitions.

From the supplied 48 test-pair records and 98 scene-status records, we recomputed image-based argon preference accuracy .7292, geometry-based preference accuracy .5833 and ergonomics accuracy .9583. The ergonomics-first, image-preference-on-ties tandem scores .979, resolving two critic ties; it is comparable to the .958 critic on this small subset. Image preference scores .375 on the eight shift pairs. This task scores scenes under the preference rubric, whereas the main table's judge compares ergonomic edits directly.

Rechecking the archived results gives geometry-preference/ergonomics/tandem accuracies of .560/.917/.918 on 300 ergonomic pairs and .704/.621/.723 on 157 preference-targeted pairs. The records are available from the authors. These saved evaluations use an earlier ergonomics-critic version and reveal sensitivity to criterion choice. The image comparison uses one VLM on eight test controls, with 48 paired interventions. The reported scene-score correlation $r=.33$, approximately 3.5 attempts per valid image response and 44\% unrated criteria likewise lack complete independent regeneration. Output validity, scene judgment and criterion coverage are recorded as distinct quantities.

\begin{table}[t]\centering\small
\caption{\textbf{Reported room-level exact agreement} between geometry and image modes of the experimental preference implementation. Counts are transcribed from the reported room-rating summaries.}
\label{tab:static-preference-agreement}
\begin{tabular}{@{}llrr@{}}\toprule
ID & Preference criterion & Agree / total & \%\\\midrule
F1 & Backing support & 60/106 & 56.6\\
F3 & Entrance view & 56/98 & 57.1\\
F5 & Circulation & 197/401 & 49.1\\
F7 & Angle exposure & 61/106 & 57.5\\
F10 & Density & 275/401 & \textbf{68.6}\\\bottomrule
\end{tabular}\end{table}



\subsection{Record provenance}
Reported rankings, detection, localization, repair and judge statistics are transcribed from their respective archive summaries. Arithmetic checks cover the 200 displacement comparisons, the 48-pair preference test, and the 300- and 157-pair preference/ergonomics comparisons. These evidence types retain separate labels throughout the section. The measured figures use the corresponding static records; dynamic rollout figures use recorded apartment executions.
