# Supplementary material for: CoHABIT: Complementary Evaluation of Furniture Layouts through Spatial Rules and Household Routines
Source: arXiv:2611.29494 source file (2026-11-22)
Supplement: Supplementary file 6 [file c_architecture_learning.tex]

The resident computation in Figure~\ref{fig:architecture-detailed} is bound to the pinned daily implementation. Schematic residents denote separately acting decision makers with shared weights. Their actions change one persistent apartment state; original-need assessment is independent of the training objective. The 3D thumbnail reuses exact source furnishing geometry with illustrative materials and heights.

\begin{figure*}[tp]\centering
\includegraphics[width=\textwidth]{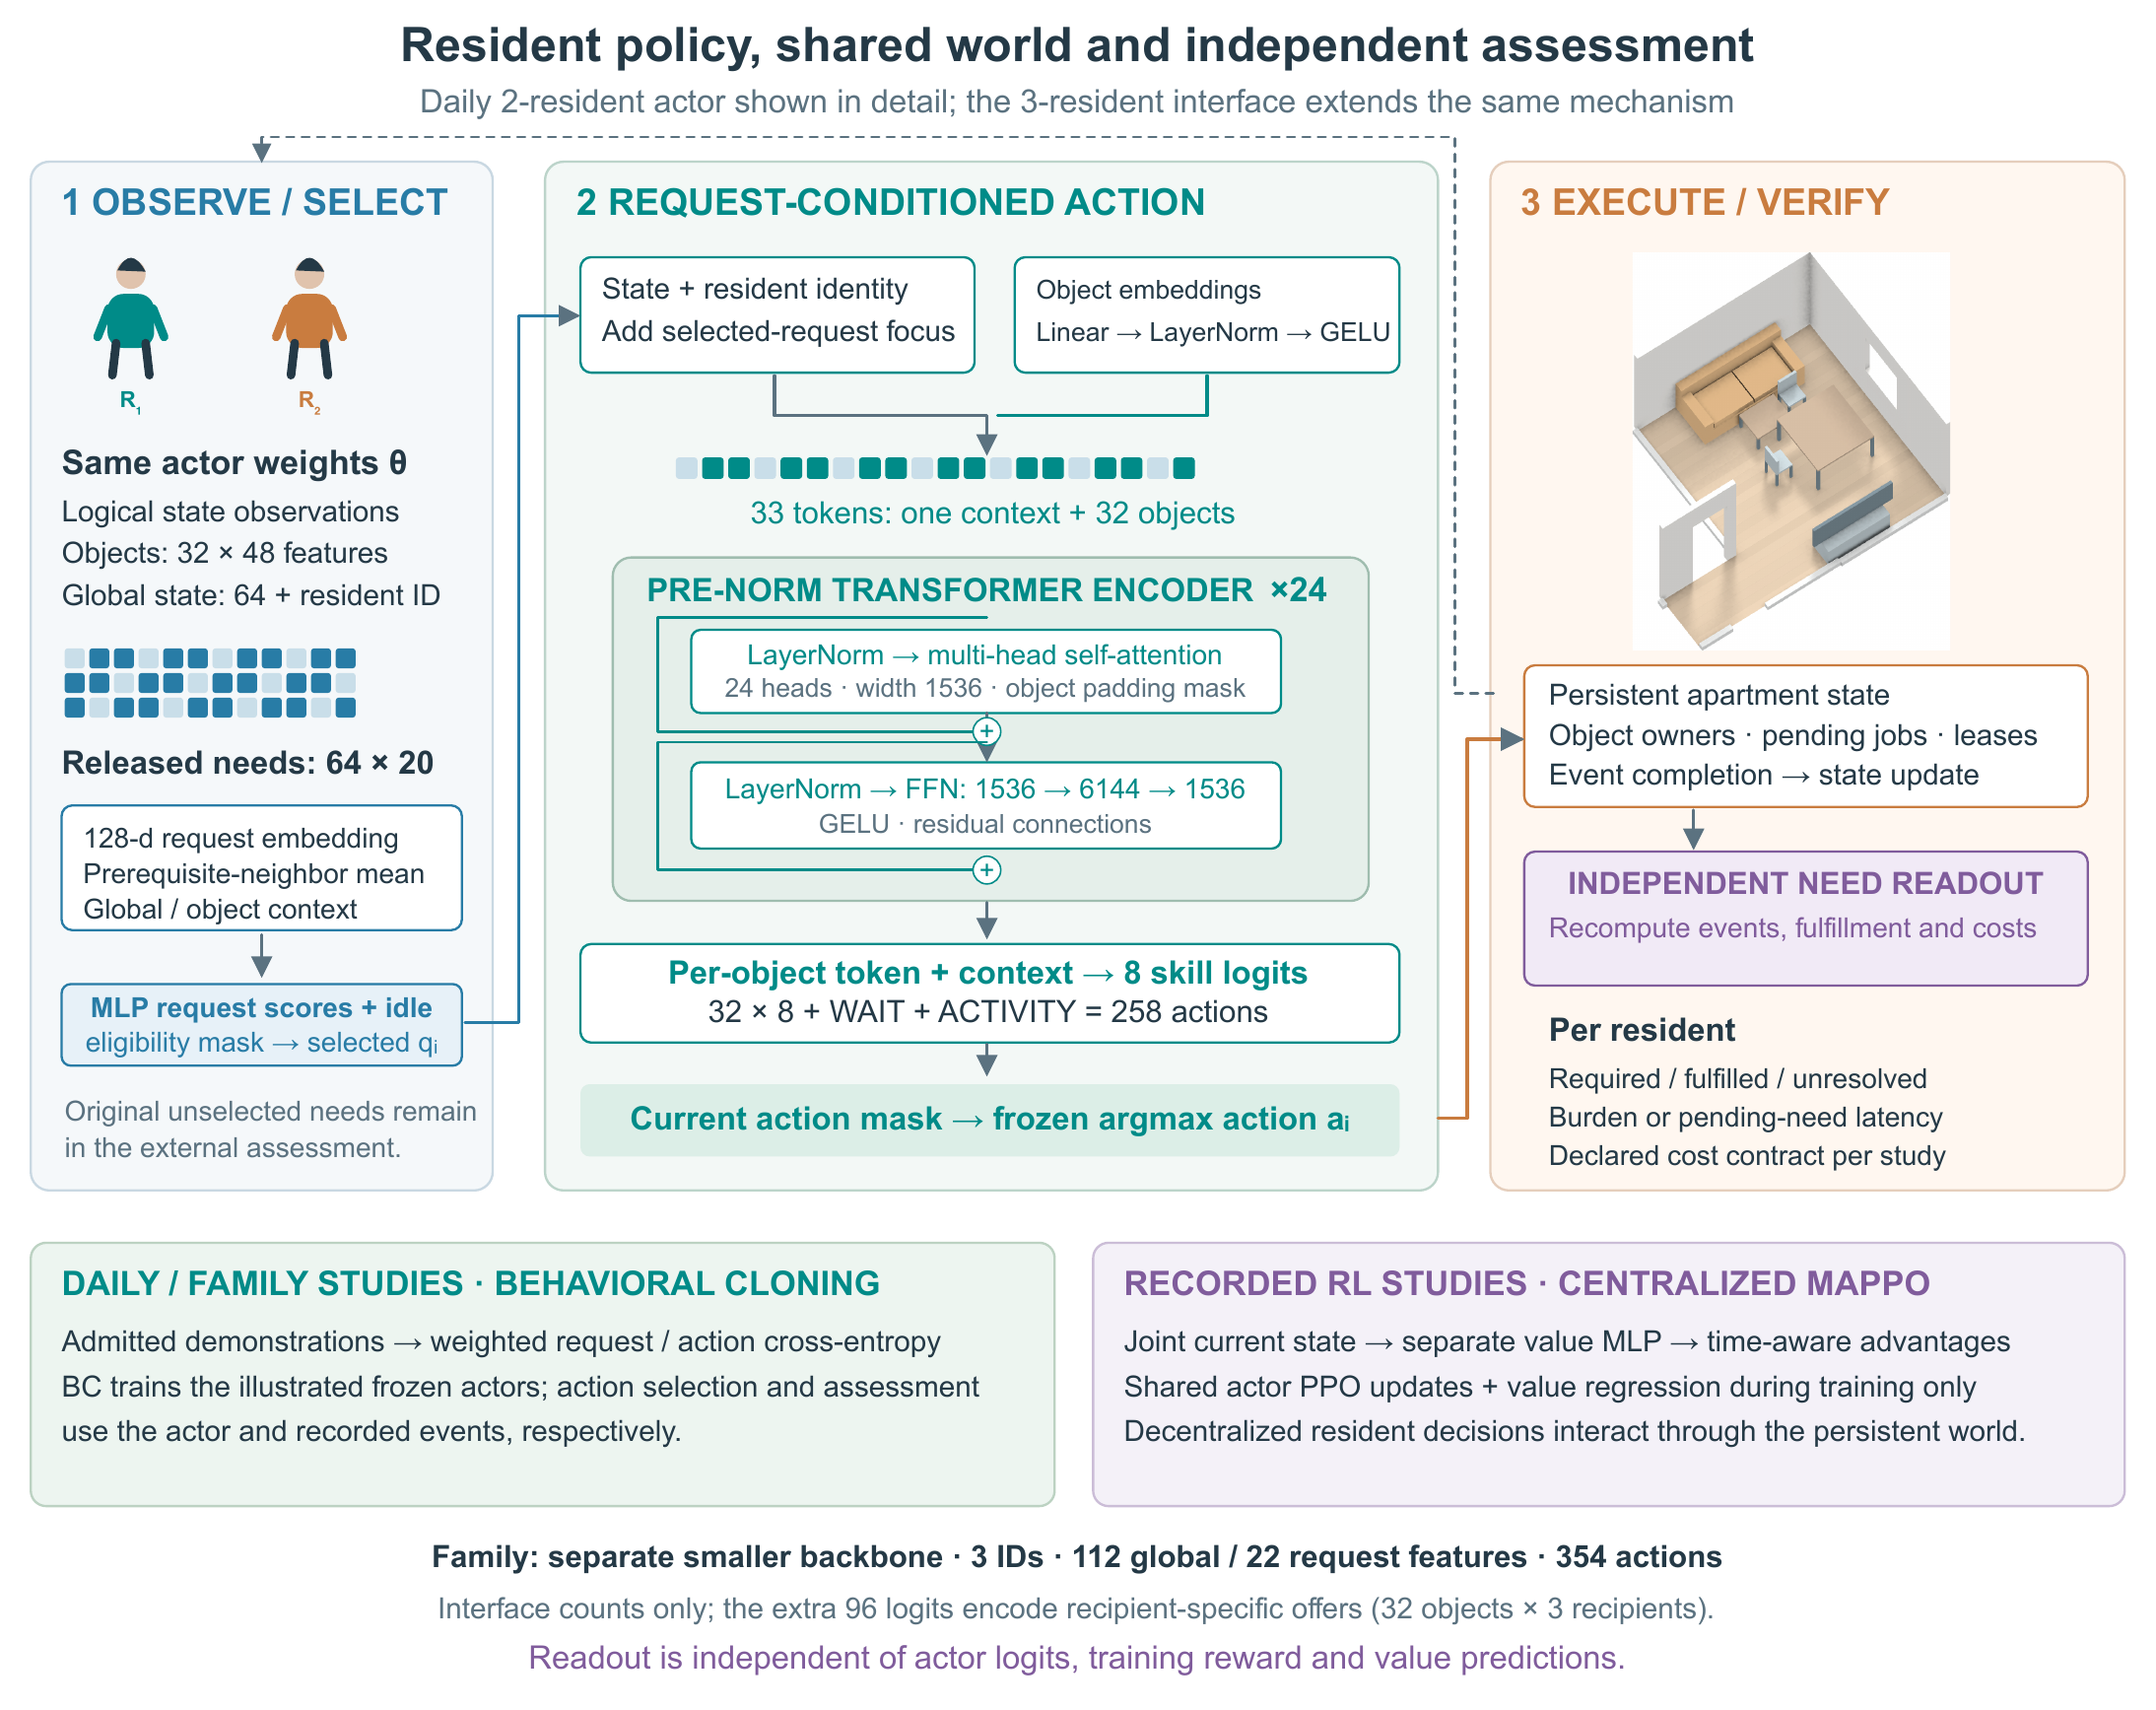}
\caption{\textbf{Learned resident computation and shared-world semantics.} The two-resident daily architecture is shown from its pinned implementation. Request selection uses embedded released needs, prerequisite-neighbor aggregation and current context; the selected request conditions the shared pre-norm Transformer. Object-wise action logits are masked before fixed decoding. The three-resident model has a separate smaller backbone and extends the interface with recipient-specific transfer choices. The lower panels distinguish the BC actors used in the daily/family studies from the separately recorded MAPPO training protocol. Independent household readout uses executed events and the declared assessment functional.}
\label{fig:architecture-detailed}
\end{figure*}

\subsection{Learning objectives and implemented architecture}
\label{app:architecture-learning}
For recorded MAPPO studies, residents share an actor while a separate centralized value critic conditions on the joint state. With importance ratio $r_{n,i}(\theta)$ and a critic-derived advantage $\widehat A_{n,i}$, the actor uses the clipped PPO objective
\begin{equation}
\begin{aligned}
\mathcal L_{\rm clip}(\theta)=\mathbb E_{n,i}\big[\min\big(&r_{n,i}(\theta)\widehat A_{n,i},\\
&\operatorname{clip}(r_{n,i}(\theta),1-\epsilon,1+\epsilon)\widehat A_{n,i}\big)\big].
\end{aligned}
\end{equation}
The implementation's time-aware discounts and current-state value estimates account for variable-duration events. The actor and critic learn during training; fixed resident policies generate evaluation trajectories. Centralized value information supports learning from interacting decisions in a common state~\cite{yu2022mappo,ppo2017}.

The successful daily and family comparison actors instead optimize masked request/action cross-entropy on constructive demonstrations:
\begin{equation}
\begin{aligned}
\mathcal L_{\rm BC}= -\mathbb E_{(o,q^*,a^*)}\!\big[&w_q\log\pi_\theta^{\rm req}(q^*\mid o)\\
&+w_a\log\widetilde\pi_\theta^{\rm act}(a^*\mid o,q^*)\big].
\end{aligned}
\end{equation}
BC updates the actor; its saved critic remains fixed and external assessment uses executed events. The MAPPO and BC cohorts therefore retain separate checkpoint and action-interface identities.

GRPO's group comprises sampled candidate completions used to form a reward-relative training baseline~\cite{shao2024deepseekmath}. MAPPO's residents instead interact through state transitions, leases, ownership and timing. This choice matches centralized training to the recorded interacting-resident RL setting; the BC cohorts provide an alternative learned executor. SceneTeract combines semantic planning and geometric feasibility verification and additionally uses GRPO for feasibility prediction~\cite{maillard2026sceneteract}. TEAM-GRPO groups complete joint-household trajectory replicas for relative-return estimation, defining a different estimator over the same interacting-agent setting. Each declared executor is assessed through the same household-use functional $\mathcal Q$; outcomes retain their executor identity.
