# Supplementary material for: CoHABIT: Complementary Evaluation of Furniture Layouts through Spatial Rules and Household Routines
Source: arXiv:2611.29494 source file (2026-11-22)
Supplement: Supplementary file 7 [file c_dynamic.tex]

\section{Resident Model and Event Semantics}
\label{app:dynamic_model}\label{app:learned_execution}\label{app:operational_model}\label{app:learning_details}
\subsection{Persistent state and actions}
The shared state contains time, positions, object anchors/owners, open states, pending jobs, leases, released requests and credited needs. Ready residents select requests and actions; scheduled completions update the persistent world. The actor observes logical state. Variable-duration commitments follow the semi-Markov view of temporal abstraction~\cite{sutton1999options}, with durations determined by modeled actions.

The daily interface has 258 actions: 32 object-indexed choices for NAV, OPEN, CLOSE, PICK, PLACE, USE, OFFER and ACCEPT, plus WAIT and sustained ACTIVITY. State-dependent masks restrict policy support~\cite{mask2022} through affordances and immediate eligibility. NAV uses profile-specific graphs; PICK/PLACE update ownership/support; sustained activities advance requests. Capacity-one resources use leases. Eligible actions can still loop without completing needs.

For resident $i$, the frozen policy factorizes as
\begin{equation}
\pi_\theta(q_i,a_i\mid o_i)=\pi_\theta^{\rm req}(q_i\mid o_i)\,
\widetilde\pi_\theta^{\rm act}(a_i\mid o_i,q_i).
\end{equation}
Both furnishings use identical weights and argmax decoding. Requests and actions are learned; temporal controllers remain separate. Unselected original needs remain in the evaluator.

\input{supplement_sections/c_architecture_learning}

\subsection{Matched execution and independent readout}
\label{app:criterion-algorithms}
Algorithm~2 states the execution/readout boundary. A fixed decoder acts on matched original needs; replay reconstructs actual outcomes before costs are compared. Unfinished obligations remain visible.

\begin{table*}[t]\centering\small
\begin{tabularx}{\textwidth}{@{}rY@{}}\toprule
\multicolumn{2}{@{}l}{\textbf{Algorithm 2. Matched household execution and independent readout}}\\\midrule
\textbf{Input}&Layouts $(\mathcal{L}_A,\mathcal{L}_B)$; household $H$, original needs $\xi$, frozen actor $\pi_\theta$ and execution contract.\\
\textbf{Output}&Verified need records, personal burdens, interactions and supported pairwise comparison.\\\midrule
1&Validate matched needs, profiles, schedules, decoding and semantics; retain identical physical starts for furnishing edits and admitted starts for cross-home comparisons.\\
2&\textbf{for each} layout $\mathcal{L}\in\{\mathcal{L}_A,\mathcal{L}_B\}$ \textbf{do}\\
3&\quad Initialize persistent state $x_0$ and retain every original need in the evaluator.\\
4&\quad \textbf{while} events or original needs remain, within the declared horizon and action budget \textbf{do}\\
5&\qquad For each ready resident $i$, select $q_i=\operatorname{Decode}(\pi^{\mathrm{req}}_\theta)$ and $a_i=\operatorname{Decode}(\widetilde\pi^{\mathrm{act}}_\theta(\cdot\mid q_i))$ with fixed decoding.\\
6&\qquad Schedule admissible actions; commit the earliest completion and update shared resources, ownership and time.\\
7&\quad Independently replay the resulting events and reconstruct each resident's original-need outcomes and costs.\\
8&\textbf{if} both alternatives fulfill the complete matched need set, compare their household and personal burdens.\\
9&\textbf{else} retain incomplete, certified-adverse and unresolved outcomes without interpreting early abandonment as low cost.\\
10&\textbf{return} matched outcomes and evidence using the external assessment functional.\\\bottomrule
\end{tabularx}
\end{table*}

\input{supplement_sections/c_mappo_update}

\subsection{Behavioral cloning and competence}
For the BC objective defined above, constructive demonstrations supply the training targets. The whole-home actor descends from the rich-assessment BC checkpoint through daily balanced and event-uniform BC stages. Earlier MAPPO cohorts remain separate experiments (Table~\ref{tab:learning-cohorts}).

Daily actors clone admitted constructive demonstrations using weighted masked request/action cross-entropies. Uniform and skill-balanced variants change row/action weights. The kitchen comparison freezes three separately trained actors after six passes: uniform seeds 4101/4102 and balanced seed 4103.

Actions alter subsequent observations, making closed-loop performance dependent on the policy-induced state distribution~\cite{ross2011dagger}. Normalization placement also affects Transformer optimization~\cite{xiong2020layernorm}. We assess competence through executed original needs and recomputed burden. Appendix~F separates fixed-weight request/action interventions from weight-changing adaptation and its retention check.

\paragraph{Policy learning and external assessment.}
PPO optimizes a clipped surrogate~\cite{ppo2017}; GAE trades bias against variance in advantage estimation~\cite{gae2016}. Independent PPO uses local value estimates~\cite{ippo2020}; COMA assigns credit through counterfactual baselines~\cite{foerster2018coma}; QMIX factorizes team values monotonically~\cite{rashid2018qmix}. These optimize return; our resident burdens are external measurements. The MAPPO/GRPO distinction is detailed in Section~\ref{app:architecture-learning}.

\subsection{Clock, waiting and original needs}
The engine processes the earliest pending completion, rounding positive sub-microsecond activity residuals upward to one microsecond. This corrects a legacy defect that could prolong a five-second activity until an unrelated request. Main-paper daily comparisons use the corrected clock; independent replay checks actions and times. Historical Appendix~F diagnostics retain their protocols.

Primary burden includes instrumental actions, invalid-attempt time and forced waiting; desired eating, rest and work are excluded. Voluntary waiting enters a separate sensitivity comparison. Unfinished released needs stay in the denominator; matched costs require all original needs to complete.

\paragraph{Reproducibility.}
Section~\ref{app:policy_choice} specifies the matched comparison contract; Algorithm~2 defines replay and readout. Scene, execution, need and action counts retain separate denominators; research records preserve run histories.
