# Supplementary material for: CoHABIT: Complementary Evaluation of Furniture Layouts through Spatial Rules and Household Routines
Source: arXiv:2611.29494 source file (2026-11-22)
Supplement: Supplementary file 8 [file c_mappo_update.tex]

\subsection{Centralized training for the recorded MAPPO branch}
Algorithm~3 makes the recorded native MAPPO update explicit. Ready residents contribute separate action rows but share an event-level advantage from the current joint-state critic. The time-aware recursion uses $\gamma_n=\gamma^{\Delta t_n/u}$ and $\lambda_n=\lambda^{\Delta t_n/u}$, where $u$ is the declared time unit. This is the finite-TRAIN-epoch branch studied below; the request-conditioned daily/family BC branch retains its separate cross-entropy objective.
\begin{table*}[t]\centering\small
\begin{tabularx}{\textwidth}{@{}rY@{}}\toprule
\multicolumn{2}{@{}l}{\textbf{Algorithm 3. Event-based MAPPO with a current joint-state critic}}\\\midrule
\textbf{Input}&Shared actor $\pi_\theta$, centralized critic $V_\phi$, admitted training cases, rollout length, PPO budget, time unit $u$.\\
\textbf{Output}&Updated actor and critic; checkpoint preserving optimizer, collector and random state.\\\midrule
1&Initialize training worlds and a frozen actor anchor $\pi_{\rm ref}$; retain their original exogenous cases.\\
2&\textbf{while} admitted training cases remain \textbf{do}\\
3&\quad Collect a rollout: for each event, record the current joint state $s_n$ and $V_\phi(s_n)$ before acting.\\
4&\quad Each ready resident samples a masked action; record its old log probability and execute the joint dispatch.\\
5&\quad Record reward, elapsed time $\Delta t_n$, terminal flag and final next-state value before any reset.\\
6&\quad Compute backwards $\delta_n=r_n+\gamma_n(1-d_n)V_{n+1}-V_n$ and $A_n=\delta_n+\gamma_n\lambda_n(1-e_n)A_{n+1}$.\\
7&\quad Map event advantages to resident rows and normalize once over the rollout to obtain $\widehat A_{n,i}$ for the actor.\\
8&\quad For each PPO epoch and minibatch, minimize the negative clipped surrogate, minus entropy, plus the configured $\mathrm{KL}(\pi_\theta\Vert\pi_{\rm ref})$ anchor.\\
9&\quad Separately update $V_\phi$ by mean squared error to $A_n+V_n$ using the original, unnormalized $A_n$ over valid world events.\\
10&\quad Preserve the distinct actor/critic optimizer states and the exact continuing world and scheduler state.\\
11&\textbf{return} the trained checkpoint; evaluate household needs with the separate executed-event readout.\\\bottomrule
\end{tabularx}
\end{table*}
Here $d_n$ marks an actual terminal and $e_n$ an episode boundary: continuing cuts retain their bootstrap, while resets end the bootstrap chain. Entropy and anchor terms regularize training; the external functional measures furnishing quality.
