# Supplementary material for: CoHABIT: Complementary Evaluation of Furniture Layouts through Spatial Rules and Household Routines
Source: arXiv:2611.29494 source file (2026-11-22)
Supplement: Supplementary file 9 [file d_paired_quality.tex]

\section{Matched Evaluation and Interpretation}
\label{app:resident_suitability}\label{app:human_protocol}\label{app:ablation_matrix}\label{app:complementarity_proof}
\subsection{Frozen pairing and scoring}
\label{app:policy_choice}\label{app:quality_interpretation}\label{app:dynamic_understanding}
Same-home furnishing comparisons fix the envelope, inventory and physical starts while changing the declared furniture placement or orientation. Cross-home comparisons instead match household, semantic needs and calendar through admitted task bindings and starts in each home. Both fix policy weights, decoding and cost rules. We report completion, unresolved coverage and operational burden separately. Repeated request realizations are grouped within their source family. We report source-family counts and repeated draws separately for uncertainty-aware interpretation of few-run RL estimates~\cite{agarwal2021}.

\subsection{Original needs and observed burdens}
For scored intervals $I_{im}$, resident $i$'s path $\ell_i$ sums committed NAV distances. Active time is skill occupancy intersected with those intervals; waiting follows the declared idle/WAIT/BLOCKED accounting. A shared handoff is one committed event but occupies both participants. Pre-request idle time is excluded where the scoring interval starts at request release. Missed semantic demands and missed primitive predicates retain different denominators.

Every unmet demand is classified as independently verified unmet or unresolved. Cost attribution uses the declared reference or proof assumptions. A certificate based on a fixed navigation graph is scoped to that graph. Cause-specific resource waiting is represented separately from total observed waiting. We report forced and voluntary waiting separately and test the sensitivity of furnishing order to including both.

\subsection{Measured household contrasts}
\label{app:household-main-protocol}
The contrasts below use the pairing contract in Section~\ref{app:policy_choice}, with fixed event semantics. Request randomness and policy-action randomness have separate roles.

\paragraph{Interaction cost.}
For unchanged personal needs, the additive joint-versus-solo contrast is
\begin{equation}
I(\mathcal{L},H)=C_\Sigma^{\mathrm{joint}}(\mathcal{L},H)-C_A^{\mathrm{solo}}(\mathcal{L},p_A)-C_B^{\mathrm{solo}}(\mathcal{L},p_B).
\end{equation}
Joint-only tasks are excluded from this estimand. The reference experiment crosses shared/private logical resources with request offsets, mobility profiles and furnishing variants. The private-resource control yields zero interaction, while shared resources give positive cost for synchronous requests. This control identifies the contribution of resource coupling. Helping uses a separate matched intervention with unchanged personal obligations.

\paragraph{Profile-dependent furnishing order.}
For furnishings $\mathcal{L}_A,\mathcal{L}_B$, define $\Delta_H=C_\Sigma(\mathcal{L}_A,H)-C_\Sigma(\mathcal{L}_B,H)$. A reversal has opposite signs under two household profiles and requires complete original-need fulfillment in every compared condition. The measured mobility intervention changes resident B's capability parameters while preserving request contents. The house-00685 contrast is reported separately for the initial request draw and three additional timing realizations.

\paragraph{Synchronization and temporal controls.}
Holding request contents fixed, we measure
\begin{equation}
\delta=\Delta_H^{\mathrm{sync}}-\Delta_H^{\mathrm{offset}}.
\end{equation}
The reported comparisons use a 180-second request offset, profile-weighted routes, request-priority search and finite start-delay search. The temporal controls have full information about the modeled day. Their different waiting components explain why removing forced waiting can lower primary burden while increasing voluntary delay. Algorithms are compared under the same original needs, with completion coverage reported beside cost.

\subsection{Open questions for household-conditioned assessment}
\label{app:open-questions}
\textbf{Executor sensitivity.} Which furnishing orders remain stable across independently competent executors? Matched needs and completion support comparisons of scheduling and personal costs under a common external functional.

\textbf{Routine coverage.} Which additional needs make an otherwise unused furnishing change observable? A coverage map from household activities to affected objects and routes can guide finite, interpretable scenario selection.

\textbf{Household calibration.} How should numerical capabilities and the declared preference rubric be calibrated for a target household? Separating physical parameters from preference weights allows each source of evidence to be assessed directly.

\textbf{Physical co-presence.} How do continuous body motion, mutual passage and access envelopes change conclusions based on logical resource sharing? This extends the shared-state formulation from timed ownership and cooperation to simultaneous use of physical space.

\subsection{Source-family construction}
All 12,000 original source identities are accounted for: 11,994 adapted houses and six unadapted entries. The input-capability audit checks adapted payload hashes and excludes declared geometry/source/contour families crossing official splits, as well as unsupported metadata. Eight development families are selected from the original validation split by an immutable hash ordering, requiring at least two reusable tableware nodes and a nonportable dining table. Five pass the subsequent geometry, common-start and task-binding checks used in the reported household experiment. These rules define its restricted task population.
