# Supplementary material for: CoHABIT: Complementary Evaluation of Furniture Layouts through Spatial Rules and Household Routines
Source: arXiv:2611.29494 source file (2026-11-22)
Supplement: Supplementary file 10 [file e_data.tex]

\section{Datasets, Splits and Exclusions}
\label{app:construction_audit}\label{app:whole_apartment_semantics}
\subsection{Rich furnishing cohort}
\label{app:rich_full_audit}
The rich source/geometry/alias review admits 7,704 parent houses from the original official training split. Parent and alias partitions were frozen before outcomes: 6,224 training, 701 development and 779 locked test. Two households and six recipes per parent give 92,448 fixed conditions: 74,688/8,412/9,348 by partition. The original official validation and test houses remain reserved. Collection and independent source/replay/semantic/cost checks reconcile the fixed evaluation population; dwelling outcomes are reported separately.
\begin{table}[t]\centering\small
\caption{Rich training reference verdicts, retaining every fixed condition and unknown.}
\begin{tabular}{@{}lrrr@{}}\toprule
Branch&Positive&Negative&Unknown\\\midrule
Static 0&41,244&21,782&11,662\\
Dynamic&228&5,261&69,199\\
Combined&228&27,043&47,417\\\bottomrule
\end{tabular}\end{table}
The training set contains 5,583 observed episode payloads: 228 positive, 5,261 negative and 94 unknown. Their original input/target, competence, cost and leakage checks pass; 1,834,795 actor rows are eligible constructive demonstrations. Observed behavior categories are 728 competent-full, 3,798 best-attainable partial and 1,057 non-demonstration episodes. Imitation targets include demonstrated actions only.

The full training-set semantic denominator is 8,445,192: 347,086 met, 199,465 verified unmet and 7,898,641 unknown. Observed episodes contain 563,199 semantic demands; all remaining conditions retain their recorded evaluation status. Across all partitions, 6,953 constructor/restore records and 6,949 indexed episode payloads are distinct from successful weeks. 

Strict matching uses source house, household, original requirements/physical-start context, criteria, world seed, scenario and source version. Dynamic yields 21 positive--negative pairs in 13 contexts/ten houses, versus 363 Combined pairs in 145 contexts/118 houses, among 186,720 possible within-context training pairs. The larger Combined count may follow Static 0. These metadata describe the reference cohort; neural discrimination is evaluated through actor executions.
