# Supplementary material for: CoHABIT: Complementary Evaluation of Furniture Layouts through Spatial Rules and Household Routines
Source: arXiv:2611.29494 source file (2026-11-22)
Supplement: Supplementary file 11 [file f_bc_progression.tex]

\paragraph{Historical checkpoint progression.}
Figure~\ref{fig:training-competence} organizes the existing daily-pilot and expansion evaluations by training progress. These historical checkpoints are separate from the current family actors.

\begin{figure*}[t]\centering
\includegraphics[width=.94\textwidth]{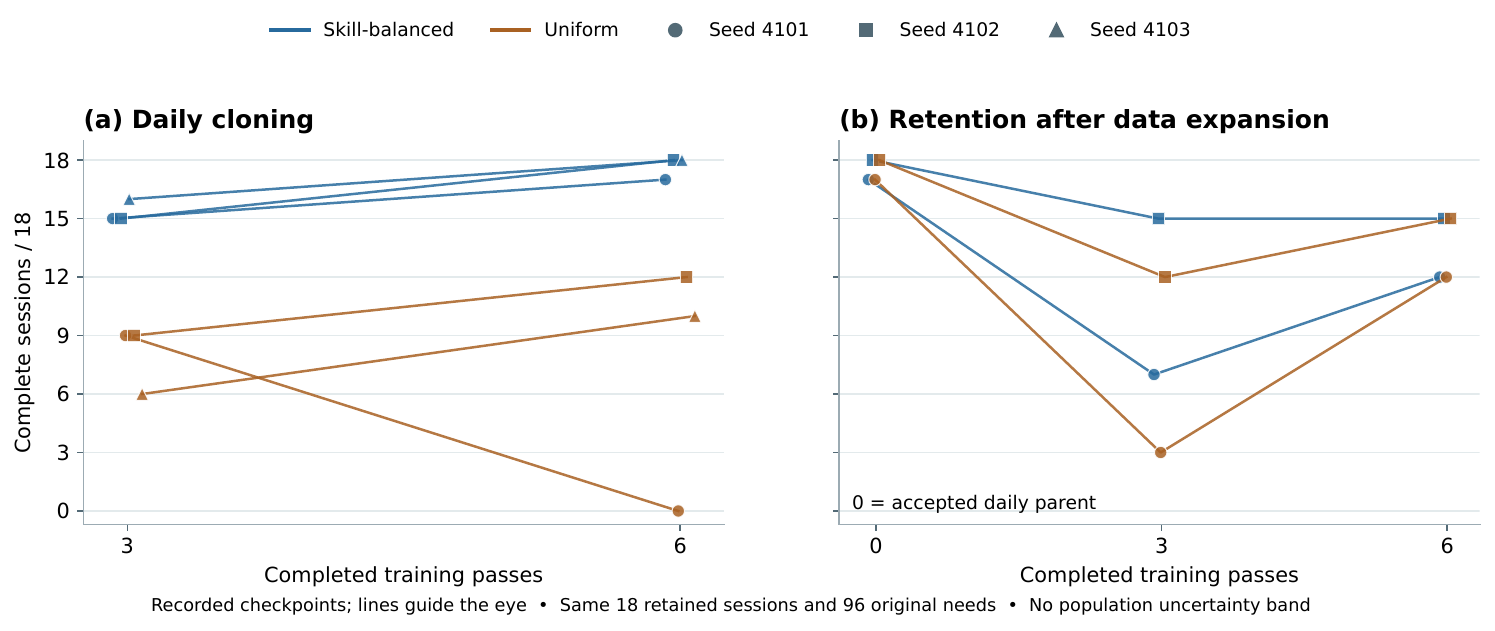}
\caption{\textbf{Demonstration fitting and retained execution are distinct measurements.} (a) Completed daily sessions at the two evaluated cloning checkpoints, for all three paired seeds. (b) Retained completion after the demonstration set expands, for the two shared-parent seed pairs. Each observation evaluates the same 18 sessions and 96 original needs under its declared historical execution contract. Zero in (b) denotes the accepted daily parent. Lines connect the measured checkpoints. Seeds replicate fine-tuning on the same exposed scenes. No population confidence interval is implied.}
\label{fig:training-competence}
\end{figure*}
