# Supplementary material for: CoHABIT: Complementary Evaluation of Furniture Layouts through Spatial Rules and Household Routines
Source: arXiv:2611.29494 source file (2026-11-22)
Supplement: Supplementary file 12 [file f_complex_trajectories.tex]

\subsection{Multi-room routines and joint execution}
\label{app:complex_trajectories}
The following saved executions show how repeated activities use a furnished home over time. The first example follows one resident across several rooms; the next two distinguish simultaneous personal routines from an actual transfer between residents. Each example retains its original agenda and model, so their goal counts and distances are read within the corresponding scenario.

\begin{figure*}[t]\centering
\includegraphics[width=.86\textwidth]{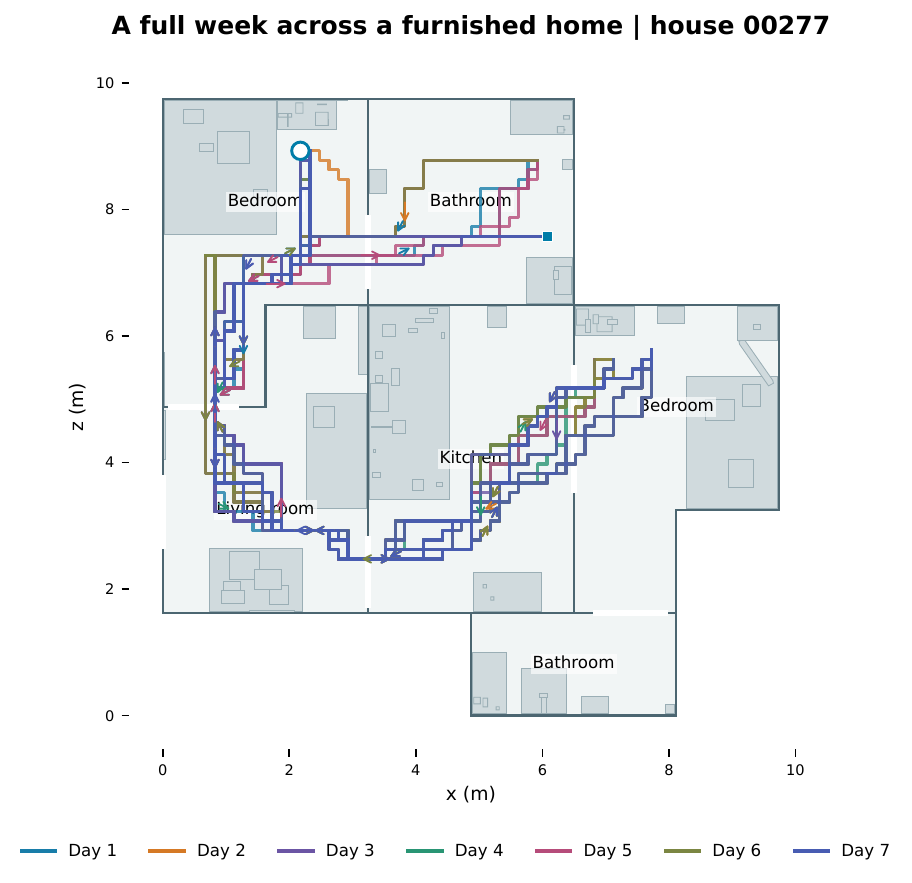}
\caption{\textbf{A full week of routes through a furnished home.} The saved PPO execution in house 00277 completes 21 stages and all 90 original goal conditions. Its 109 NAV actions cover 42 distinct directed endpoint pairs and total 1033.35\,m; recorded stops occupy five of six rooms. Colors denote the seven days, arrows give travel direction, and the circle and square mark the initial and final positions. Repeated routes overlap at their true coordinates. This single-resident example illustrates spatial coverage and repetition of the prescribed routine.}
\label{fig:complex-week-trajectory}
\end{figure*}

All routes are reconstructed from saved committed actions using the declared profile-specific free-space graph. Original floor and furniture geometry, door openings, endpoints, per-action distances and total distance are checked. The polylines represent admissible static NAV paths. These historical illustrative executions are separate from the daily-policy experiments in the main paper.

\begin{figure*}[t]\centering
\includegraphics[width=\textwidth]{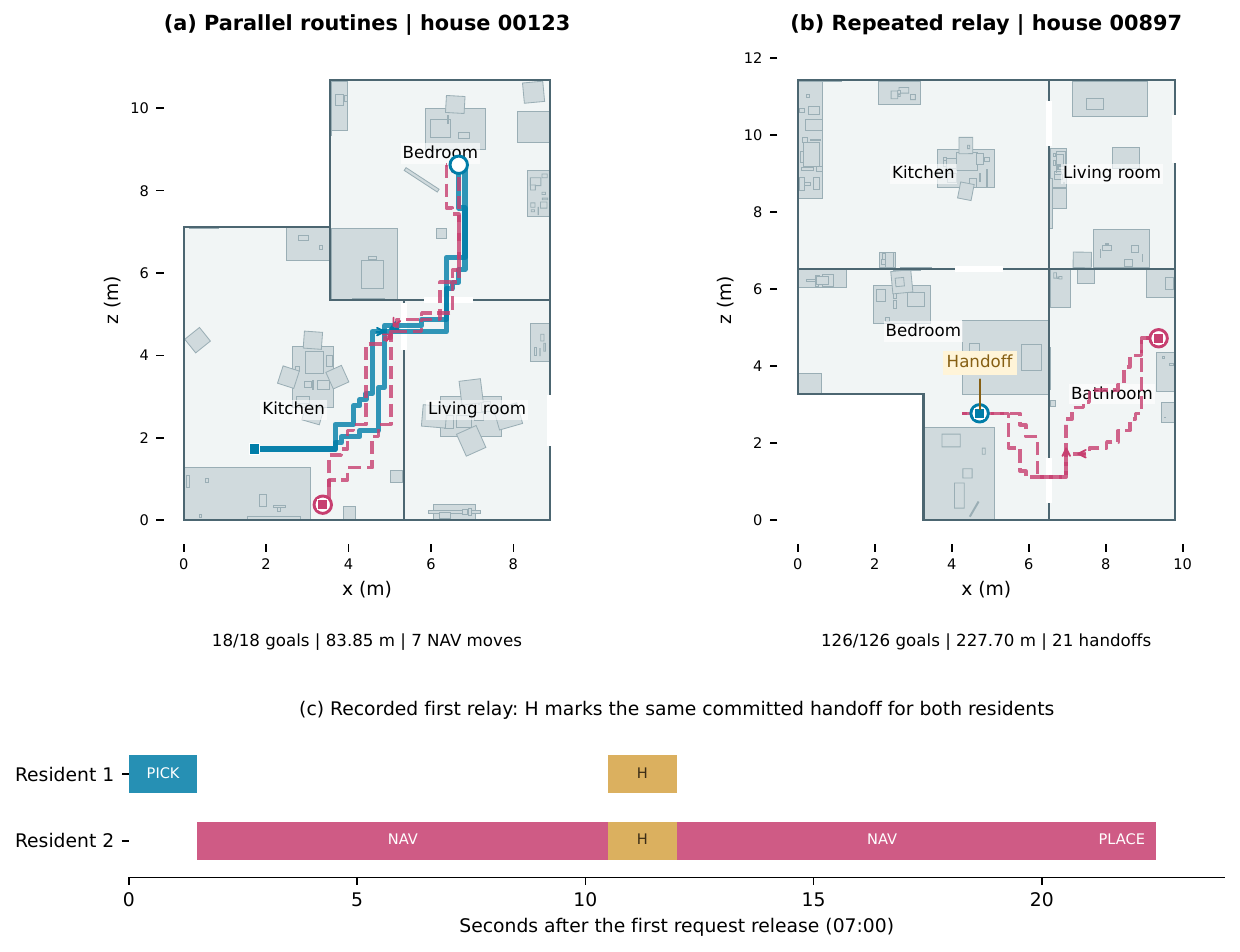}
\caption{\textbf{Two residents: concurrent routes and a repeated object relay.} Blue denotes resident 1 and dashed pink resident 2; circles and squares show starts and finishes. (a) In house 00123, both residents move between activity locations while completing all 18 goal conditions of the one-day agenda. Seven NAV actions total 83.85\,m. This is parallel execution, with no handoff. (b) In house 00897, the seven-day relay completes 126/126 goal conditions and records 21 successful handoffs. Resident 1 remains at the transfer location while resident 2 makes 22 journeys, totaling 227.70\,m. Repeated traversals share their plotted paths. (c) The first relay, directly from committed event times: resident 1 picks up the item; resident 2 navigates to the partner; both participate in the same 1.5-second handoff; resident 2 then travels to the destination and places the item. The full chain finishes 22.5 seconds after release. Gold bars mark a single shared event.}
\label{fig:joint-trajectory-examples}
\end{figure*}

The two panels use the same historical MAPPO checkpoint but different homes and agendas. They illustrate verified behavior under their recorded execution conditions. In particular, the stationary partner in the relay participates in every transfer: a resident can contribute to joint completion without accumulating a long route. The model attributes physical access to declared geometry and contention to logical-resource events; route plots show the spatial component.
