# Supplementary material for: CoHABIT: Complementary Evaluation of Furniture Layouts through Spatial Rules and Household Routines
Source: arXiv:2611.29494 source file (2026-11-22)
Supplement: Supplementary file 13 [file f_evidence.tex]

\section{Additional Household Results and Examples}
\label{app:behavioral_cloning}\label{app:policy_diagnostics}\label{app:frozen-temporal}
\subsection{Shared-resource and temporal controls}
The corrected-clock reference experiment contains $5\times2\times2\times8\times3\times2=960$ executions: families, furnishings, mobility profiles, request offsets, joint/solo occupancy and shared/private resources. Every execution fulfills its original needs. Independent replay verifies the committed decisions and recomputes the readout. The private-resource control namespaces non-actor leases by resident, preserving personal requests, starts and geometry.
\begin{figure*}[t]\centering
\includegraphics[width=.94\textwidth]{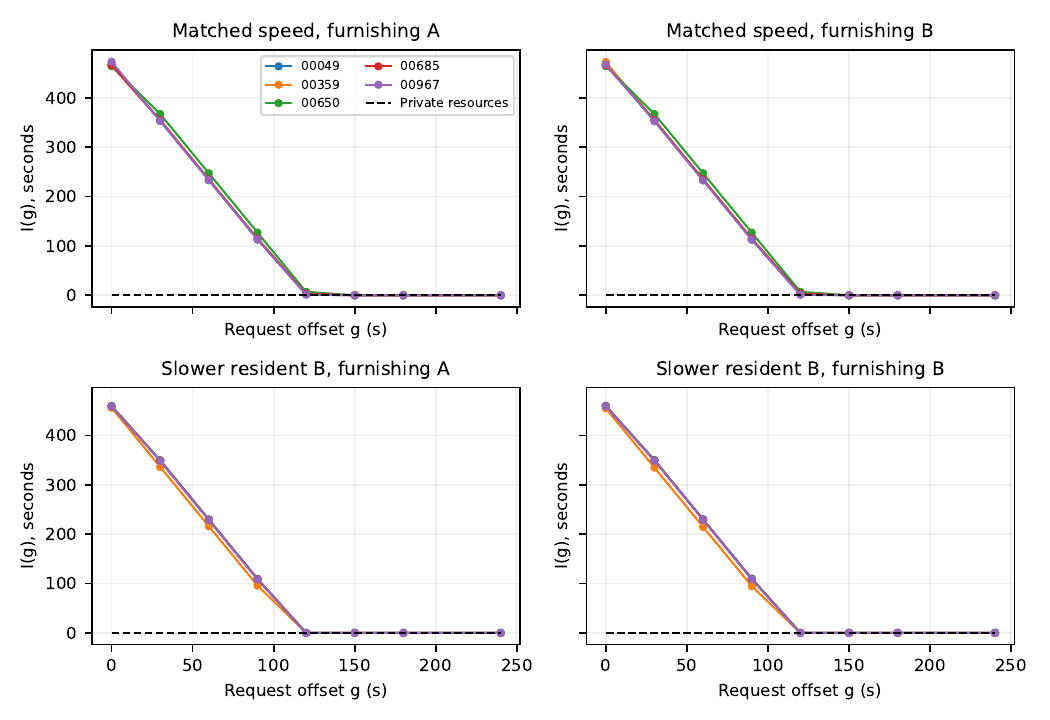}
\caption{Interaction cost $I(g)$ across every admitted family, furnishing and mobility profile. Private resources give zero interaction. Shared resources produce cost at overlapping request times, which disappears as requests separate. Curves are individual development observations.}
\label{fig:interaction-gap}\end{figure*}

\begin{figure}[t]\centering
\includegraphics[viewport=0 0 252 165,clip,width=\linewidth]{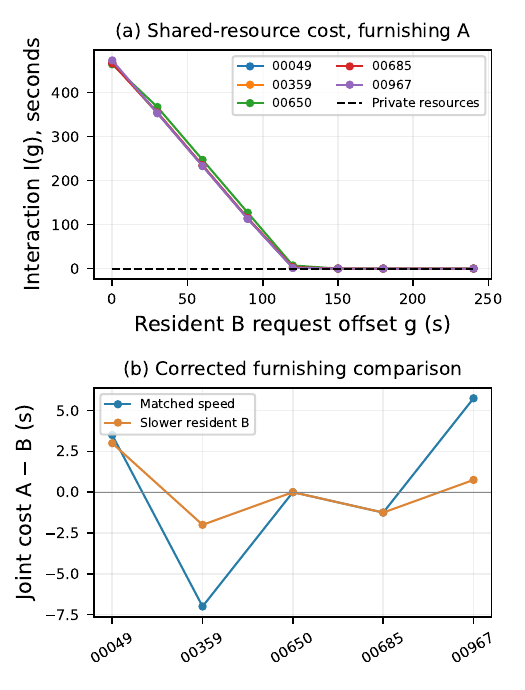}
\caption{\textbf{Furnishing-order control on the same reference cohort.} Synchronous A--B costs under matched speed and slower resident B reuse the corrected-clock executions in Figure~\ref{fig:interaction-gap}. Positive A--B favors B.}
\label{fig:h23-reference}\end{figure}

The priority controller enumerates six prerequisite-compatible orders per resident. A separate delay controller evaluates fixed offsets of 0,30,60,90,120,150,180 and 240 seconds, with 15 joint and eight solo candidate schedules per condition. Candidate selection prioritizes complete needs, then burden, with microsecond-precision and deterministic ties. These finite controllers know the modeled day in advance.

\begin{table}[t]\centering\small\setlength{\tabcolsep}{3pt}
\caption{Frozen comparison eligibility. Each method has 120 executions and 640 original needs. An interaction requires complete joint and both solo executions.}
\label{tab:frozen-eligibility}
\begin{tabular}{@{}lrrr@{}}\toprule
Method & Complete & Needs met & $I$ eligible\\\midrule
Uniform 4101 & 88/120 & 484/640 & 24/40\\
Uniform 4102 & 56/120 & 360/640 & 8/40\\
Balanced 4103 & 32/120 & 256/640 & \textbf{0/40}\\
Priority search & \textbf{120/120} & \textbf{640/640} & \textbf{40/40}\\
Delay search & \textbf{120/120} & \textbf{640/640} & \textbf{40/40}\\\bottomrule
\end{tabular}\end{table}
Balanced cloning has zero eligible interaction comparisons, so its contrast is recorded as unavailable. This comparison measures the combined change of seed and weighting.

\begin{figure*}[t]\centering
\includegraphics[width=.94\textwidth]{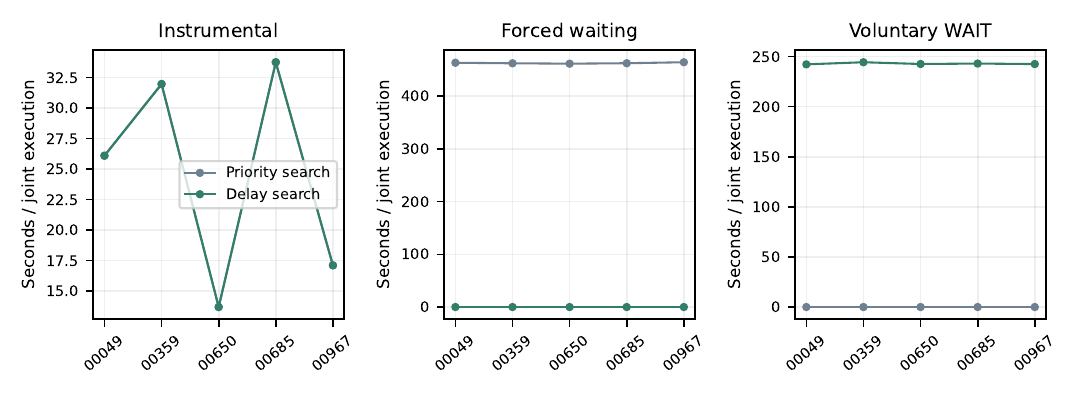}
\caption{Why schedule selection changes burden. Each point averages four synchronous joint furnishing/profile conditions in one family. Voluntary waiting is shown separately from instrumental cost and witnessed forced waiting.}
\end{figure*}
On the twenty synchronous joint conditions, mean instrumental time is 24.52\,s for both temporal controls. Priority search adds 463.00\,s of forced waiting; delay search instead adds 242.85\,s of voluntary waiting and zero forced waiting. Thus primary burden is 487.53 versus 24.52\,s, while including voluntary waiting gives 267.37\,s for delay search. This identifies the role of scheduling and the selected cost definition.

An initial-input route proxy sums start-to-item, item-to-serving-surface and surface-to-seat graph distances, divides by resident speed, and adds the configured three seconds per resident for PICK and PLACE. Across all forty joint inputs it matches delay-search primary cost to within $4.3\times10^{-14}$\,s. After forced waiting is removed, the primary cost of this kitchen task family is explained by routes and fixed manipulation costs.

\subsection{Assistance and waiting attribution}
The matched intervention preserves A's work and B's delivery/consumption needs, permitting either A or B to deliver B's object. Reactive execution reverses A/B order in four of five families. Finite scheduling removes those primary-cost reversals. When voluntary waiting is included in both schedule selection and the readout, families 00359 and 00967 retain reversals, with no-help/help contrasts $+3.00/-11.00$ and $-8.25/+0.75$\,s. All sixty executions and 120 needs per control are verified.
\begin{figure*}[t]\centering
\includegraphics[width=.94\textwidth]{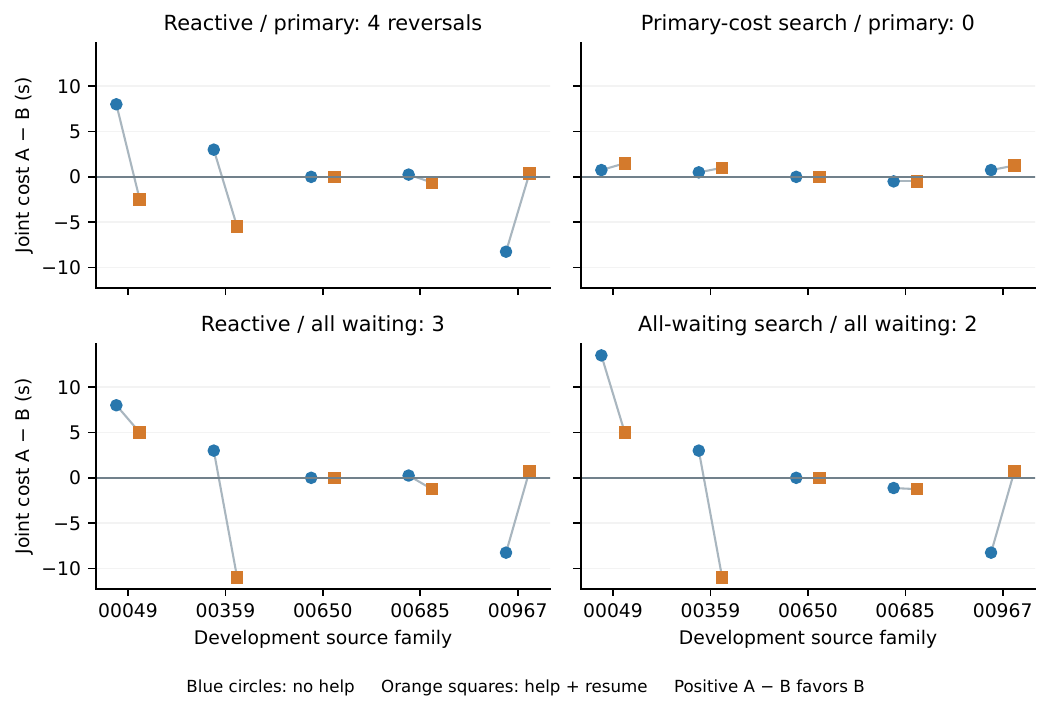}
\caption{Assistance-conditioned furnishing order under different controllers and waiting definitions. The waiting-inclusive controller is selected using the same quantity that is reported. Desired activity is excluded throughout. Points are individual development-family observations.}
\label{fig:help-wait-sensitivity}\end{figure*}
\begin{table}[t]\centering\small
\caption{Mean joint-time components over ten furnishings per row. $C$ includes instrumental and forced-wait time; $V$ is voluntary waiting. All original needs are fulfilled. Components are rounded independently.}
\label{tab:help-wait-components}
\begin{tabular}{@{}llrrr@{}}\toprule
Controller & Help & $C$ & $V$ & $C+V$\\\midrule
Reactive & Off &261.92&0.00&261.92\\
Reactive & On &252.70&9.47&262.17\\
Min. $C$ & Off &13.70&313.86&327.56\\
Min. $C$ & On &14.28&601.97&616.24\\
Min. $C+V$ & Off &118.61&133.63&252.24\\
Min. $C+V$ & On &252.70&9.47&262.17\\\bottomrule
\end{tabular}\end{table}
The apparent primary-cost benefit can exchange forced waiting for longer voluntary delay. This explains why the ranking changes with the accounting rule. A separate frequency intervention doubles B's kitchen episodes; both controllers fulfill all 800 original needs across 120 conditions, with unchanged instrumental costs. The object remains on its serving surface after the first delivery, and subsequent desired consumption is excluded from burden, explaining this null frequency effect.

\subsection{Profile contrast across request-time draws}
Uniform actor 4101 is frozen after its selection by development completion. Three additional request-time draws retain all five families, both furnishings and mobility profiles, and both offsets, giving forty joint conditions and 320 needs per draw. Each draw yields 32/40 complete executions and 260/320 fulfilled needs. Delay search completes all 120 conditions and 960 needs across the three draws.
\begin{figure*}[t]\centering
\includegraphics[width=.94\textwidth]{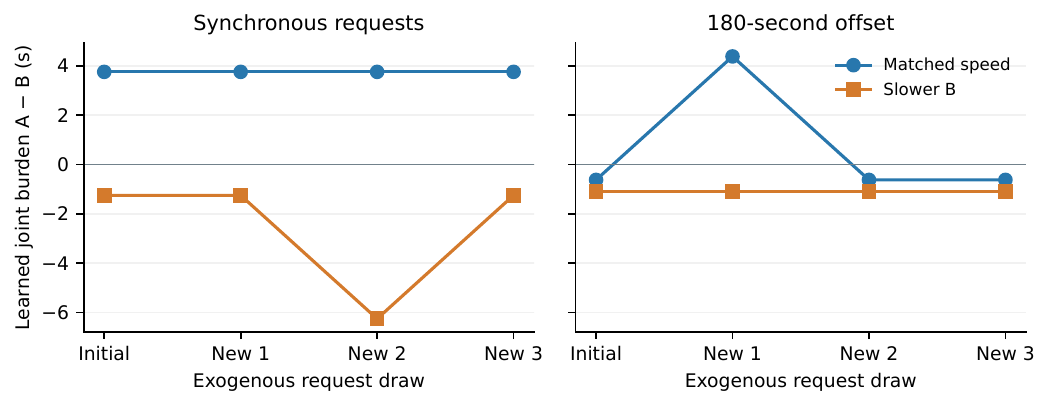}
\caption{The same frozen actor in house 00685 under the original and three additional request-time draws. Positive A--B favors B. The synchronous profile-conditioned reversal repeats; the asynchronous contrast varies. Lines connect individual realizations.}
\label{fig:learned-profile-replication}\end{figure*}
The synchronous A--B contrasts are $+3.75,+3.75,+3.75$\,s for matched speed and $-1.25,-6.25,-1.25$\,s for slower B. Every condition entering these contrasts fulfills its original needs. The synchronous reversal persists after subtracting recorded invalid-attempt time. This is a repeated local effect of the frozen behavior; the matched temporal controller retains the same furnishing order across profiles.

\subsection{Interpreting execution and retention effects}
On the same forty conditions, replacing request selection alone leaves completion at 32/40. Replacing primitive execution gives 36/40 and eliminates the action-limit cuts. Recorded failures include repeated valid NAV to the current node and persistent idle-request selection. The guards below test those two mechanisms with unchanged weights, needs, geometry and deadlines.
\begin{table}[t]\centering\small
\caption{Matched execution interventions. All rows retain forty conditions and 320 needs. Guards change inference rules; reference-action rows diagnose execution.}
\begin{tabular}{@{}lrr@{}}\toprule
Variant & Complete & Needs met\\\midrule
Original policy &32/40&260/320\\
Reference requests &32/40&260/320\\
Reference actions &36/40&304/320\\
Navigation guard &34/40&298/320\\
Request guard &32/40&260/320\\
Both guards &\textbf{37/40}&\textbf{310/320}\\
Reference actions + request guard &\textbf{40/40}&\textbf{320/320}\\\bottomrule
\end{tabular}\end{table}
Both guards improve completion to 37/40, while reference actions with the request guard complete all forty conditions. The former is a measured execution improvement under changed inference; suppressing idle requests also changes willingness to act, so competence and behavioral interpretation remain separate.

\label{sec:revision-audit}\label{sec:short-repair-pilot}
A separate one-epoch BC adaptation of uniform actor 4101 reduces learning rate and increases PICK/PLACE weight over the same 8,450 admitted rows (34 updates). On the eighteen matched retention conditions, completion falls from 18/18 to 15/18 and fulfilled needs from 96/96 to 84/96; valid PICK and PLACE commits each fall from 27 to 24. The adapted actor completes 43/48 expanded conditions and 248/256 needs. Independent replay verifies all eighty-four executions. This is an adverse retention effect on matched inputs; learning rate and weighting changed together, so neither is identified as its sole cause. The expanded set measures a separate population; the matched retention result records the regression.


\subsection{Family calendars and comparison coverage}
Two adults and a child execute three whole-home scenarios under six numerical profiles, two request draws and synchronous or shifted calendars. Each actor has 144 executions with 3,024 original needs. Two initial actors complete 120 and 108 executions and each admits 54 of 72 matched comparison contexts. Both complete all synchronous cases; incomplete shifted traces concentrate on assistance coordination. In the matched-update comparison, synchronous-only controls complete 108 and 114 executions, whereas both diverse-calendar actors complete all 144 and all needs, expanding context coverage from 54 to 72. Demonstration diversity and size change together. In every diverse-calendar comparison, all three individual costs favor B. In the birthday example in the main paper, B reduces adult/child latency by approximately 76, 58 and 79 need-seconds.

\paragraph{Independent units in the main family table.}
Development uses two homes (00650 and 00967); unfitted transfer uses two additional TRAIN-pool homes (06417 and 08887). Each calendar contains $2\times3\times6\times2=72$ executions across homes, routines, profiles and request draws. The last column counts $1\times3\times6\times2\times2=72$ contexts of one fixed home-pair across two calendars. Parenthesized repetitions use paired training seeds 7201 and 7202; the request draws are 74501 and 74502. These are controlled comparisons on fixed homes. We report exact completion counts for each seed on 72 repeated contexts of the same apartment pair. With two homes, a house-cluster bootstrap has at most three distinct resampled means and collapses for all-complete cells; uncertainty on new homes requires additional source geometries.

\input{supplement_sections/f_learning_cohorts}
\input{supplement_sections/f_retained_results}

\input{supplement_sections/f_execution_readiness}

\input{supplement_sections/f_whole_home}
\input{supplement_sections/f_complex_trajectories}
\input{supplement_sections/f_trajectory_examples}
\input{supplement_sections/f_reference_examples}
\subsection{An additional controlled furnishing intervention}
\label{app:expanded_paired_comparison}\label{app:competence_census}
The retained house-01869 example uses the earlier fixed-agenda policy and 105 original demands per furnishing. Its side-table group moves rigidly by 0.60\,m. The source-bound panels below distinguish achieved, independently certified-unmet and unresolved needs; efficiency comparisons require complete execution.
\begin{figure*}[t]\centering
\includegraphics[width=\textwidth]{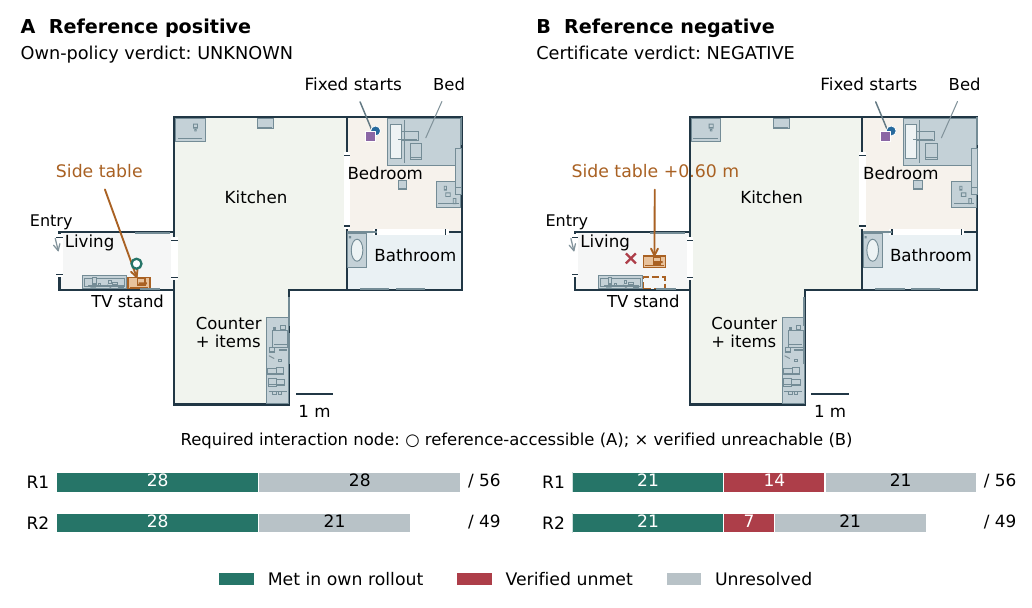}
\caption{\textbf{Actual furnishing intervention within the controlled matrix.} House 01869 keeps the same residents, starts and 105 demands; B moves a side table and its supported items $+0.60$\,m in the floor plane. MAPPO meets 56/105 versus 42/105 demands. Bars retain certified-unmet and unresolved needs. A remains unknown; B is negative only through a scoped model certificate. This selected training example illustrates a reference-conditioned contrast.}
\label{fig:frozen-pair}
\end{figure*}
