# Supplementary material for: CoHABIT: Complementary Evaluation of Furniture Layouts through Spatial Rules and Household Routines
Source: arXiv:2611.29494 source file (2026-11-22)
Supplement: Supplementary file 14 [file f_execution_readiness.tex]

\subsection{Admissibility and routine composition}
\label{app:execution-readiness}
Six development cases hold actor 4101's weights, geometry, households and original needs fixed across interfaces. The cohort spans two homes and one calendar. Interfaces developed on this cohort constrain current-state choices without teacher replacement, defining distinct executed policies.

\begin{table}[tb]\centering\small
\caption{\textbf{Matched admissibility interventions.} Six cases and 106 original needs per row; all executions independently replayed, without weight updates.}
\label{tab:whole-home-readiness}
\begin{tabular}{@{}lrr@{}}\toprule
Decision interface & Complete & Needs met\\\midrule
Original affordances &0/6&8/106\\
Activity readiness &0/6&33/106\\
Suppress idle request &0/6&11/106\\
Activity + idle control &0/6&33/106\\
Physical readiness &\textbf{2/6}&\textbf{71/106}\\\bottomrule
\end{tabular}\end{table}
Idle is suppressed only with an eligible need. Physical readiness adds manipulation preconditions to activity readiness, preserving navigation, transfer, waiting and request selection. It completes the illustrated home's independent-day and shared-evening joint routines; the paired home reaches the kitchen stage but leaves later needs unmet. Both contrasts remain horizon-censored policy outcomes, separating local admissibility from complete-routine assessment.

\begin{figure}[tb]\centering
\includegraphics[width=\linewidth]{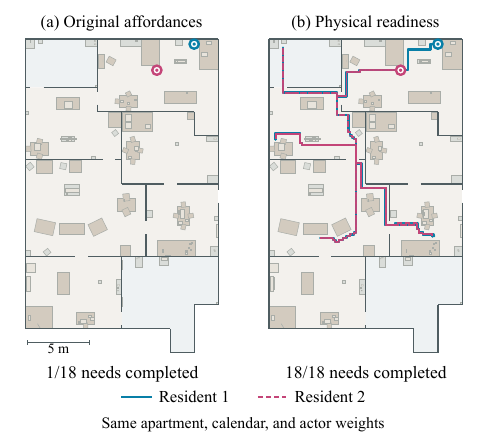}
\caption{\textbf{Admissibility exposes joint execution.} The shared-evening example uses fixed actor weights and original needs. Physical readiness completes the joint routine, including a shared meal and conversation. Curves reconstruct verified committed navigation; rings mark coincident start/end positions.}
\label{fig:whole-home-readiness}
\end{figure}
