# Supplementary material for: CoHABIT: Complementary Evaluation of Furniture Layouts through Spatial Rules and Household Routines
Source: arXiv:2611.29494 source file (2026-11-22)
Supplement: Supplementary file 15 [file f_learning_cohorts.tex]

\subsection{Learning branches and recorded training progress}
\label{app:learning-cohorts}
Table~\ref{tab:learning-cohorts} resolves training identity before interpreting an executor's results. MAPPO was trained and evaluated in three earlier branches; the daily and family furnishing comparisons use BC-trained actors. The accepted checkpoint and training record identify each actor's algorithm.

\begin{table*}[t]\centering\small
\caption{Learning provenance of the reported resident cohorts. Source hashes and logs accompany the materials. Checkpoint identity includes interface, data and evaluation contract as well as seed.}
\label{tab:learning-cohorts}
\begin{tabularx}{\textwidth}{@{}p{.19\textwidth}p{.19\textwidth}p{.21\textwidth}Y@{}}\toprule
Cohort & Training & Checkpoint or trace & Evidence supported\\\midrule
Fixed agendas & MAPPO & Seed 103, update 406 & One-day parallel routine (18/18 goals); seven-day relay (126/126, 21 handoffs). Verified trajectory examples under fixed agendas.\\
Native finite-TRAIN & MAPPO & Seeds 302--304; 58,043 training cases per seed & Iteration-level training progress in the native training runtime.\\
Rich optimization & BC warm-up, then MAPPO & Seeds 201--205; privileged and route-hidden & Ten iteration traces describe optimization. The frozen comparison below uses its own fixed evaluation cohort.\\
Rich frozen comparison & BC predecessor versus MAPPO & Route-hidden seed 201, before/after RL & Matched need coverage and tie-adjusted ordering on 21 selected pairs, 32 TRAIN conditions and ten houses.\\
Daily and whole-home & Behavioral cloning & Daily seeds 4101--4103; whole-home 6101, update 512 & Corrected-clock household comparisons; whole-apartment and shared-50-pair executions use the declared fixed interface.\\
Family volume-changing & Offline behavioral cloning & Seeds 7201--7202; single/diverse, update 2,048 & Four actors; 28,506 versus 81,462 demonstration examples. Main-paper calendar comparison and initial transfer.\\
Family matched-volume & Offline behavioral cloning & Seeds 7201--7204; synchronous/diverse, update 2,048 & Eight paired-calendar actors; fixed 27,158 examples per condition; temporal and geometric transfer tests retain their own splits.\\\bottomrule
\end{tabularx}
\end{table*}

\paragraph{Iteration-level MAPPO observations.}
Figures~\ref{fig:training-rich-mappo} and~\ref{fig:training-native-mappo} retain the separate five-seed rich-assessment and three-seed native cohorts. Each plotted value comes from an actual logged update, with minibatch metrics aggregated within that update. Recorded endpoints differ across runs. These curves expose optimization and training progress; verified original-need outcomes below provide the behavioral evidence.

\begin{figure*}[t]\centering
\includegraphics[width=.94\textwidth]{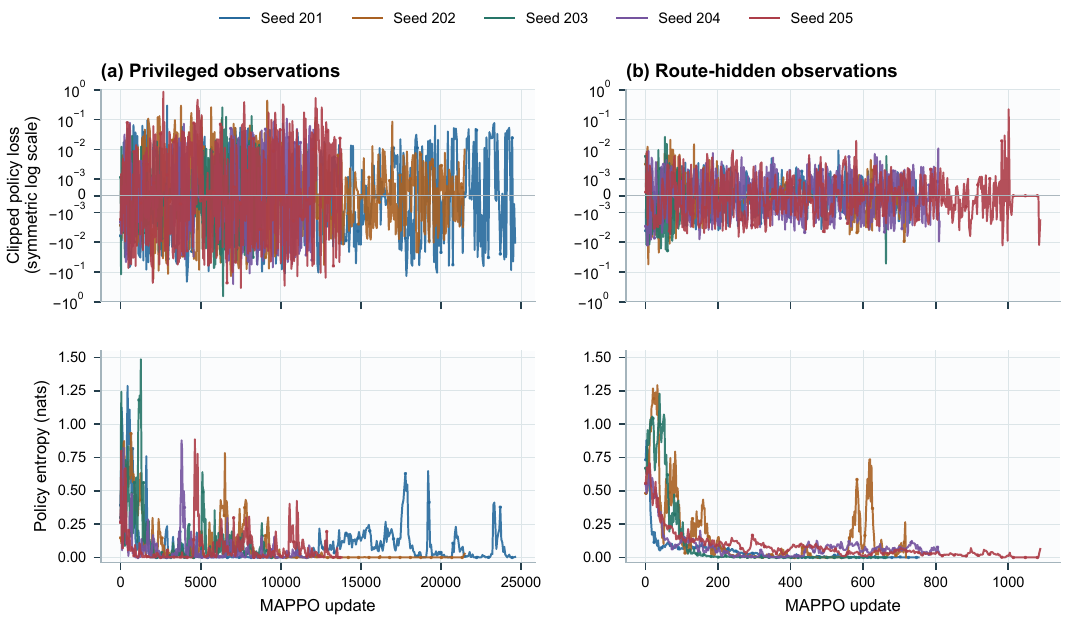}
\caption{\textbf{Recorded MAPPO optimization across five initializations.} Privileged and route-hidden observations are shown separately, with actual update coordinates and per-update minibatch means. Curves stop at the corresponding recorded endpoints. Policy loss uses a symmetric logarithmic scale; entropy uses a linear scale. Both statistics describe policy optimization; held-out execution measures household competence.}
\label{fig:training-rich-mappo}
\end{figure*}

\begin{figure*}[t]\centering
\includegraphics[width=.94\textwidth]{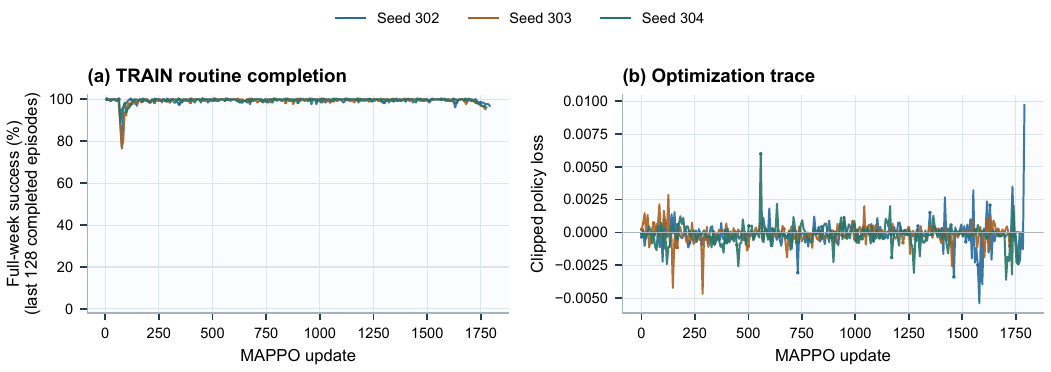}
\caption{\textbf{Native-runtime MAPPO iterations for seeds 302--304.} This cohort is separate from the rich-assessment branch above. Left: recorded success in the latest 128 completed TRAIN episodes. Right: policy loss at actual logged updates. Rolling training windows measure progress on changing training cases.}
\label{fig:training-native-mappo}
\end{figure*}
