# Supplementary material for: CoHABIT: Complementary Evaluation of Furniture Layouts through Spatial Rules and Household Routines
Source: arXiv:2611.29494 source file (2026-11-22)
Supplement: Supplementary file 16 [file f_reference_examples.tex]

\subsection{Reference-execution examples across apartments and households}
\label{app:desktop_reference_gallery}
These four post-hoc illustrations reuse the archived reference trajectories from the earlier 24-condition CPU pilot: 16 modeled weeks, six positive, ten negative and eight unknown outcomes. Its visit agenda and 150/75\,m budgets differ from the rich 900\,m study. Original polygons, object identities, rigid edits, goals, physical starts and readouts are retained; no new NAV, simulated episode or neural call produced these figures. Bounding-box footprints and the fixed 2.5D graph define the spatial approximation used in these simulated activities.

Pilot static approval checks for added overlap; broader ergonomic criteria have their own assessment. G1/G2 are saved targets, S1/S2 are starts, and bars are one model metre. No continuous paths are reconstructed. Selected examples explain mechanisms under their recorded conditions.
\begin{figure*}[t]\centering
\includegraphics[width=.90\textwidth]{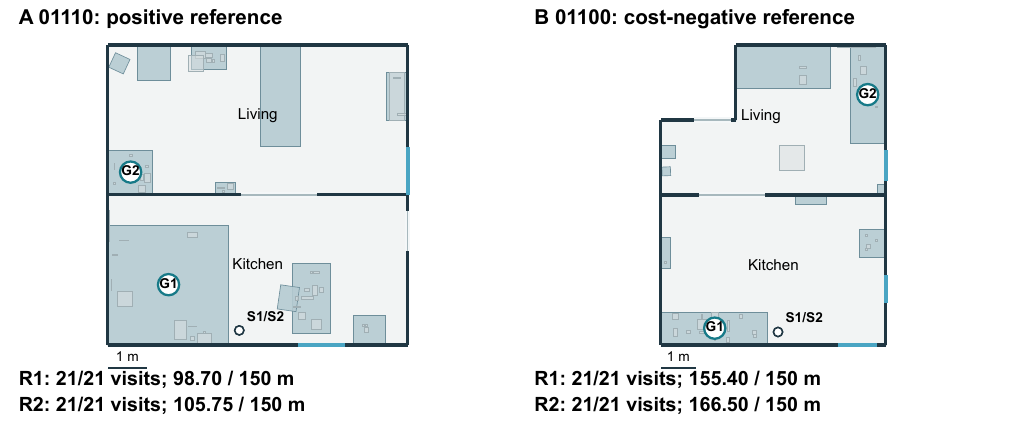}
\caption{\textbf{Different apartments, same declared household.} Both standard/fast residents meet 21/21 visit requirements. In 01110, paths 98.70/105.75\,m satisfy the 150/150\,m contract. In 01100, paths 155.40/166.50\,m exceed it, supporting a cost-negative operational assessment despite completion. Both pass the pilot's relative no-new-overlap condition. This comparison uses different apartments and a reference executor under the declared criteria.}
\label{fig:desktop_different_houses}
\end{figure*}


\begin{figure*}[t]\centering
\includegraphics[width=.90\textwidth]{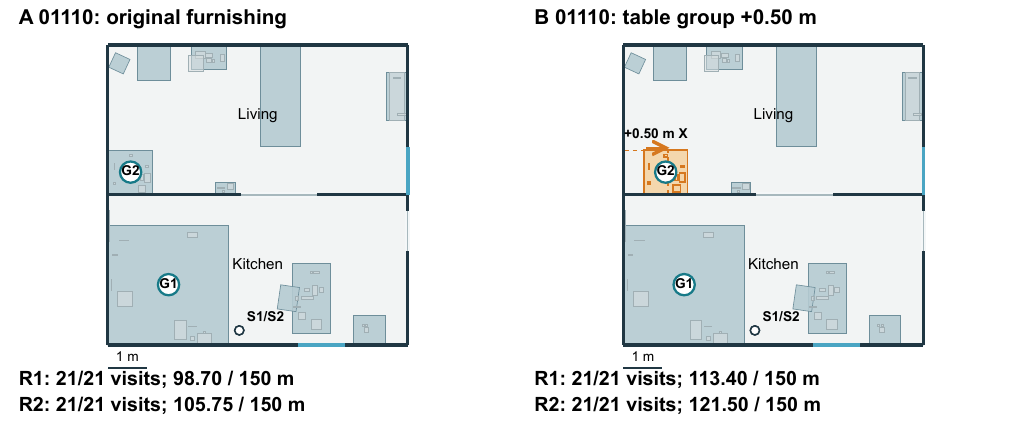}
\caption{\textbf{Actual matched furnishing pair without a verdict flip.} In 01110 the saved dining-table/support group shifts by 0.50\,m along the source $x$ axis; envelope, household and visit requirements remain fixed. Orange marks edited geometry; dashed outlines show its old position. Paths rise from 98.70/105.75 to 113.40/121.50\,m, while all 21/21 visit requirements per resident and both 150\,m limits are satisfied. Both outcomes remain positive under this contract; the translation changes travel costs without changing the contract verdict.}
\label{fig:desktop_furnishing_pair}
\end{figure*}


\begin{figure*}[t]\centering
\includegraphics[width=.90\textwidth]{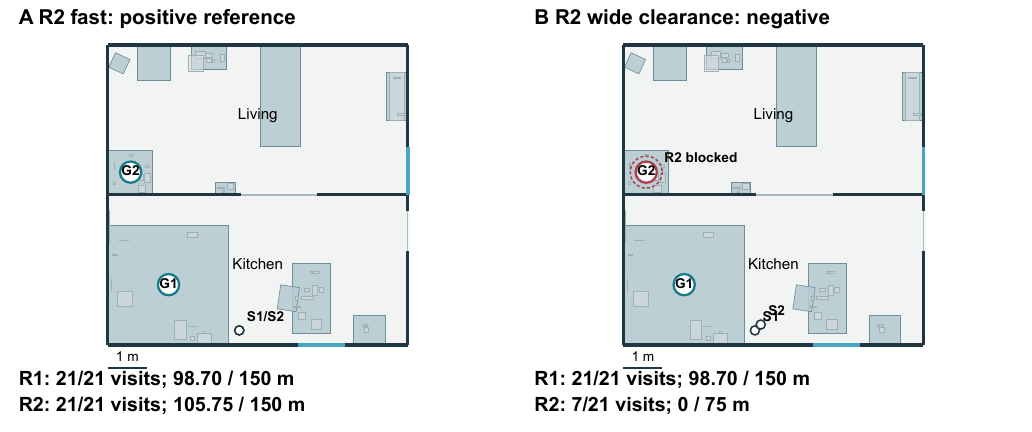}
\caption{\textbf{Same furnishing, different household contract.} R2 changes from fast to wide-clearance and its path limit changes from 150 to 75\,m. Under the saved fixed-graph access model, R2 meets 7/21 visits, with 14 verified unreachable visits at G2; R1 remains 21/21. R2 remains at its initial G1 node, completing the seven colocated visits with 0\,m travel; fourteen other required visits remain unreachable. The blocked-target annotation refers only to that stored graph certificate. Profile and budget change jointly under the fixed-graph access model; the resulting infeasibility verdict is scoped to that graph.}
\label{fig:desktop_household_change}
\end{figure*}


\begin{figure*}[t]\centering
\includegraphics[width=.90\textwidth]{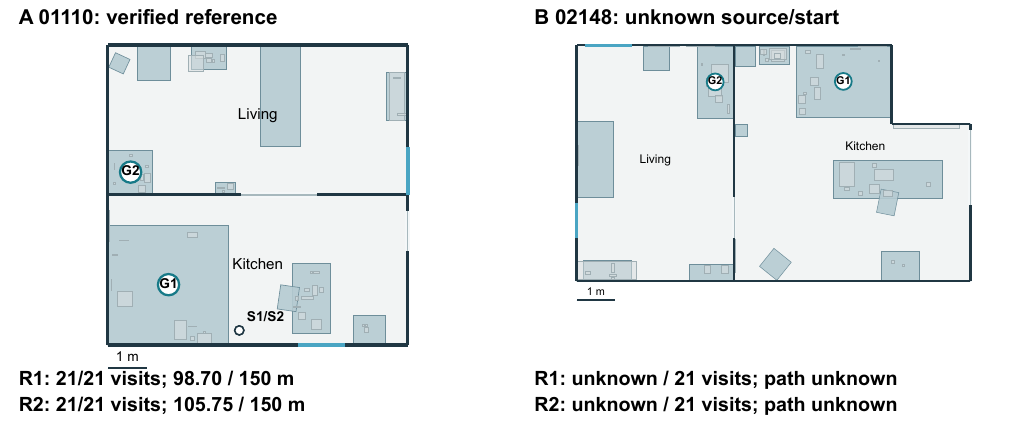}
\caption{\textbf{Unknown retains its denominator.} Source 01110 has verified reference readouts; 02148 lacks a preserved valid physical-start binding for the attempted condition. Its source plan is displayed with the attempted execution recorded as unresolved. All 21 required visits per resident remain in the denominator; completion and distance retain unknown values. The unresolved source condition retains an unknown furnishing verdict.}
\label{fig:desktop_unknown}
\end{figure*}
