# Supplementary material for: CoHABIT: Complementary Evaluation of Furniture Layouts through Spatial Rules and Household Routines
Source: arXiv:2611.29494 source file (2026-11-22)
Supplement: Supplementary file 17 [file f_retained_results.tex]

\subsection{Additional measured competence results}
\label{app:retained-diagnostics}
These historical studies separate execution competence from layout assessment. Rich actors use the earlier fixed-agenda, 257-action interface; the daily pilot predates the corrected-clock comparisons. Results are reported separately by execution contract.

\paragraph{Frozen comparisons and necessary bounds.}
Twenty-one reference-selected pairs reuse 32 training conditions in ten houses. Frozen BC, MAPPO and legal-mask control executions share exogenous draws and independent replay; learned decoding is FP32 masked argmax. Pair ordering gives half credit to ties:
\begin{center}\small\setlength{\tabcolsep}{4pt}
\begin{tabular}{@{}lrr@{}}\toprule
Policy & Met / required & Pair ordering\\\midrule
BC predecessor &90/2,884&.524\\
Subsequent MAPPO &\textbf{1,204/2,884}&\textbf{.762}\\
Legal-mask control &0/2,884&.500\\\bottomrule
\end{tabular}\end{center}
All methods have 0 positive, 11 certificate-negative and 21 unresolved verdicts: better demand ordering adds no verified classification gain.

Across 228 reference-feasible training conditions, two rich actors meet 9,910 and 4,299 of 21,112 demands, with no verified positive. Among 15 additional adverse cases, NAV+agenda bounds certify ten; stronger necessary checks certify eleven, without rejecting any feasible case. Both dynamic readouts inherit those eleven negatives. Necessary conditions explain the verified classification coverage; remaining cases are unknown.

\paragraph{From demonstrated actions to closed-loop skills.}
The corpus contains 285,090 manipulation targets among 1,834,795 eligible rows, yet final actors request only NAV/WAIT in 439 executions. On 2,736 familiar manipulation states, seed-201 demonstrated-action agreement falls from 2,317 after BC to 333 after adaptation; seed~205 yields eleven. A retention snapshot matches 403/456 PICK targets but commits no valid PICK in 228 executions, fulfilling 392/21,112 demands. BC navigation agreement was already weak: 5/226 picked-goal and 10/142 handoff-goal states. These contrasts compare checkpoints together with their recorded training protocols.

On eighteen short-chain cases with three action draws, BC completes 2/54 and final retention 0/54; neither completes handoff or parallel delivery. These probes evaluate exposed houses under the legacy clock; corrected-clock daily actors form a separate cohort. A modeled cross-room handoff completes in 22.5\,s with resident distances 0/20.70\,m, providing a verified event-sequence example.

\paragraph{Cloning gains are local and can regress after expansion.}
Checkpoint identity includes the training protocol as well as the seed: the pilot checkpoints below differ from the later corrected-clock kitchen actors carrying the same seed integers. The earlier daily pilot shares one parent and eighteen familiar-house sessions (96 needs) across three paired seeds. After six passes:
\begin{center}\small\setlength{\tabcolsep}{3pt}
\begin{tabular}{@{}lrr@{}}\toprule
Seed & Balanced: complete; met & Uniform: complete; met\\\midrule
4101 &17/18; 95/96&0/18; 38/96\\
4102 &\textbf{18/18; 96/96}&12/18; 81/96\\
4103 &\textbf{18/18; 96/96}&10/18; 72/96\\\bottomrule
\end{tabular}\end{center}
Fresh balanced initialization completes 9/18 sessions and 33/96 needs. Expanding to 48 demonstrations reduces retained completion from 17/18 and 18/18 to 12/18 and 15/18 after six passes under both weightings. Expanded coverage and matched retention are assessed separately. These outcomes measure local learning on the exposed routines. The later daily corpus contains 8,450 eligible NAV, PICK, PLACE, WAIT and ACTIVITY rows.

\input{supplement_sections/f_bc_progression}
