# Supplementary material for: CoHABIT: Complementary Evaluation of Furniture Layouts through Spatial Rules and Household Routines
Source: arXiv:2611.29494 source file (2026-11-22)
Supplement: Supplementary file 18 [file f_training_traces.tex]

\paragraph{Iteration-level family training observations.}
\label{app:training-observations}
Figure~\ref{fig:training-family-bc} shows the measured training loss for the eight matched-calendar family actors. Each condition has 27,158 admitted examples and a fixed budget of 2,048 accepted optimizer updates. The archive retains 39 unique minibatch observations across the eight runs: the first two accepted updates and available progress snapshots. The exact replay of update two is counted once. The final retained loss is at update 2,045; the accepted full checkpoint is at update 2,048. Only observed points are plotted, without smoothing, imputed updates or uncertainty bands. These losses measure demonstration fitting; independently audited routine execution establishes comparison competence.

\begin{figure*}[t]\centering
\includegraphics[width=\textwidth]{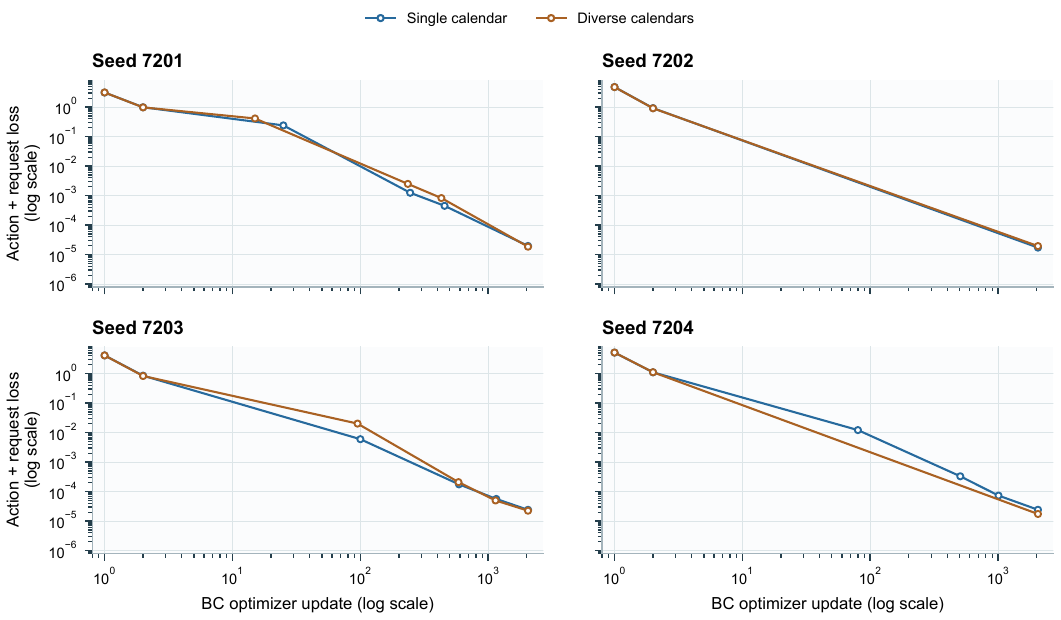}
\caption{\textbf{Iteration-level BC observations for four paired initializations.} Markers show all 39 retained optimizer-update observations under single and diverse calendars; connecting segments guide the eye without reconstructing missing iterations. Both conditions use the same training budget, with different observation densities. Both axes are logarithmic. The last retained loss is at update 2,045; accepted final states are at update 2,048. Independent execution establishes comparison competence.}
\label{fig:training-family-bc}
\end{figure*}
