# Supplementary material for: CoHABIT: Complementary Evaluation of Furniture Layouts through Spatial Rules and Household Routines
Source: arXiv:2611.29494 source file (2026-11-22)
Supplement: Supplementary file 19 [file f_trajectory_examples.tex]

\subsection{Recorded resident trajectories}
\label{app:trajectory_examples}
Figure~\ref{fig:recorded-trajectories} shows two seven-day executions in furnished house 00663: two residents and 126 original goals. These earlier fixed-agenda examples are separate from the daily-policy comparisons.

\begin{figure*}[t]\centering
\includegraphics[width=\textwidth]{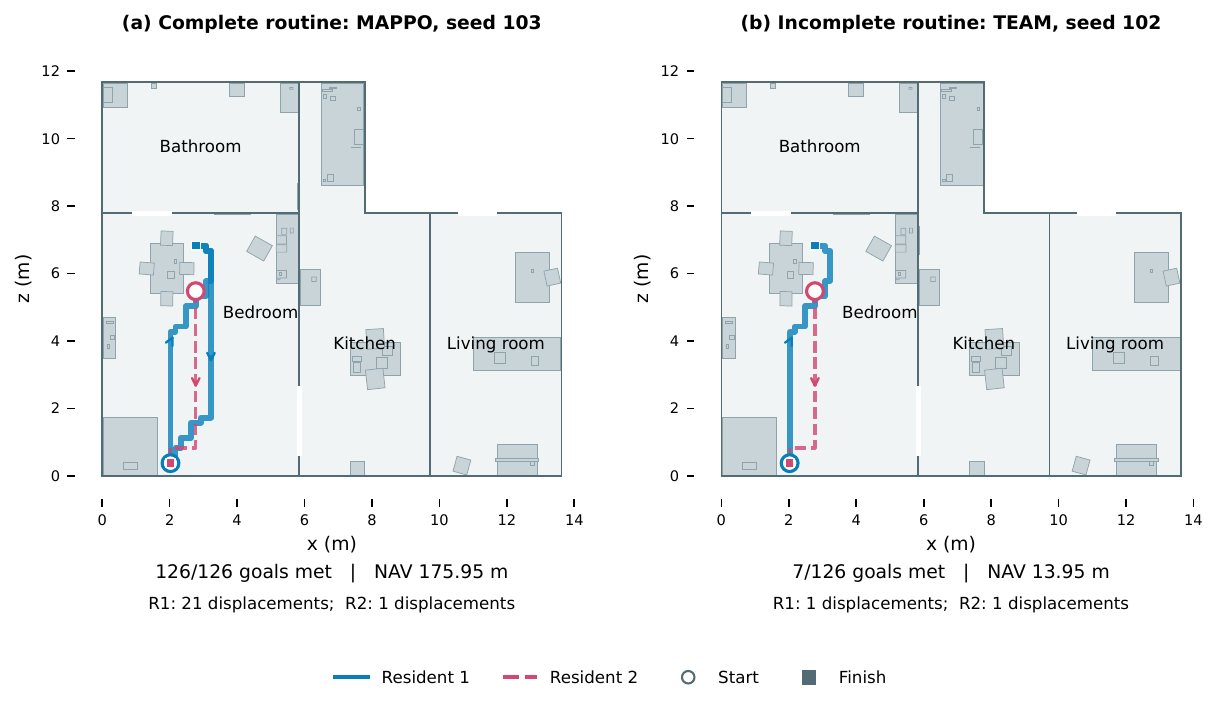}
\caption{\textbf{Read routes together with fulfilled needs.} In the same furnished home, MAPPO fulfills 126/126 goals and travels 175.95\,m; TEAM fulfills 7/126 and travels 13.95\,m, also repeating 497 zero-distance NAV actions. Blue/pink denote residents; circles/squares mark starts/finishes. Repeated traversals share a route. Efficiency is assessed jointly with original-need completion. The executions compare the recorded policy--training combinations.}
\label{fig:recorded-trajectories}
\end{figure*}

\paragraph{What the lines represent.}
Lines reconstruct committed NAV actions on shortest-grid routes, checking geometry, endpoints and distances within the navigation model. Both executions remain in one room; this agenda has single-room coverage. Coincident endpoints retain overlapping markers.

\subsection{Calendar diversity at equal demonstration volume}
Each arm uses 36 demonstrations, 27,158 resident/action/selector-matched examples and 2,048 updates. All 288 cases per actor are independently audited across four paired initializations (Table~\ref{tab:family-matched-volume}).
\begin{table*}[t]\centering\small
\caption{Shifted completion out of 72. S: synchronous training; D: diverse calendars. Bold: higher.}
\label{tab:family-matched-volume}
\begin{tabular}{@{}lcccc@{}}\toprule
Repeat & Development S & Development D & Unfitted S & Unfitted D\\\midrule
1 &36&\textbf{72}&36&\textbf{42}\\
2 &48&\textbf{72}&36&\textbf{72}\\
3 &54&\textbf{72}&60&\textbf{72}\\
4 &66&\textbf{72}&36&36\\\bottomrule
\end{tabular}
\end{table*}
Transfer discordances (diverse-only/control-only) are 24/18, 36/0, 12/0 and 0/0 across repeats. Both repeat~4 actors fail on home 06417 under either calendar: unfitted synchronous coverage is 36/72, versus 72/72 in the other repeats. Thus aggregate gains coexist with local regressions and a shared transfer failure. Action-limit stops and their incomplete pair comparisons retain an unresolved verdict. These results cover the inspected development and TRAIN inputs under numerical simulator profiles.



\input{supplement_sections/f_training_traces}
