# Supplementary material for: CoHABIT: Complementary Evaluation of Furniture Layouts through Spatial Rules and Household Routines
Source: arXiv:2611.29494 source file (2026-11-22)
Supplement: Supplementary file 20 [file f_whole_home.tex]

\subsection{Comparing furnished homes through whole-apartment routines}
\label{app:whole-home-comparison}
Matched routines link rest, sink use, deliveries, work, meals and conversation. Admitted furniture and routes support timed resource reservations.

Reference and finite temporal controllers each fulfill all 1,976 needs in 108 independently replayed executions across three admitted development homes. Each controller yields 84 complete joint and 12 complete single-resident comparisons. Opposing resident costs occur in 14 reference and 20 temporal joint comparisons. Profiles are compared on common admitted homes.

Matched households and calendars retain completion and personal pending-need latency:
\begin{equation}
L_i=\sum_{r:\,i\in\mathcal B_r}\bigl(\min\{T_r,\tau\}-a_r\bigr),\qquad L_\Sigma=\sum_i L_i.
\end{equation}
The sum covers the original needs released by $\tau$ ($a_r\leq\tau$). Here $a_r$ is release time, $T_r$ is physical completion ($+\infty$ if unmet), $\tau$ is the common horizon, and $\mathcal B_r$ contains beneficiaries. Shared needs contribute to both residents. $L_\Sigma$ measures pending-need time (reported as $L_\Sigma$ in the route figure); earlier results retain their stated burden definition $C$.

\textbf{Scheduling control.} For synchronous work in 00359 versus 00650, temporal search removes the reference reversal below. Both residents favor 00359 at both speeds: its advantage spans 56--64 need-seconds at equal speeds and 40--86 after the speed change, across two calendars. Apartment order is schedule-conditioned.

The main-paper routes reconstruct 36 verified NAV transitions; plotted intersections describe spatial overlap, with simultaneous collisions outside the motion model. Earlier daily-policy examples below retain their original protocols.

\begin{figure*}[t]\centering
\begin{minipage}[t]{.48\textwidth}\vspace{0pt}\centering
\includegraphics[width=\linewidth]{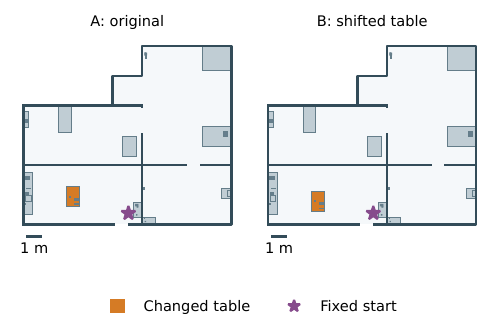}
\captionof{figure}{\textbf{Controlled furnishing change.} The table and supported objects move together; room geometry, other furniture and start remain fixed. Cost compares complete identical needs.}
\label{fig:paired-00685}
\end{minipage}\hfill
\begin{minipage}[t]{.48\textwidth}\vspace{0pt}\centering
\includegraphics[width=.82\linewidth]{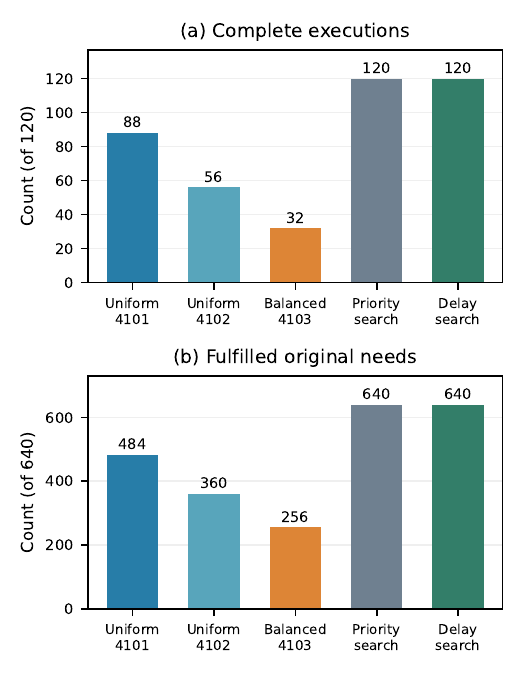}
\captionof{figure}{\textbf{Frozen actors and temporal controls.} Visual summary of Table~\ref{tab:frozen-eligibility}, with 640 original needs per method under corrected timing. Actors denote distinct checkpoints; the figure summarizes their existing executions.}
\label{fig:frozen-temporal}
\end{minipage}
\end{figure*}

\textbf{Learned whole-routine comparison.} After 28 TRAIN routines in two homes, actor 6101 completes 106/108 development executions and 1,956/1,976 needs, versus its parent's 12 and 989 under identical readiness. Independent replay verifies both own-action evaluations without fallback. Of 92 complete apartment pairs, 80 are joint; four expose personal tradeoffs. Two home-work executions each leave ten needs unmet, censoring four pairs. This matched gain combines balancing and additional training.

\textbf{Whole-apartment readout.} Independent replay verifies both executions and recomputes $L_\Sigma$. Relative to 00650, home 00359 reduces residents' latency by 28.25 and 30.125 need-seconds, totaling 58.375. Movement contributes 65.575 less, witnessed forced waiting 7.2 more; other components match. Both residents benefit because shorter travel outweighs waiting. This direct joint comparison requires no solo-policy success.

Under reference execution, work at home in the same apartments changes $L_{\Sigma,A}-L_{\Sigma,B}$ from $[-363.0,-357.4]$ to $[+173.9,+177.1]$ need-seconds across two calendars when only resident~2's speed decreases from 1.20 to 0.65\,m/s. This aggregate reversal reflects opposing personal costs.
