# Supplementary material for: CoHABIT: Complementary Evaluation of Furniture Layouts through Spatial Rules and Household Routines
Source: arXiv:2611.29494 source file (2026-11-22)
Supplement: Supplementary file 21 [file j_final_results.tex]

\section{Shared-layout completion, ablation, and temporal generalization}
\label{sec:final-complementarity}
\subsection{The same 50 furnishing pairs}
\paragraph{Acceptance and denominators.}
All results below come from completed independent action/event replay audits, with original-need identities and the pending-need integral checked separately. Replay verifies record consistency with the simulator; original-need checks determine routine completion. All failures and technical truncations remain in the denominators. No models were retrained for these evaluations.

\paragraph{Matched inputs.}
The static-study cohort supplies 100 furnished scenes, each executed in solo, asynchronous-pair and synchronous-pair contexts: 300 scenarios and 150 matched A/B comparisons per method. These are one- and two-resident experiments, distinct from the three-resident family series. The frozen uniform6101 actor is evaluated at update 512. Every A/B comparison matches needs, numerical profiles, release times, horizon and execution protocol. All 150 A/B pairs are explicitly bound by pair identity and context and pass the same strict input validator.

\begin{center}\begin{minipage}{\linewidth}\centering\small
\captionof{table}{Independent shared-layout outcomes. Full: all original needs completed; observed: scalar available over the declared horizon. Each row retains 300 scenarios and 5730 needs.}
\label{tab:final-pairs50}
\begin{tabular}{@{}lrrr@{}}\toprule
Executor/interface & Full & Needs met & Observed\\\midrule
Coarse navigation&27&1345&37\\
Corrected navigation&51&1770&58\\
NAV-only mask&51&1770&71\\
Request + NAV mask&51&3775&300\\
Reference planner&51&3775&300\\\bottomrule
\end{tabular}\end{minipage}\end{center}

The corrected navigation uses a 2.5-cm grid and rejects interaction through unrelated furniture. This correction changes the execution geometry while learned weights remain fixed. Repeated blocked-route actions explain the 242 technical caps after the geometry correction. Masking only NAV reduces unavailable outcomes to 229, with completed needs and full scenarios unchanged. Masking currently unreachable requests as well yields 2005 additional completed needs and no unavailable scalars under the same 12000-action limit. Each mask configuration defines an explicit deployment interface for the frozen actor. Every original request remains in the evaluation denominator. Horizon-censored scalars describe partial execution; complete matched routines support model-specific cost comparisons.

The corrected-grid reference and the request-plus-NAV executor each complete 17 scenes in all three contexts. Only pairs 009, 026, 028 and 041 have both alternatives complete in every context: 12 of 150 context-specific comparisons. All 12 have exactly zero A-minus-B household latency. The other 138 comparisons remain unsupported for complete-routine comfort ranking. The NAV-only interface also supports 12 complete comparisons; coarse navigation supports six. Thus the experiment establishes improved execution and observability; the input-equivalence check below determines how its paired outcomes can be interpreted. Residual unreachable targets and unresolved geometry retain their separate diagnostic statuses.

\paragraph{What the adapter actually distinguishes.}
A post-run inspection of all 150 saved A/B input pairs finds 36 equivalent contexts, corresponding to 12 of 50 furnishing pairs. Equality holds for runtime nodes, rooms, navigation and scenario fields after excluding identifiers and source metadata. The remaining 38 pairs have different navigation inputs. All four complete pairs belong to the equivalent subset: pair 009 rotates a balcony chair, 026 a balcony storage cabinet, and 028/041 a balcony wardrobe. Each edit reverses the front by $180^\circ$ without changing its footprint; none of these objects is referenced by an original task. The adapter preserves all source furniture and uses its footprints as obstacles, but constructs interaction fronts for task targets. These four edits preserve interaction points and routes, explaining equal delays through unchanged task-relevant runtime inputs. This motivates the task-relevant input checks used for the interventions in Appendix~H.

\subsection{Profile-by-calendar pilot on complete pairs}
A preregistered exploratory pilot conditions on the four complete pairs above. It crosses the original speed with a $0.7\times$ speed for resident~0 (1.20 to 0.84\,m/s), and original request releases with a 120-s shift for that resident. The geometry, all original requests, activities, deadlines and 7200-s horizon are unchanged; both A/B alternatives receive identical interventions. The 24 original cells are retained by audited provenance. The three new factorial cells yield 72 new scenarios, 36 new A/B comparisons, 72 reference executions and 144 independent audits. The already audited request-plus-NAV interface is fixed before observing these new outcomes; selection precedes the NAV-only ablation outcomes.

Both reference and the request-plus-NAV executor complete all 72 new scenarios, and every one of the 36 new paired latency differences is exactly zero. The original 12 paired comparisons were also tied. The source-input check explains these ties: both alternatives have equivalent task-relevant representations, and receive the same speed and release interventions. This pilot tests household-condition changes on equivalent executable layouts. Earlier profile-dependent contrasts use distinct runtime inputs and are reported separately. The four pairs form the fully complete subset of the 50-pair corpus.

\subsection{Frozen family actors at new calendar shifts}
\label{sec:calendar-extrap-final}
Eight frozen actors (paired initializations 7201--7204, synchronous-only versus diverse-calendar demonstrations) are tested at previously unevaluated 60-s and 330-s offsets. Each actor executes 288 scenarios on the same four admitted homes: three routines, six numerical profiles, two request realizations, two calendars and four homes. These are temporal generalization tests; no new geometric transfer or demographic validation is implied. The reference completes 288/288. All eight actor audits are accepted, with one distinct execution record per case.
\begin{table*}[t]\centering\small
\caption{Complete family routines at new offsets. Each offset has 144 scenarios; total denominator is 288. S: synchronous-only; D: diverse-calendar training.}
\begin{tabular}{@{}lrrrrrr@{}}\toprule
 &\multicolumn{2}{c}{60 s}&\multicolumn{2}{c}{330 s}&\multicolumn{2}{c}{Total}\\
Seed&S&D&S&D&S&D\\\midrule
7201&72&126&72&114&144&240\\
7202&72&144&84&144&156&288\\
7203&141&144&114&144&255&288\\
7204&108&108&102&108&210&216\\
\bottomrule\end{tabular}\end{table*}

Diversity increases full completion in all four paired initializations by 96, 132, 33 and 6 scenarios, respectively. The descriptive totals are 1032/1152 versus 765/1152 across repeated scenarios and paired seeds. Gain varies across seeds, with 72 outcomes still incomplete for diverse7204. Complete routines support apartment-cost comparisons; incomplete outcomes retain their policy-conditioned status.

\paragraph{Overall interpretation.}
The static, preference and dynamic studies measure complementary properties under declared conditions. Earlier complete-routine witnesses demonstrate schedule-dependent rankings and personal tradeoffs. The shared-50-pair study additionally shows why task coverage must accompany behavioral evidence: spatial rules assess furniture fronts beyond those used by a particular routine. Together, the studies motivate complementary reporting of spatial validity, preferences, need fulfillment and individual burdens, supporting interpretable choices under explicit household conditions.
