# Supplementary material for: CoHABIT: Complementary Evaluation of Furniture Layouts through Spatial Rules and Household Routines
Source: arXiv:2611.29494 source file (2026-11-22)
Supplement: Supplementary file 22 [file k_illustrative_layouts.tex]

\FloatBarrier
\section{Task-covered furnishing interventions and audited trajectories}
\label{sec:illustrative-layouts}
\paragraph{Purpose and selection.}
These explanatory case studies connect a furnishing intervention to the routines that use it. They are distinct from the original 50-pair comparison. Three previously complete A scenes (009, 026, 028) supply real archived geometry; their new B variants change a task-used dining-table front, wardrobe position and sofa position, respectively. Bases are selected from cases with known completion for explanatory case studies. Before new execution, a finite protocol fixes the target, candidate order and input-only acceptance: no added floor-furniture overlap or outside-room area, all original task targets reachable, and at least 0.25\,m change in a task-node distance. The first admissible candidate is retained without consulting new policy outcomes. The first two sofa positions are rejected (overlap and outside-room placement); the third is admitted. No furniture or original need is removed.

\paragraph{Matched conditions and acceptance.}
Each new pair is evaluated in solo, asynchronous and synchronous contexts, with original speed or resident~0 slowed from 1.20 to 0.84\,m/s: 36 scenarios and 18 A/B comparisons per method. Releases are spaced every 120\,s instead of 180\,s, retaining the 180-s resident-1 offset in the asynchronous context, all task dependencies, and the 7200-s horizon. The denser request schedule defines a new evaluation condition. The frozen uniform6101 actor uses the audited request-plus-NAV interface. The checkpoint and execution interface are fixed before comparison. Both methods complete all 36 scenarios and all 660 original needs, and both independent audits pass. Every paired comparison is supported. The reference planner and learned executor yield the same paired costs on these cases.



\paragraph{What the examples add.}
The table-front reversal tests an assigned access interface on a physically symmetric table. Its 8.542--20.744 need-second differences quantify sensitivity to the assigned access side. The unequal personal differences (13.417 and 3.417 need-seconds in the synchronized normal-speed condition) remain reproducible simulator outcomes. We therefore use the directional wardrobe study below as the physically interpretable orientation example. Task coverage spans four functional rooms and hallway transit; the balcony has no assigned task. No preference reversal occurs.

The 0.40-m wardrobe and sofa translations also change runtime inputs, but their aggregate effects are small: B increases latency by at most 0.152 and 0.051 need-seconds, respectively. These small differences depend on the 2.5-cm navigation discretization and the executor's 0.2-s minimum NAV duration. Their role is to show that a visible, task-covered geometric change can have little impact under a declared routine. All examples retain the same reported static overlap/outside-room area as A. A subsequent fixed E/F rescore on these exact scenes is reported in Section~\ref{sec:efd-same-layouts}.

\paragraph{Trajectory provenance.}
Figures below use the prespecified synchronized original-speed condition for all three examples. Each plotted transition comes from an audited NAV event. Its polyline is reconstructed on the same pinned collision-free grid; the full distance matrix agrees exactly with the execution input, and every event duration agrees with $\max(0.2,d/v)$. Repeated identical routes are drawn once. Timelines retain actual action times; conflict labels require a causal event. The orange object is the sole furnishing intervention. The routes are reconstructed simulator paths.

\paragraph{Furnished views and complete routes.}
\label{sec:remaining-room3d}
The furnished views and full-apartment plans visualize the same executions. Each A/B pair shares camera, scale and lighting. Insets retain audited NAV transitions where perspective occludes paths. E, geometric Feng Shui and D are joined on these exact saved layouts (Section~\ref{sec:efd-same-layouts}); scores and route evidence retain their separate meanings. Each furnished view is followed by its complete plan and timeline.


\begin{figure*}[p]\centering
{\small
\captionof{table}{A-minus-B household pending-need latency (need-seconds). Positive values favor B. ``Slow'' changes resident~0 only. Every entry has complete original-need fulfillment.}
\label{tab:illustrative-deltas}
\begin{tabular}{lrrrrrr}\toprule
&\multicolumn{2}{c}{Solo}&\multicolumn{2}{c}{Asynchronous}&\multicolumn{2}{c}{Synchronous}\\
Intervention & Normal & Slow & Normal & Slow & Normal & Slow\\\midrule
Table front & 8.542 & 12.202 & 17.083 & 20.744 & 16.833 & 11.833\\
Wardrobe shift & -0.063 & -0.089 & -0.125 & -0.152 & -0.125 & -0.125\\
Sofa shift & -0.021 & -0.030 & -0.042 & -0.051 & -0.042 & -0.042\\
\bottomrule\end{tabular}}
\medskip
\includegraphics[width=.94\textwidth]{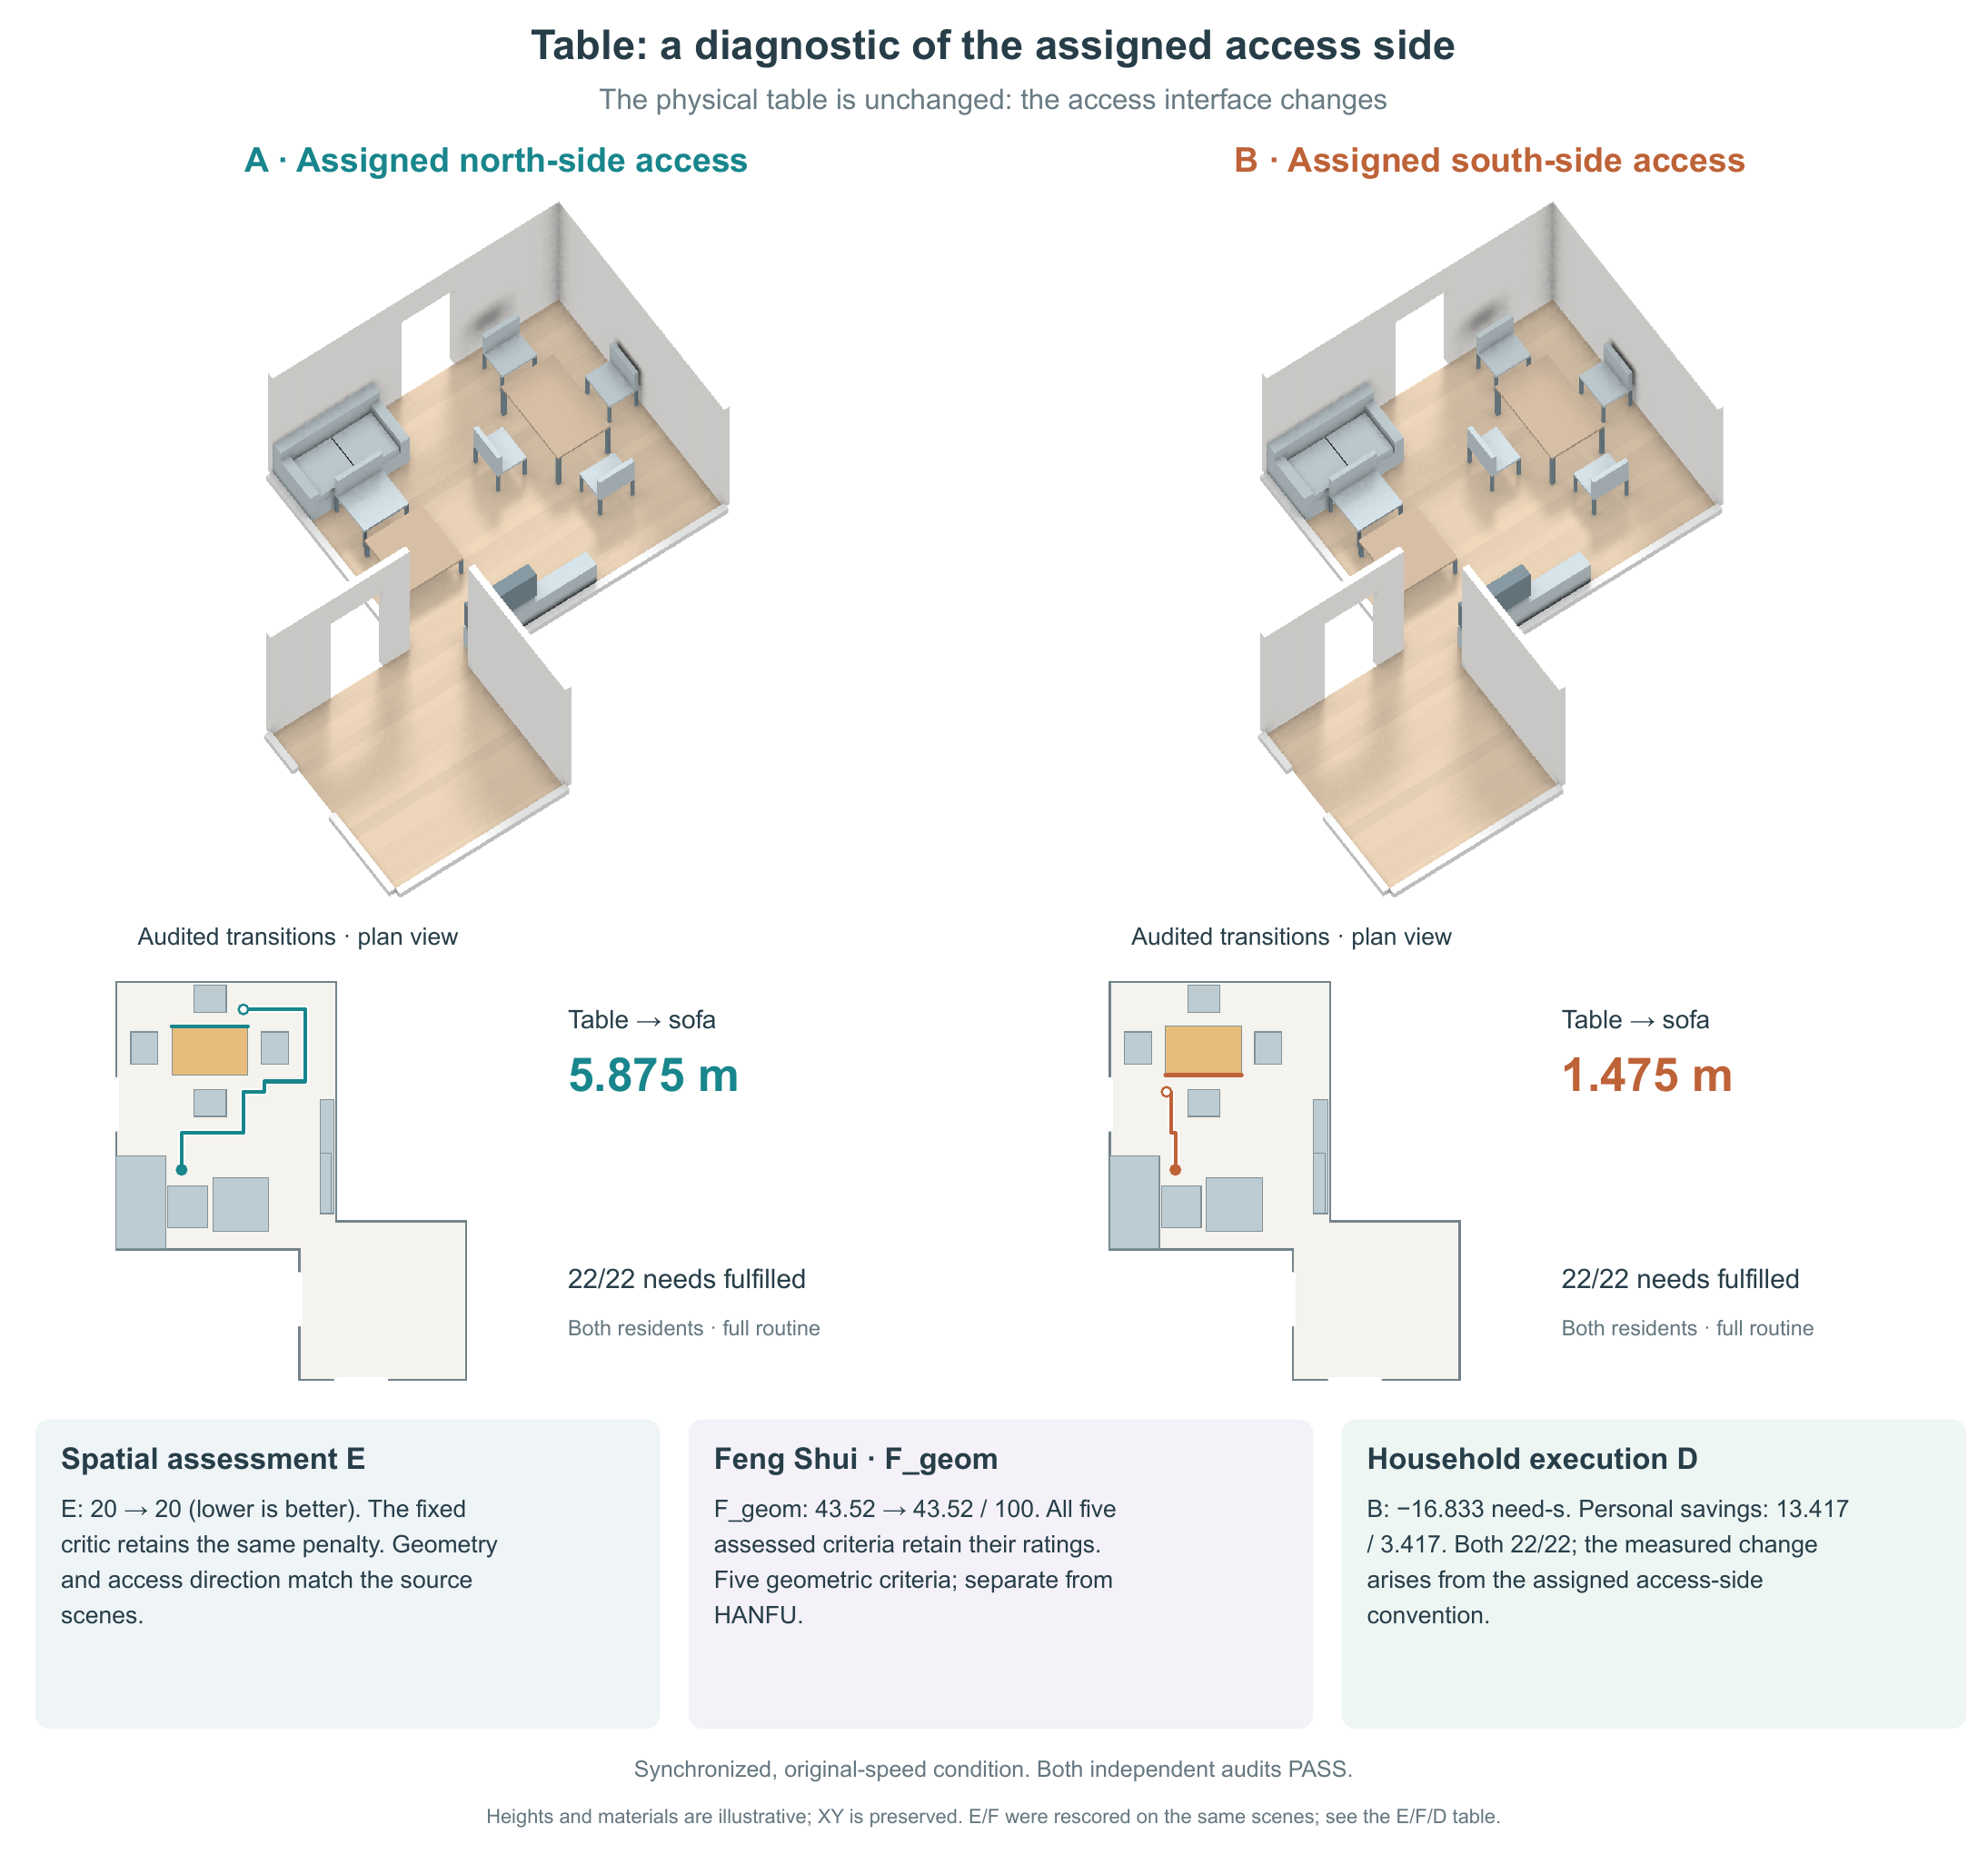}
\caption{\textbf{Assigned access-side diagnostic for a symmetric table.} The depicted table geometry is identical in A and B. Only its assigned interaction side changes, marked on the plan view. The audited table-to-sofa route changes from 5.875 to 1.475\,m and household latency decreases by 16.833 need-seconds, with unequal personal reductions of 13.417 and 3.417. The measured effect concerns the assigned interaction side of the symmetric table. The separately tested directional wardrobe provides the physically interpretable facade example.}
\label{fig:room3d-009}
\end{figure*}
\begin{figure*}[tp]\centering
\includegraphics[width=\textwidth]{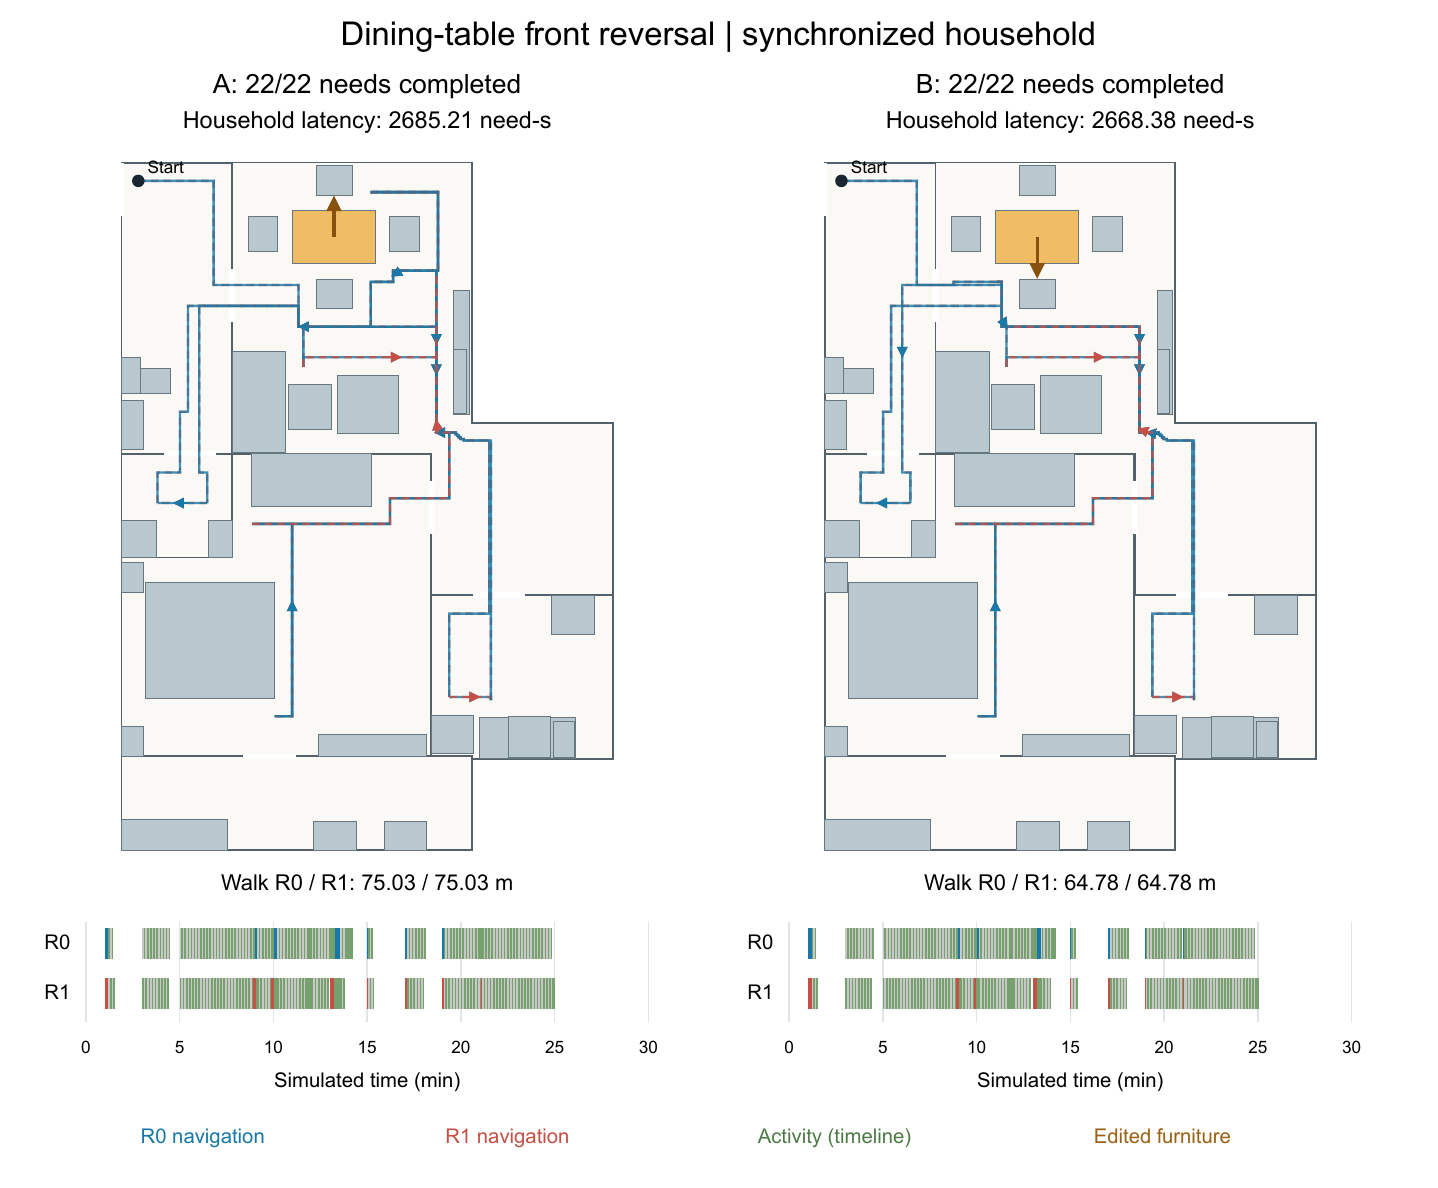}
\caption{\textbf{Assigned access-side diagnostic for a symmetric table.} Both layouts complete 22/22 needs. Reversing the table front changes access routes and reduces household latency from 2685.208 to 2668.375 need-seconds. The two residents benefit by different amounts under the declared access-side convention.}
\label{fig:illustrative-009}
\end{figure*}
\begin{figure*}[tp]\centering
\includegraphics[width=\textwidth]{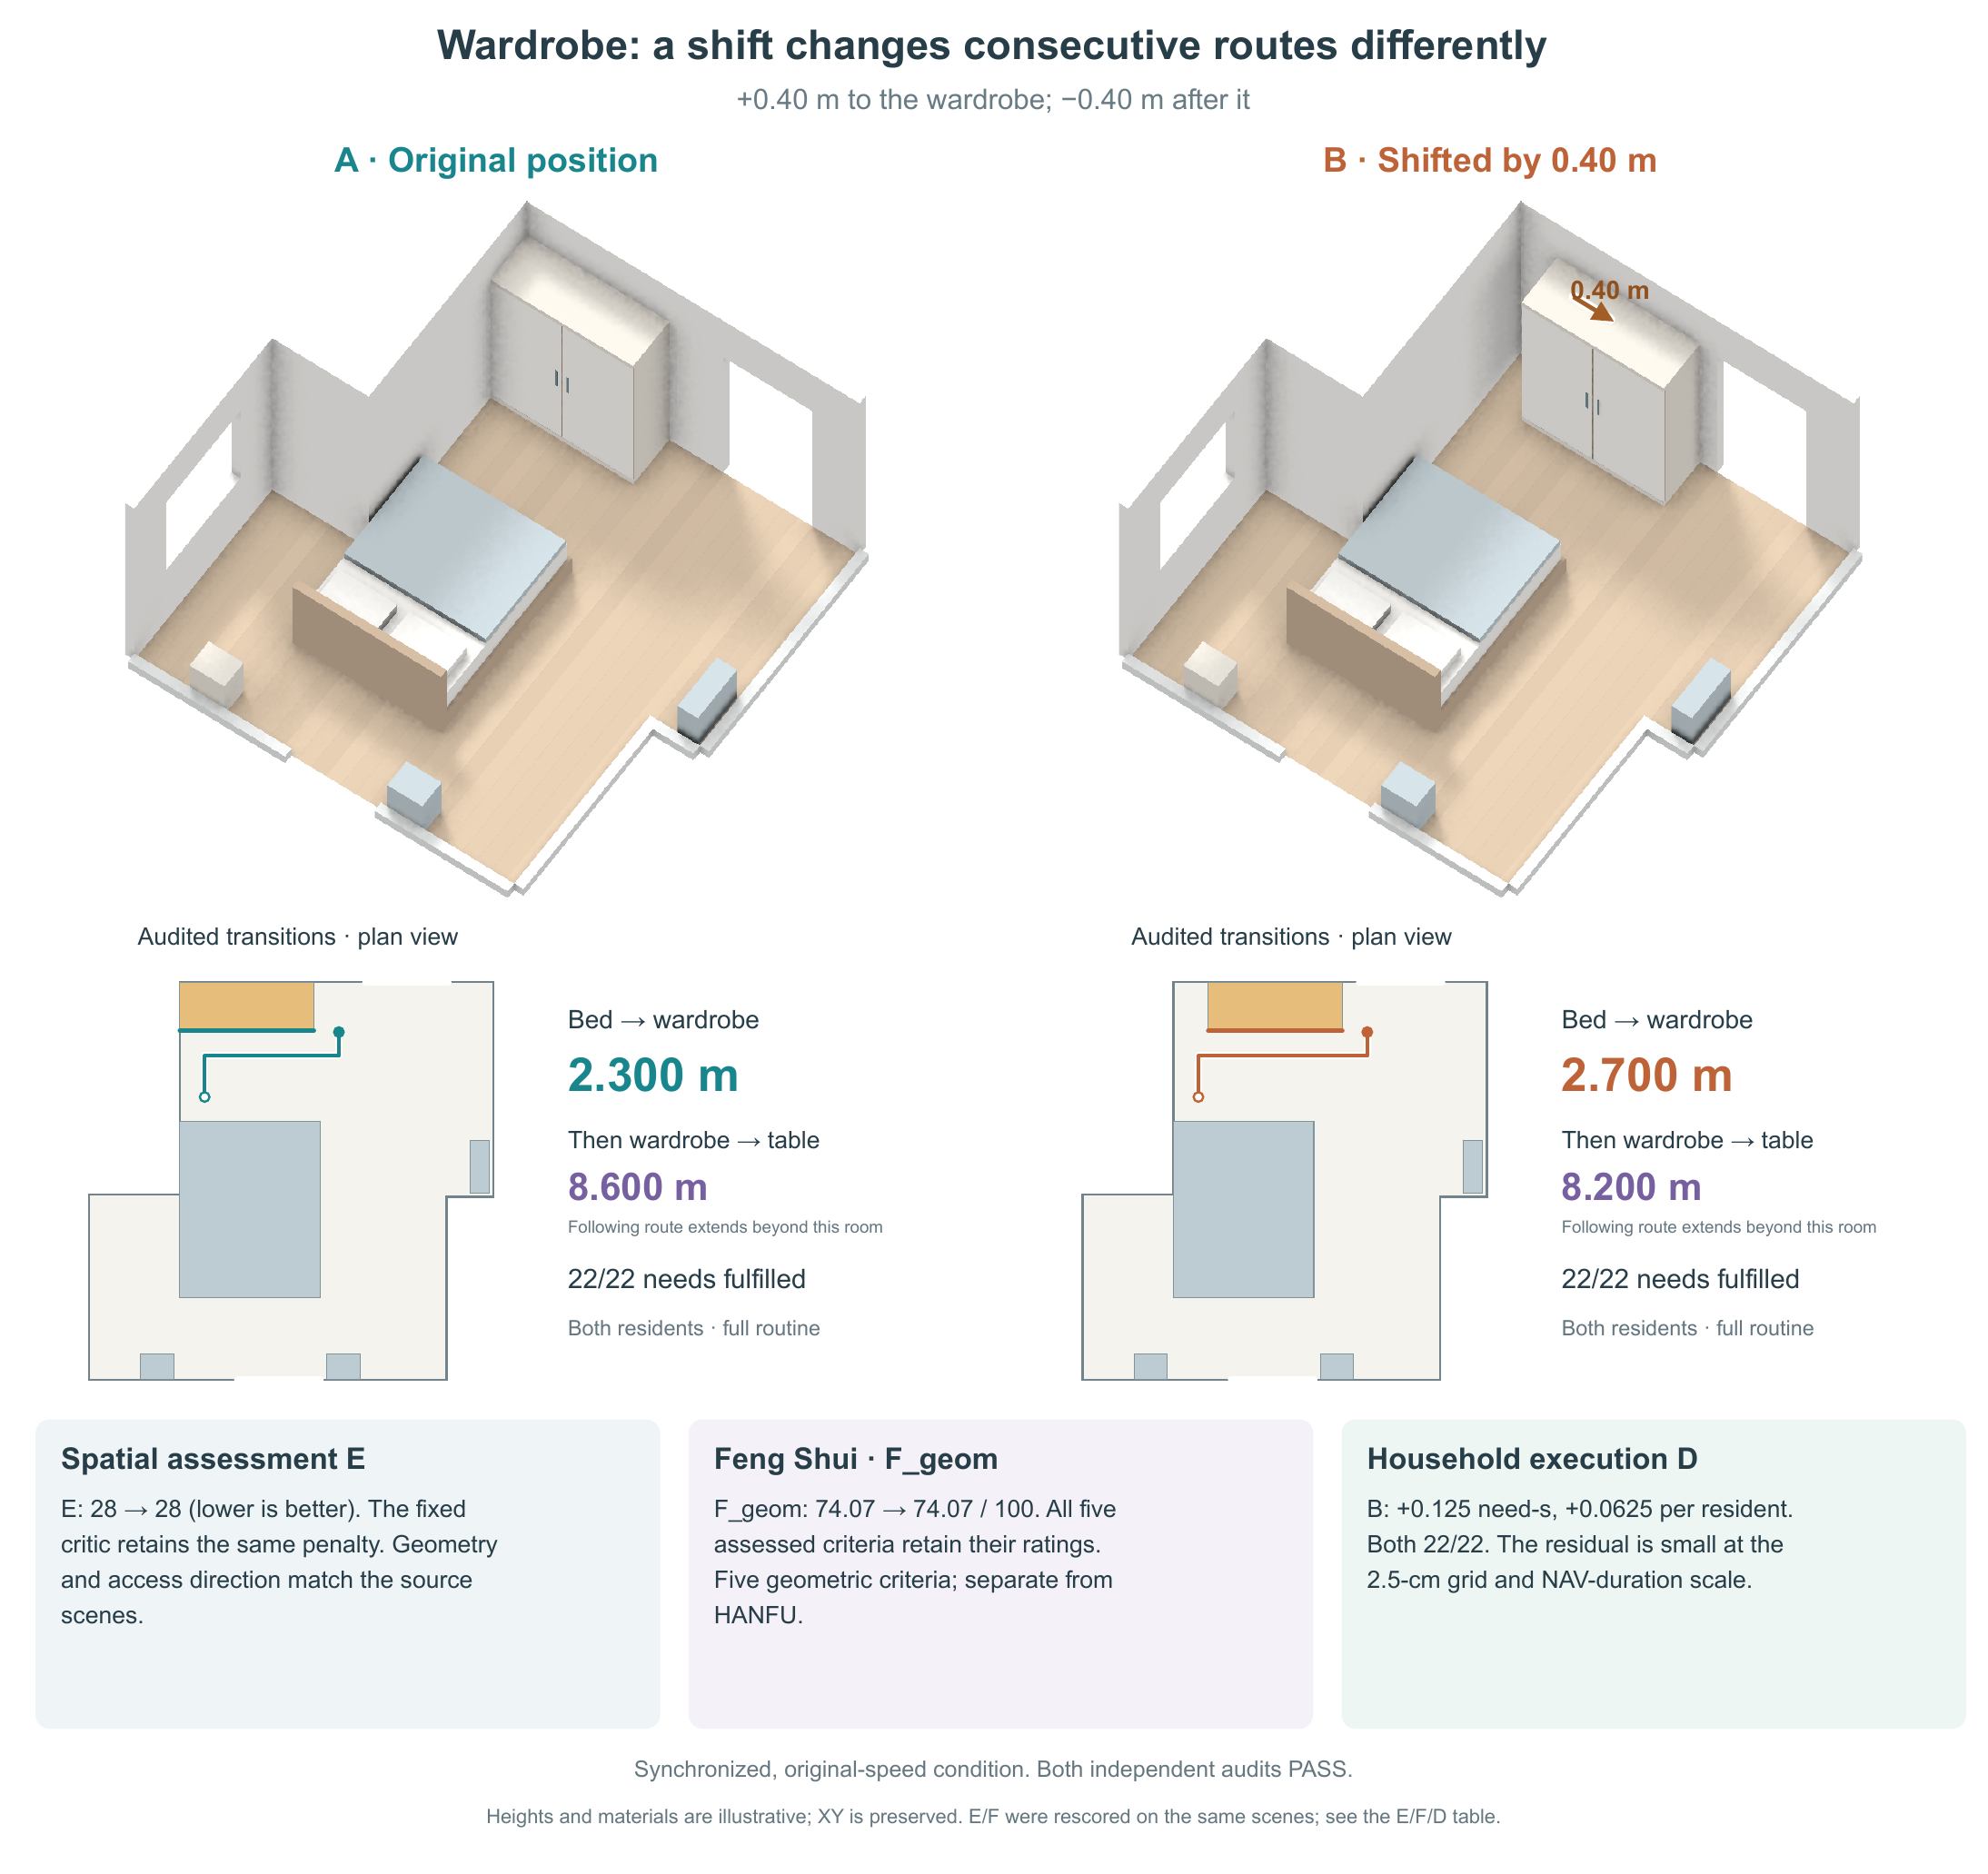}
\caption{\textbf{Wardrobe relocation: local route changes compensate.} Moving the wardrobe 0.40\,m increases bed-to-wardrobe distance from 2.30 to 2.70\,m but reduces the subsequent wardrobe-to-table route from 8.60 to 8.20\,m. The latter extends beyond the depicted room. Total walk changes from 60.625 to 60.700\,m per resident; the 0.075-m residual comes from entry-to-refrigerator navigation. Both layouts complete 22/22 needs. The 0.125 need-second household increment characterizes sensitivity at the grid and NAV-duration scale.}
\label{fig:room3d-026}
\end{figure*}
\begin{figure*}[tp]\centering
\includegraphics[width=\textwidth]{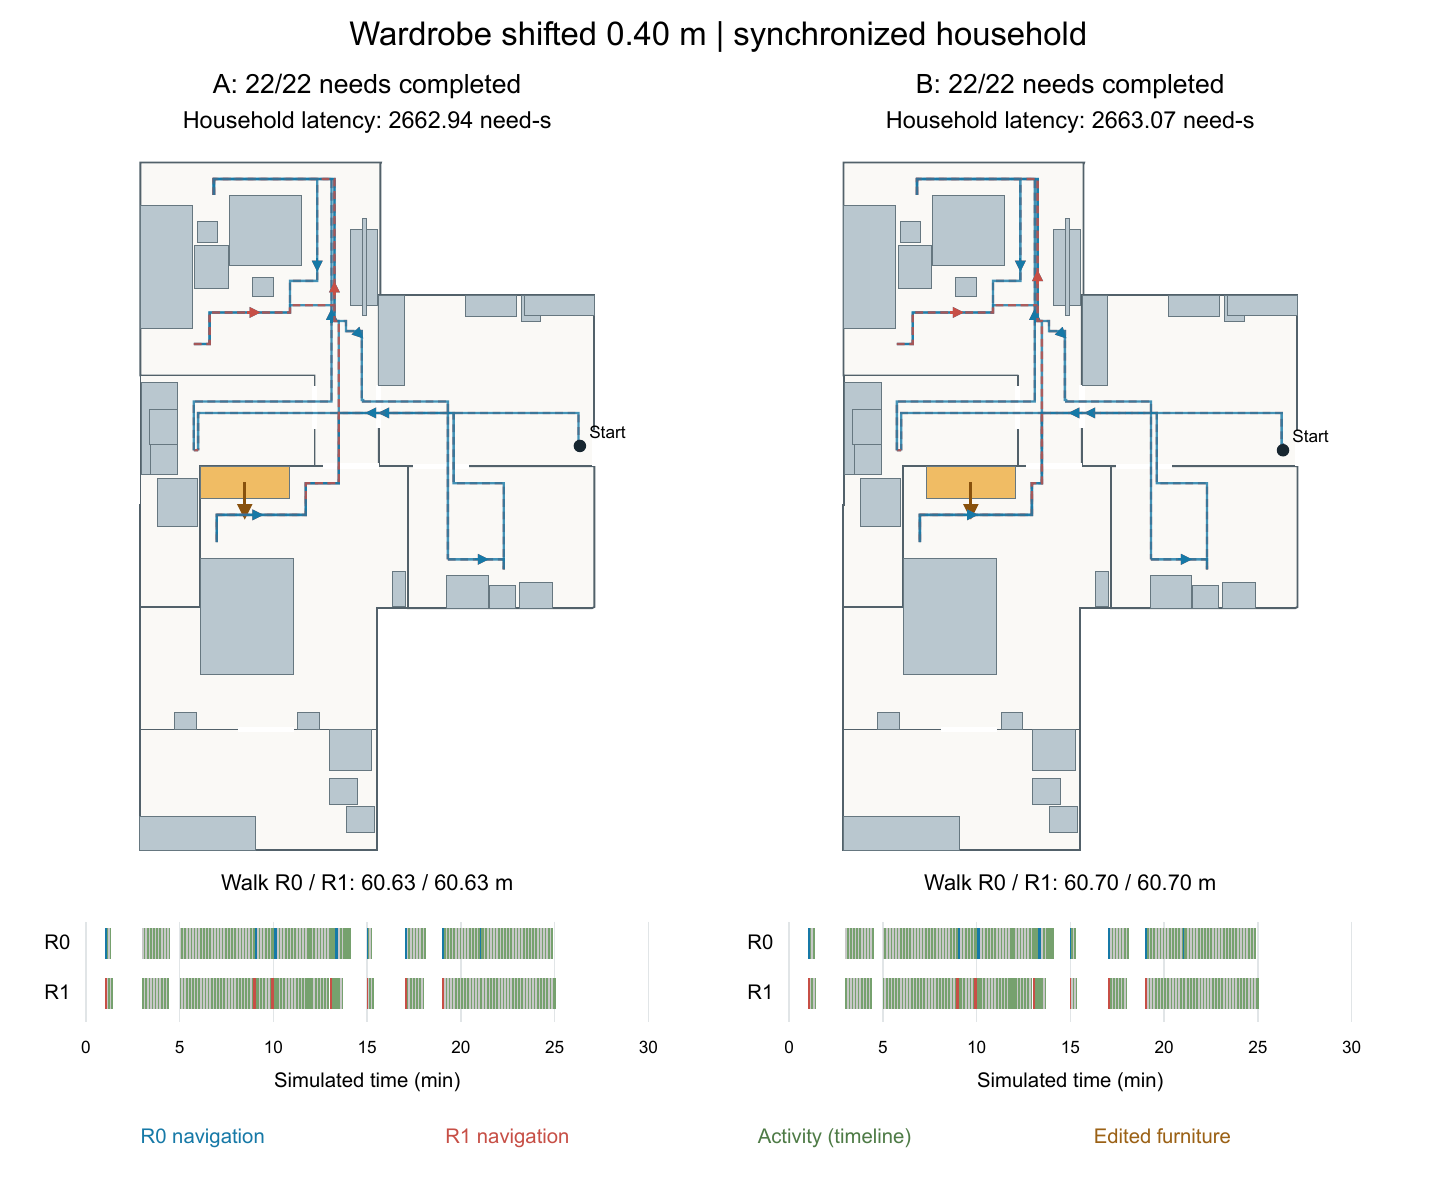}
\caption{\textbf{A visible relocation with a small routine effect.} The wardrobe moves 0.40\,m within its room without adding overlap. Both layouts complete 22/22 needs; latency changes from 2662.942 to 2663.067 need-seconds. The plan and timeline show the complete execution corresponding to the room view above.}
\label{fig:illustrative-026}
\end{figure*}
\begin{figure*}[tp]\centering
\includegraphics[width=\textwidth]{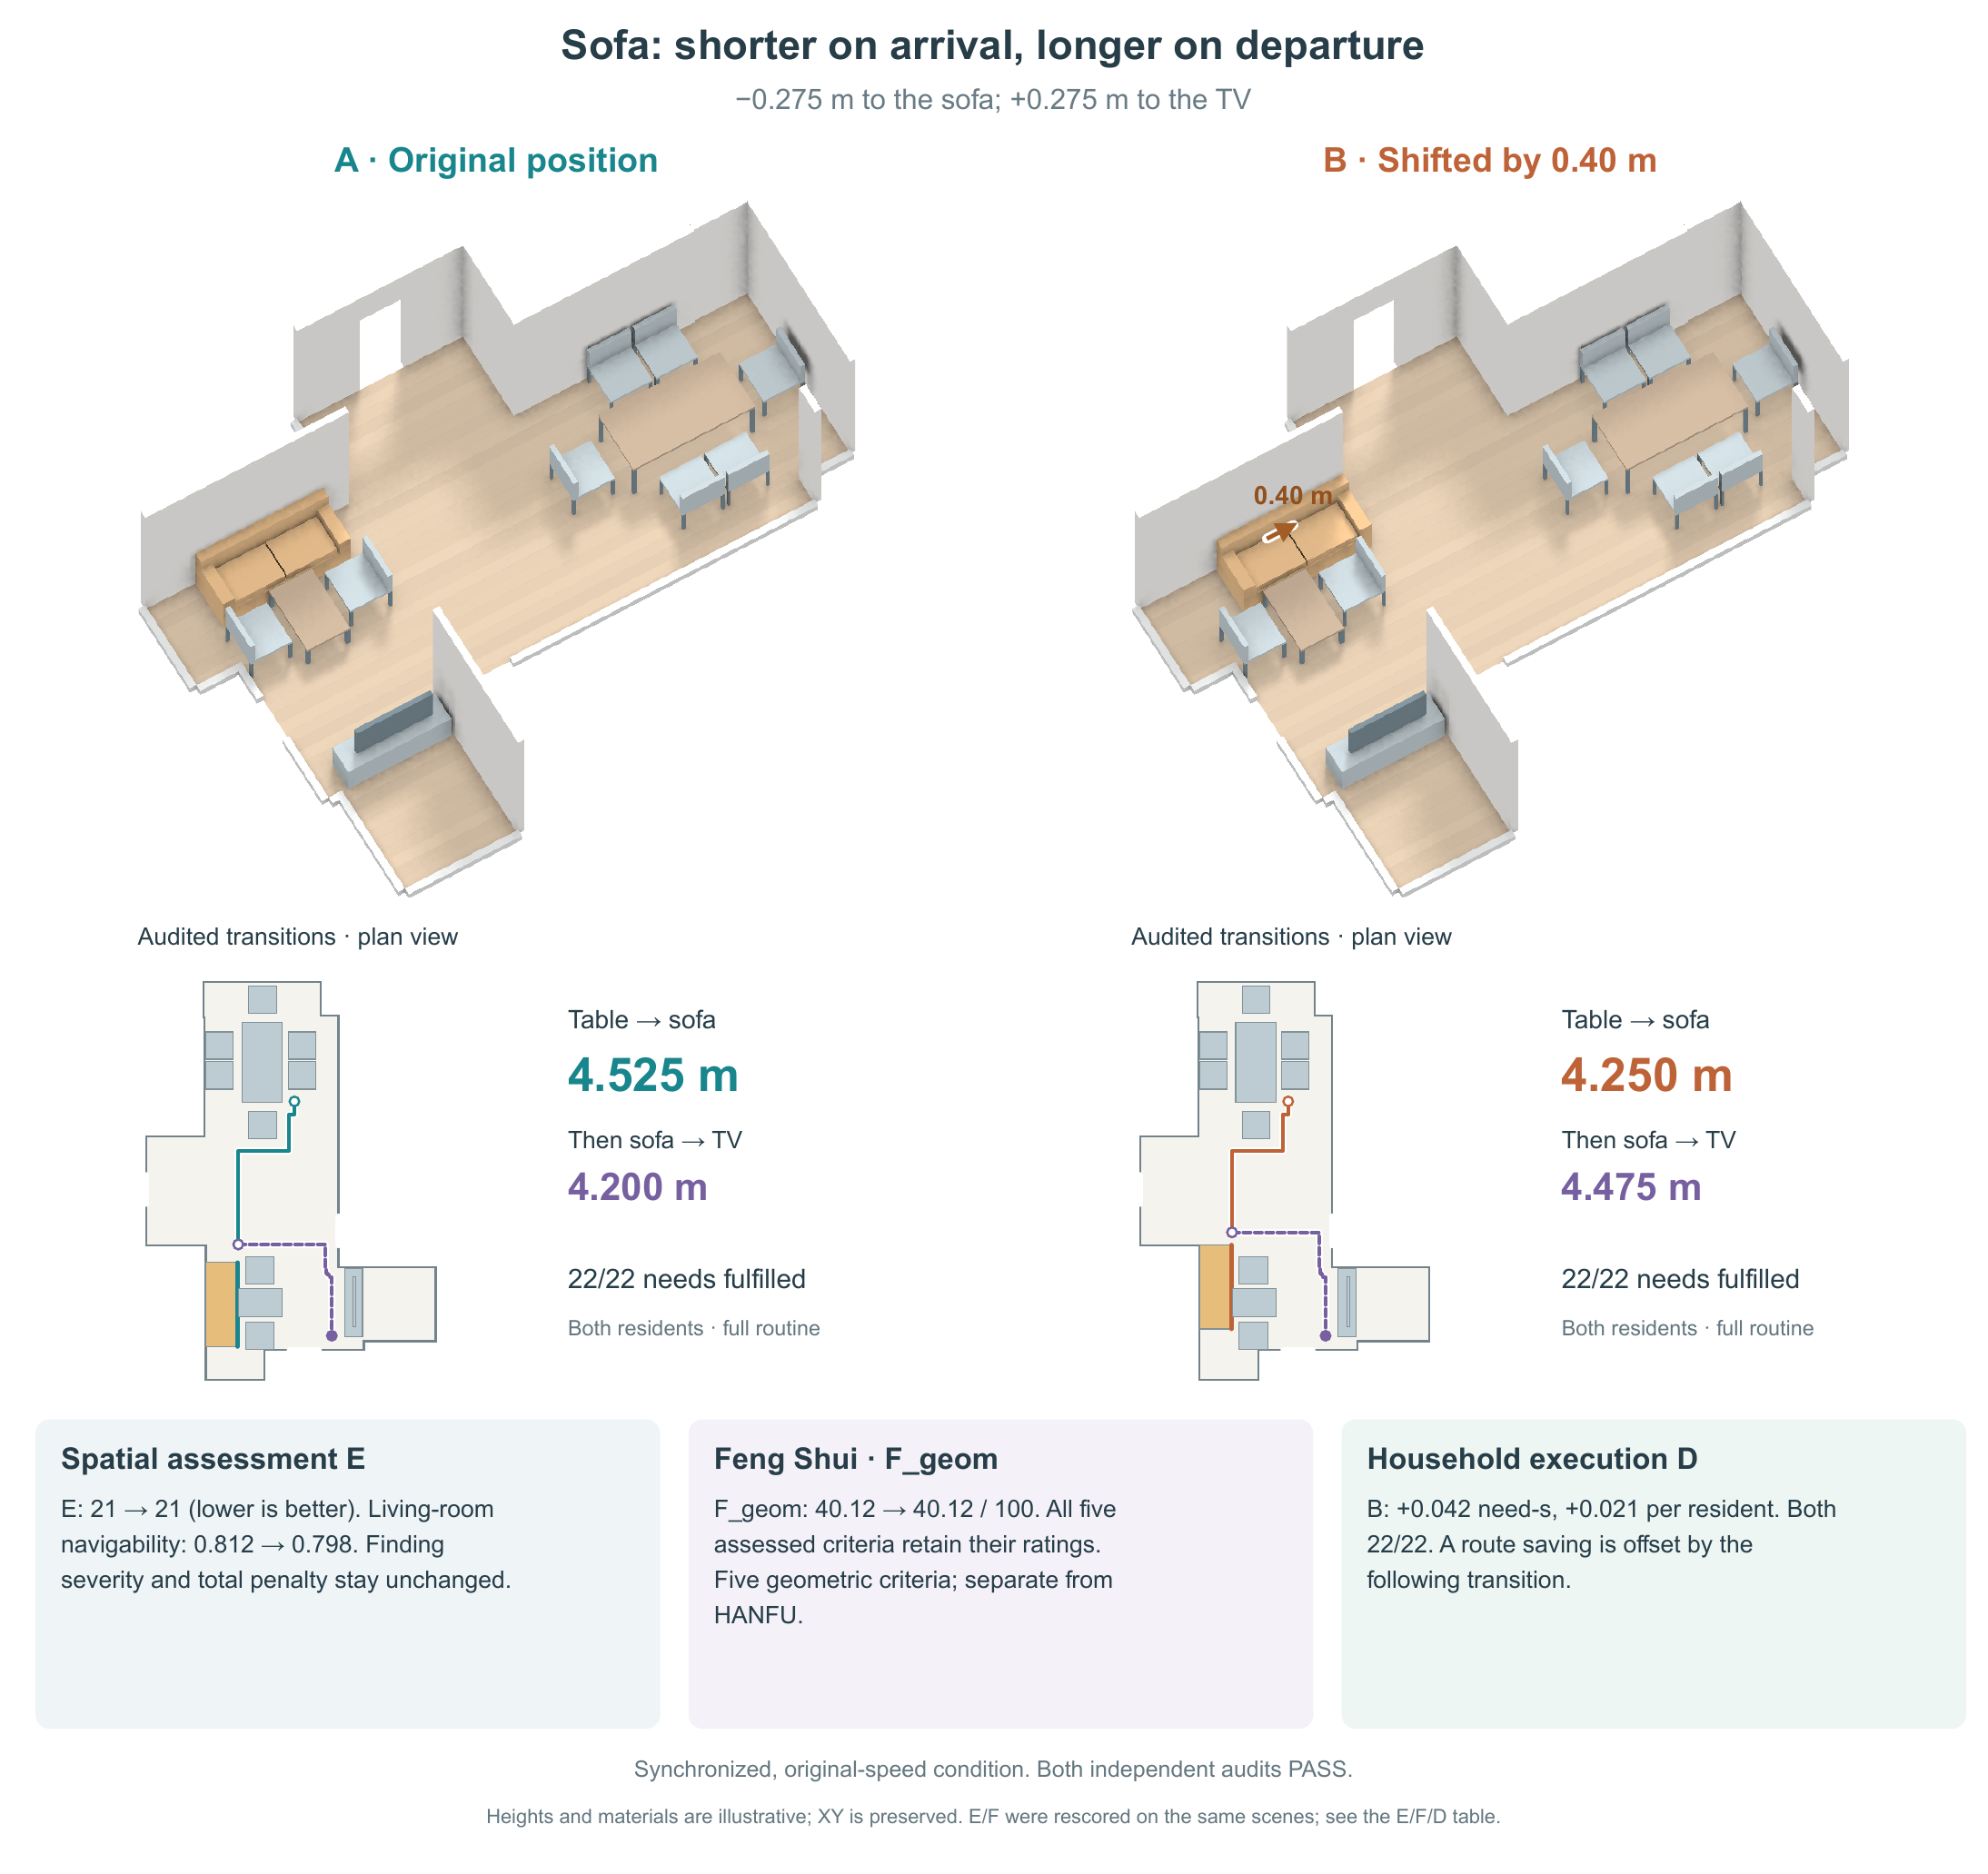}
\caption{\textbf{Sofa relocation: a shorter arrival is offset by a longer departure.} The accepted 0.40-m shift reduces table-to-sofa distance by 0.275\,m and increases sofa-to-TV distance by the same amount; the dashed purple route denotes the second transition. Geometry screening had already rejected two earlier candidates for overlap or outside-room placement. The complete routine retains all 22 needs. The remaining household latency difference is 0.041667 need-seconds; a 0.025-m entry-to-refrigerator route difference is retained in the full accounting. Spatial screening prevents invalid edits; household execution determines whether a locally shorter route yields a net benefit.}
\label{fig:room3d-028}
\end{figure*}
\begin{figure*}[tp]\centering
\includegraphics[width=\textwidth]{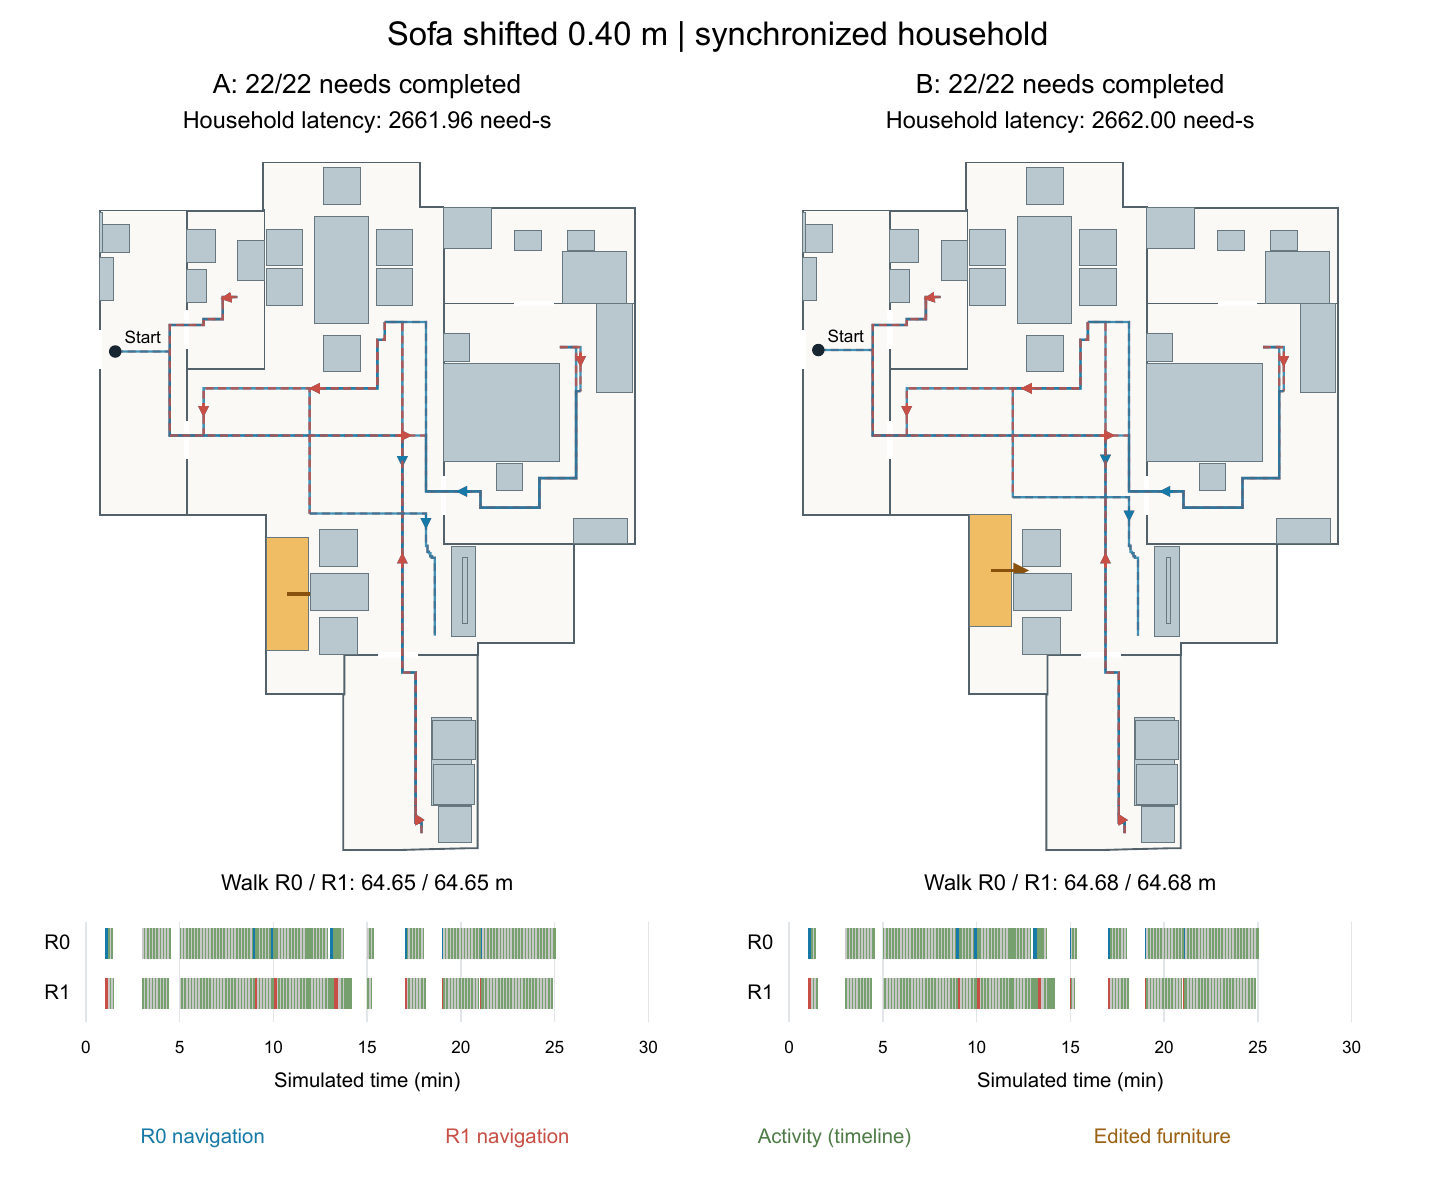}
\caption{\textbf{Local circulation changes with nearly constant aggregate burden.} A permitted 0.40-m sofa shift preserves access to all task targets. Both layouts complete 22/22 needs; latency changes from 2661.958 to 2662.000 need-seconds. The full plan and timeline complement the local arrival/departure routes in the room view above.}
\label{fig:illustrative-028}
\end{figure*}

\FloatBarrier
\subsection{Directional wardrobe with tasks in every room}
\label{sec:directional-wardrobe}
A wardrobe has a functional facade and a back, making the orientation edit interpretable. We retain the archived A geometry of apartment~009 and move its bedroom wardrobe 0.65\,m south in \emph{both} alternatives, leaving access on either side. A faces the bed; B reverses the facade by $180^\circ$ at the identical position and footprint. The common relocation defines the baseline for this controlled orientation comparison. Before execution, a finite protocol fixes the candidate shifts (0.65, 0.75, 0.85, 0.95\,m); the first candidate passes independent input checks for no added overlap or outside-room placement and complete target reachability. Candidates are selected using input geometry before policy evaluation.

All original task chains are retained. Entry storage and balcony storage/rest tasks are explicitly added, so the scenario now includes functional activities in all six source rooms. The same solo/asynchronous/synchronous contexts, two numerical speed profiles, 120-s releases and 7200-s horizon produce 12 scenarios and six matched comparisons per method. The frozen actor uses the fixed request-plus-NAV interface. Both the reference planner and neural executor complete all 12 scenarios and 280/280 needs; both independent audits pass. Their paired costs agree. This controlled case study compares complementary evidence under two executors with agreeing costs.

\begin{table}[t]\centering\small
\caption{Added household latency of facade B relative to A (need-seconds). Both variants fulfill every need.}
\begin{tabular}{lrr}\toprule
Context & Original speed & Resident 0 slower\\\midrule
Solo &4.125&5.893\\
Asynchronous &8.250&10.018\\
Synchronous &8.250&8.250\\\bottomrule
\end{tabular}\end{table}

In the prespecified synchronized original-speed condition, the bed-to-wardrobe route is 2.625\,m in A and 7.675\,m in B. The subsequent wardrobe-to-table route is 0.10\,m shorter in B, yielding a net 4.95\,m additional walk per resident. Each resident incurs 4.125 additional need-seconds; household latency changes from 3452.917 to 3461.167 need-seconds, about 0.24\%. The aggregate change is modest relative to the total routine latency. Independent event checks confirm completed activities in all six rooms in both variants, including the balcony.

Footprint validity alone leaves the pair tied, directional access explains the detour, and household execution quantifies its consequences under a declared schedule. These assessments thus answer complementary questions. The simulator represents fixed front-side access and timed use; articulated door kinematics lie outside its state model. Figure~\ref{fig:wardrobe-facade} preserves the actual XY geometry and audited routes; its 3D room views use schematic furniture meshes and illustrative materials.

\begin{figure*}[tp]\centering
\includegraphics[width=\textwidth]{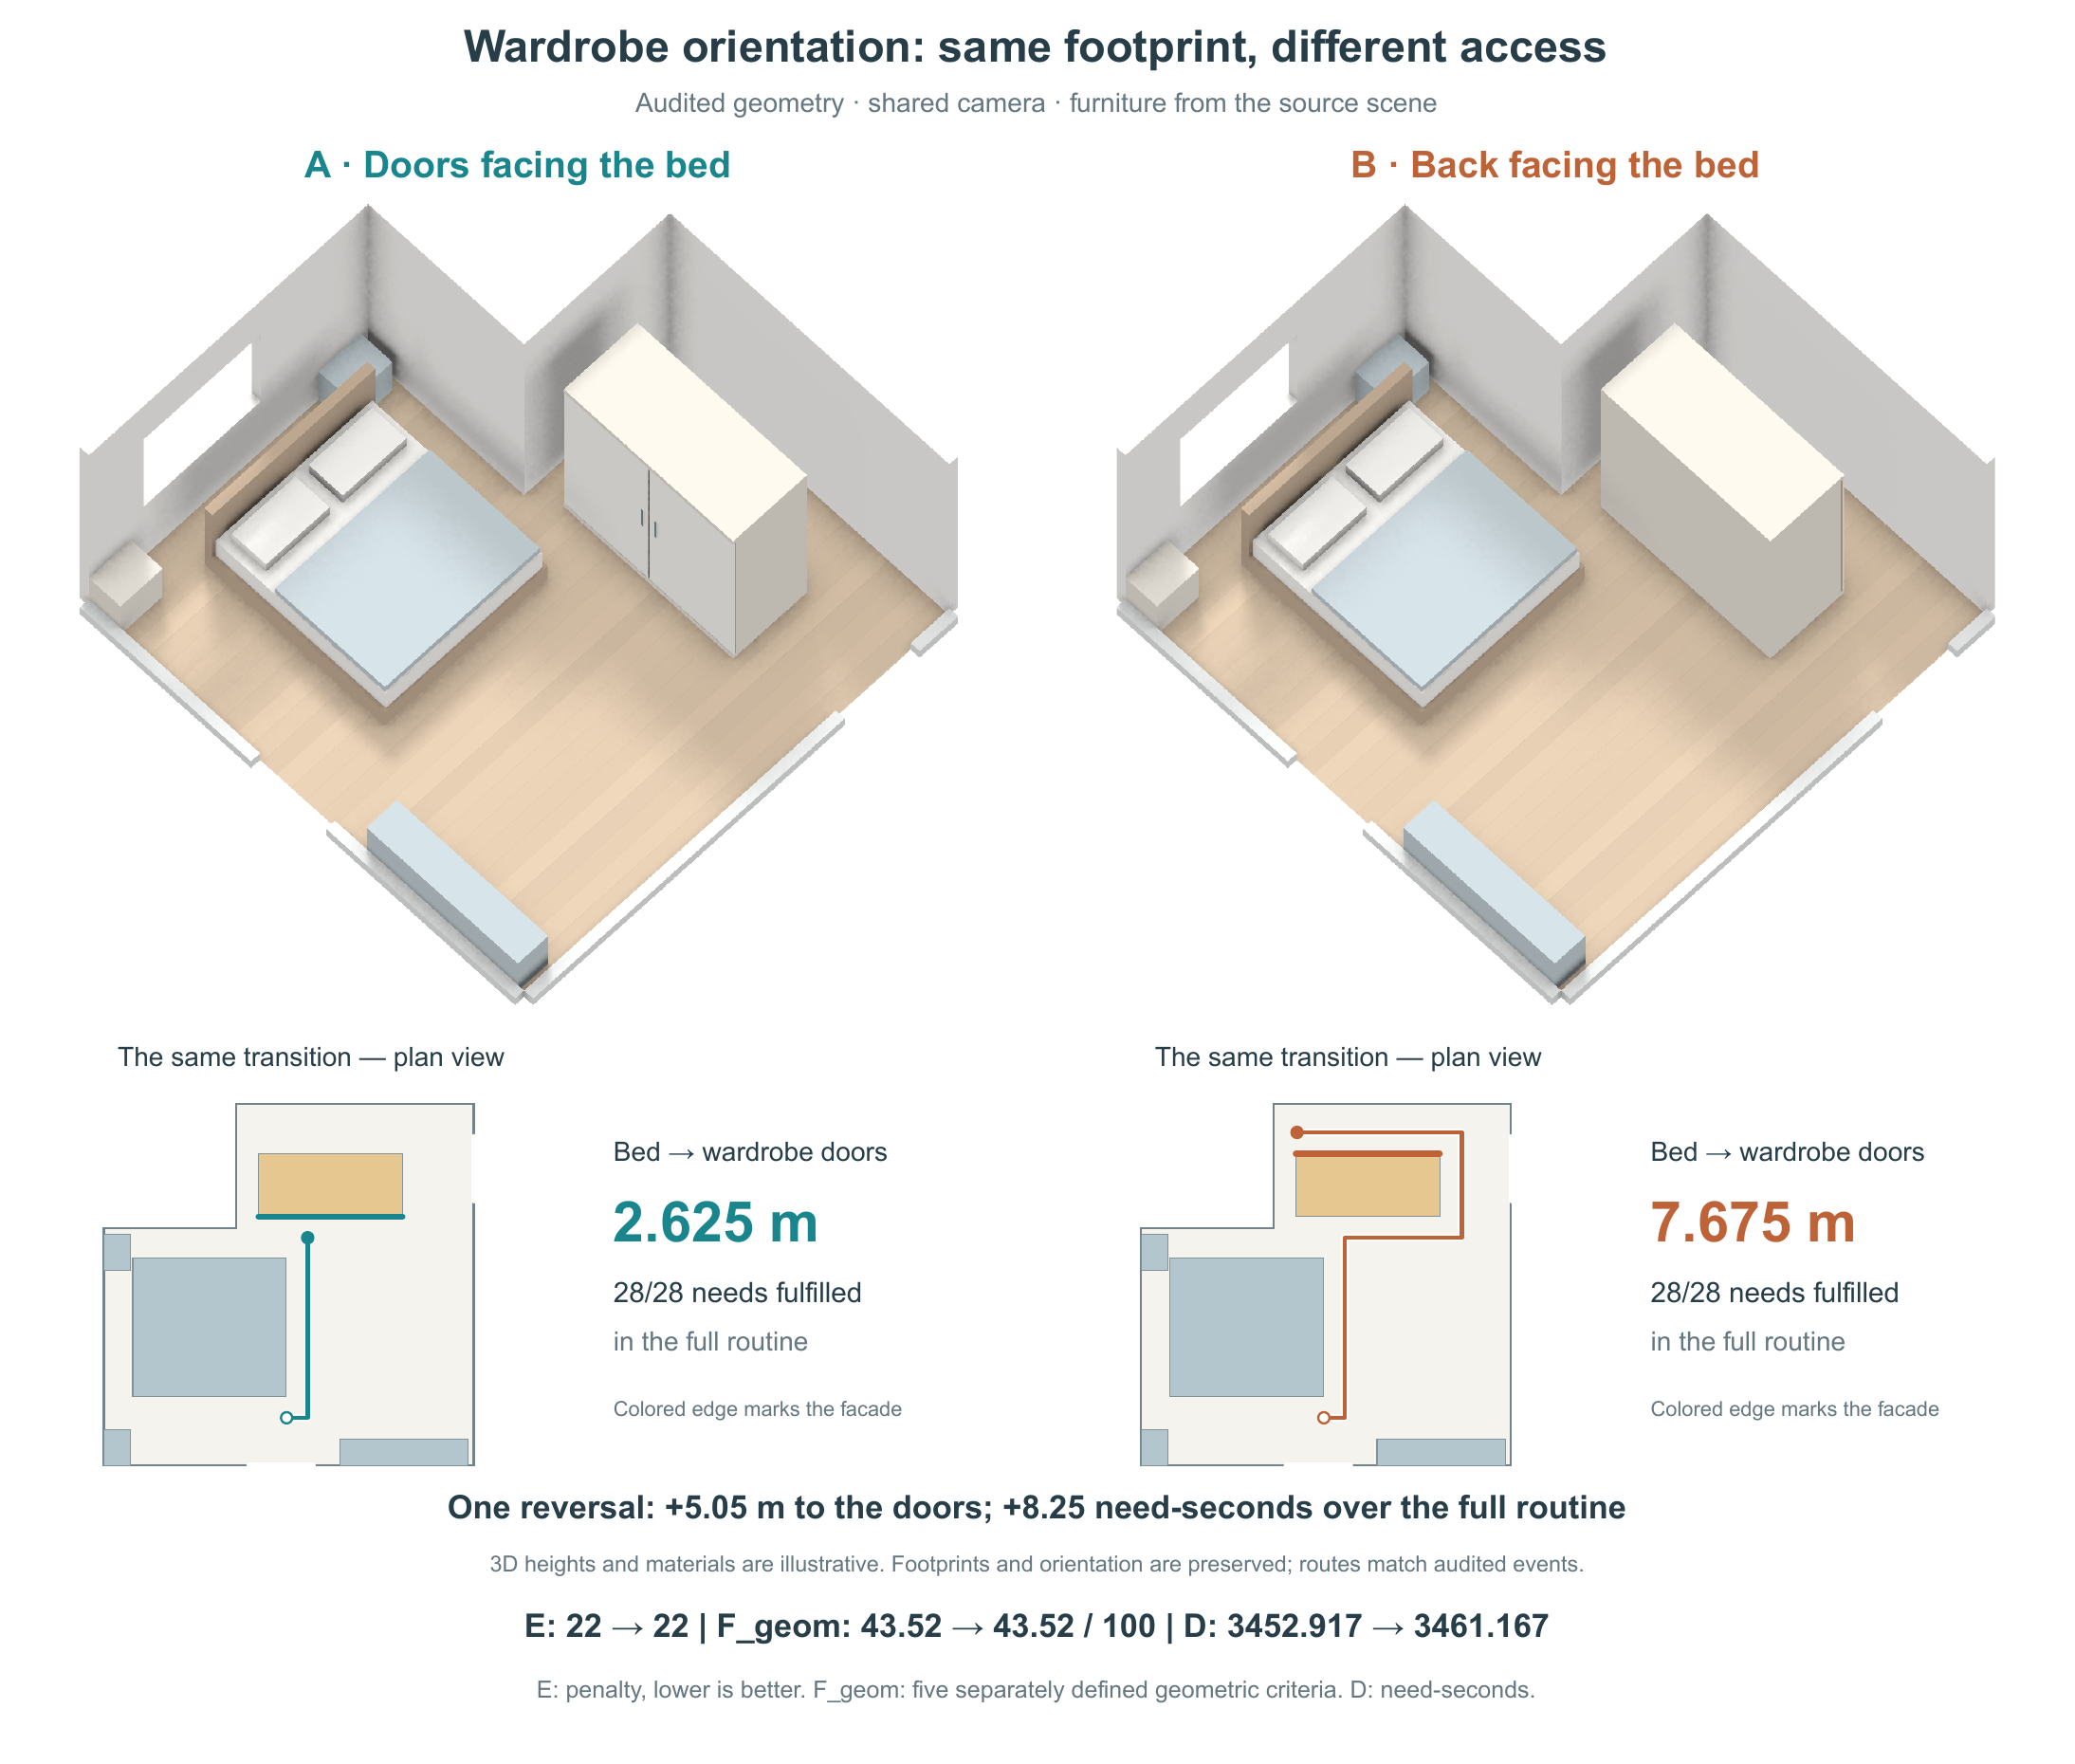}
\caption{\textbf{A directional object makes the orientation effect explicit.} The existing source-geometry room renderer shows wardrobe doors in A and its back in B from the same camera. Room and furniture footprints, openings and orientation follow the archived input; heights and materials are illustrative. The plan views below show audited routes without 3D occlusion, explaining the 5.05-m bed-to-wardrobe difference. Both synchronized scenarios complete 28/28 needs. Colored edges denote the facade. Doors are represented by fixed geometry.}
\label{fig:wardrobe-facade}
\end{figure*}

\subsection{Three assessments on the identical saved layouts}
\label{sec:efd-same-layouts}

\begin{table*}[t]\centering\small
\caption{Same-layout E/F/D comparison, A $\rightarrow$ B. D is household pending-need latency in need-seconds in the prespecified synchronized original-speed condition. All needs are fulfilled. E and F use their declared score scales; D retains fulfilled-need counts.}
\label{tab:efd-same-layouts}
\begin{tabular}{lrrrr}\toprule
Intervention & E $\downarrow$ & $F_{\mathrm{geom}}\uparrow$ & D $\downarrow$ & $\Delta$D (B--A)\\\midrule
Wardrobe facade & $22\to22$ & $43.52\to43.52$ & $3452.917\to3461.167$ & $+8.250$\\
Wardrobe shift & $28\to28$ & $74.07\to74.07$ & $2662.942\to2663.067$ & $+0.125$\\
Sofa shift & $21\to21$ & $40.12\to40.12$ & $2661.958\to2662.000$ & $+0.042$\\
Assigned table side$^*$ & $20\to20$ & $43.52\to43.52$ & $2685.208\to2668.375$ & $-16.833$\\\bottomrule
\end{tabular}
\par\smallskip\footnotesize $^*$Assigned-interface diagnostic for a symmetric object. The facade study includes extra entry/balcony needs; compare D within each pair.
\end{table*}
\paragraph{Matched geometry and fixed implementations.}
We recompute static E and geometric Feng Shui on all eight saved layouts above and join the previously audited dynamic outcomes. This rescore reuses the same geometry and audited dynamic executions. The adapter retains every room polygon, furniture footprint, facing, layer and support link. Source opening endpoints are projected by at most 1\,cm to their room boundary and represented by the archived evaluator's 8-cm inward rectangles. A generic storage cabinet is explicitly mapped to its enclosed-storage front-access type. Separate checks verify source and code hashes, geometric correspondence, static facts, score arithmetic and dynamic-result identity.

E is the archived critic penalty $3n_{\mathrm{critical}}+n_{\mathrm{advisory}}$ (lower is better), accompanied by its full findings. It includes implementation-specific recommendations. $F_{\mathrm{geom}}$ uses version 3.0.0 with the original (v1) geometry predicates; the complete HANFU rubric has separate criterion definitions. Its fixed active criteria are bedroom position (F1), living-room position (F3), circulation (F5), bed/door axis (F7), and density/function (F10), with weights $(2,2,2,2,1)$ and maxima $(4,3,4,2,3)$. These version-specific F5/F10 meanings differ from CoHABIT's complete HANFU rubric. Each layout has all 15 applicable room-level ratings. We average within each criterion and normalize its mean as $(\bar f_k-1)/(m_k-1)$, then take the fixed weighted average on a 0--100 scale. The score covers the declared geometric criteria; compass and elemental attributes remain unspecified.



\paragraph{What each assessment contributes.}
E retains explicit spatial findings. For the sofa, the living-room navigability diagnostic changes from 0.812 to 0.798 while its advisory severity and total penalty remain unchanged. An aggregate E tie can coexist with changed geometric diagnostics. The assessed spatial-preference relations and all their ratings are unchanged within each pair: these interventions preserve the assessed preference categories. F records the same declared preference profile in both alternatives.

D adds routine-dependent discrimination to those static ties. In the directional wardrobe example, equal E and $F_{\mathrm{geom}}$ coexist with a verified 5.05-m access detour and 8.25 extra household need-seconds, distributed equally between residents. Adjacent route changes compensate, linking local path differences to the full-routine total. Together the views separate spatial findings, preference categories and execution consequences on the same input. They illustrate complementary evidence, without requiring every assessment to change or treating small discretization-scale residuals as established comfort differences. The F audit independently checks back support, entry view, bed/door axis, density and aggregation; circulation is evaluated by the pinned producer algorithm.

\subsection{Contrasting spatial, preference and routine evidence}
\label{sec:efd-contrasts}


Two controlled furnishing interventions in apartment~026 are selected for changed E and preference facts before observing their new dynamic outcomes. Both retain source dimensions, all objects, all needs and complete target reachability, with no added overlap or outside-room placement. Earlier candidates and their rejection reasons remain archived. These explanatory interventions share one baseline apartment. The living-room intervention shifts the sofa and a chair 0.20\,m east and the coffee table 0.20\,m east/0.50\,m south. The bedroom intervention turns the bed $180^\circ$ and shifts it 0.60\,m north.

\paragraph{Physical preference checks.}
For these pairs, $F_{\mathrm{geom}}$ uses a pinned physical-predicate revision: door-view rays stay inside the room polygon, and rear support contacts only solid source walls. The five criteria, weights and score thresholds above are unchanged. This addresses limitations of the archived v1 geometry predicates used in Table~\ref{tab:efd-same-layouts}, whose historical scores are retained with their original version. Correcting the living-room ray that crossed a concave wall changes apartment~026's baseline from 74.07 to 62.96. No new pair mixes F versions. Independent checks cover source geometry, support, wall-aware visibility, door axis, density and score arithmetic; circulation retains the pinned producer implementation. This score covers the specified geometric preference subset.

\paragraph{Matched execution and audit.}
Each intervention has six matched conditions: solo, asynchronous and synchronous routines, each with the original speed profile or resident~0 at $0.7\times$ speed. All task chains include the six apartment zones. Twelve new B cases per method are matched to twelve previously audited, hash-pinned A observations, reusing the shared baseline.  The reference planner and neural executor each fulfill 280/280 new needs in 12/12 cases, with independent audits passing; the retained A observations also fulfill every need. Explicit external-case validation checks matched needs, profiles and calendars. Both executors yield the same costs, supporting the reported furnishing contrasts under either execution method.



\paragraph{Complementarity in the living room.}
E reports reduced chair clearance (0.64 to 0.44\,m) and changed neighboring gaps; F3 separately detects lost sofa backing (rating 2 to 1). Yet the table-to-sofa route shortens from 7.10 to 4.55\,m and sofa-to-TV from 3.125 to 2.925\,m. In the synchronized original-speed routine, B reduces total latency by 7.750 need-seconds while changing individual costs by $+11.125/-18.875$. With slower resident~0, B instead adds 28.009. The solo/asynchronous deltas are $-8.354/-16.708$ at original speed and $-11.935/-20.289$ with slower R0. Static preference, geometric access and household scheduling therefore provide distinct evidence for the same choice.

\paragraph{Complementarity in the bedroom.}
E detects a 0.45-m bed--wardrobe gap and partial obstruction of wardrobe access, while the earlier door-opening finding disappears. F7 independently detects the bed facing the door axis (rating 2 to 1). Bed-to-wardrobe distance increases from 2.300 to 4.725\,m. The synchronized original-speed total increases by 19.333, but the residents' changes are $+52.167/-32.833$; with slower R0 the total changes by $-1.167$. Solo/asynchronous changes are $+3.896/+7.792$ at original speed and $+5.565/+9.461$ with slower R0. Personal accounting resolves who benefits from these simulator-specific aggregate changes. Together, the examples show household-dependent tradeoffs among the separate criteria.

\begin{figure*}[p]\centering
{\small
\captionof{table}{Matched same-input contrasts. E is a penalty, $F_{\mathrm{geom}}^{v2}$ a preference score; $\Delta$D is B--A household pending-need latency (need-seconds). The last two columns use synchronized routines.}
\label{tab:efd-contrasts}
\begin{tabular}{lrrrr}\toprule
Intervention & E $\downarrow$ & $F_{\mathrm{geom}}^{v2}\uparrow$ & $\Delta$D original & $\Delta$D slower R0\\\midrule
Living-room arrangement & $28\to34$ & $62.96\to51.85$ & $-7.750$ & $+28.009$\\
Bed rotation/shift & $28\to29$ & $62.96\to40.74$ & $+19.333$ & $-1.167$\\\bottomrule
\end{tabular}
}
\medskip
\includegraphics[width=.94\textwidth]{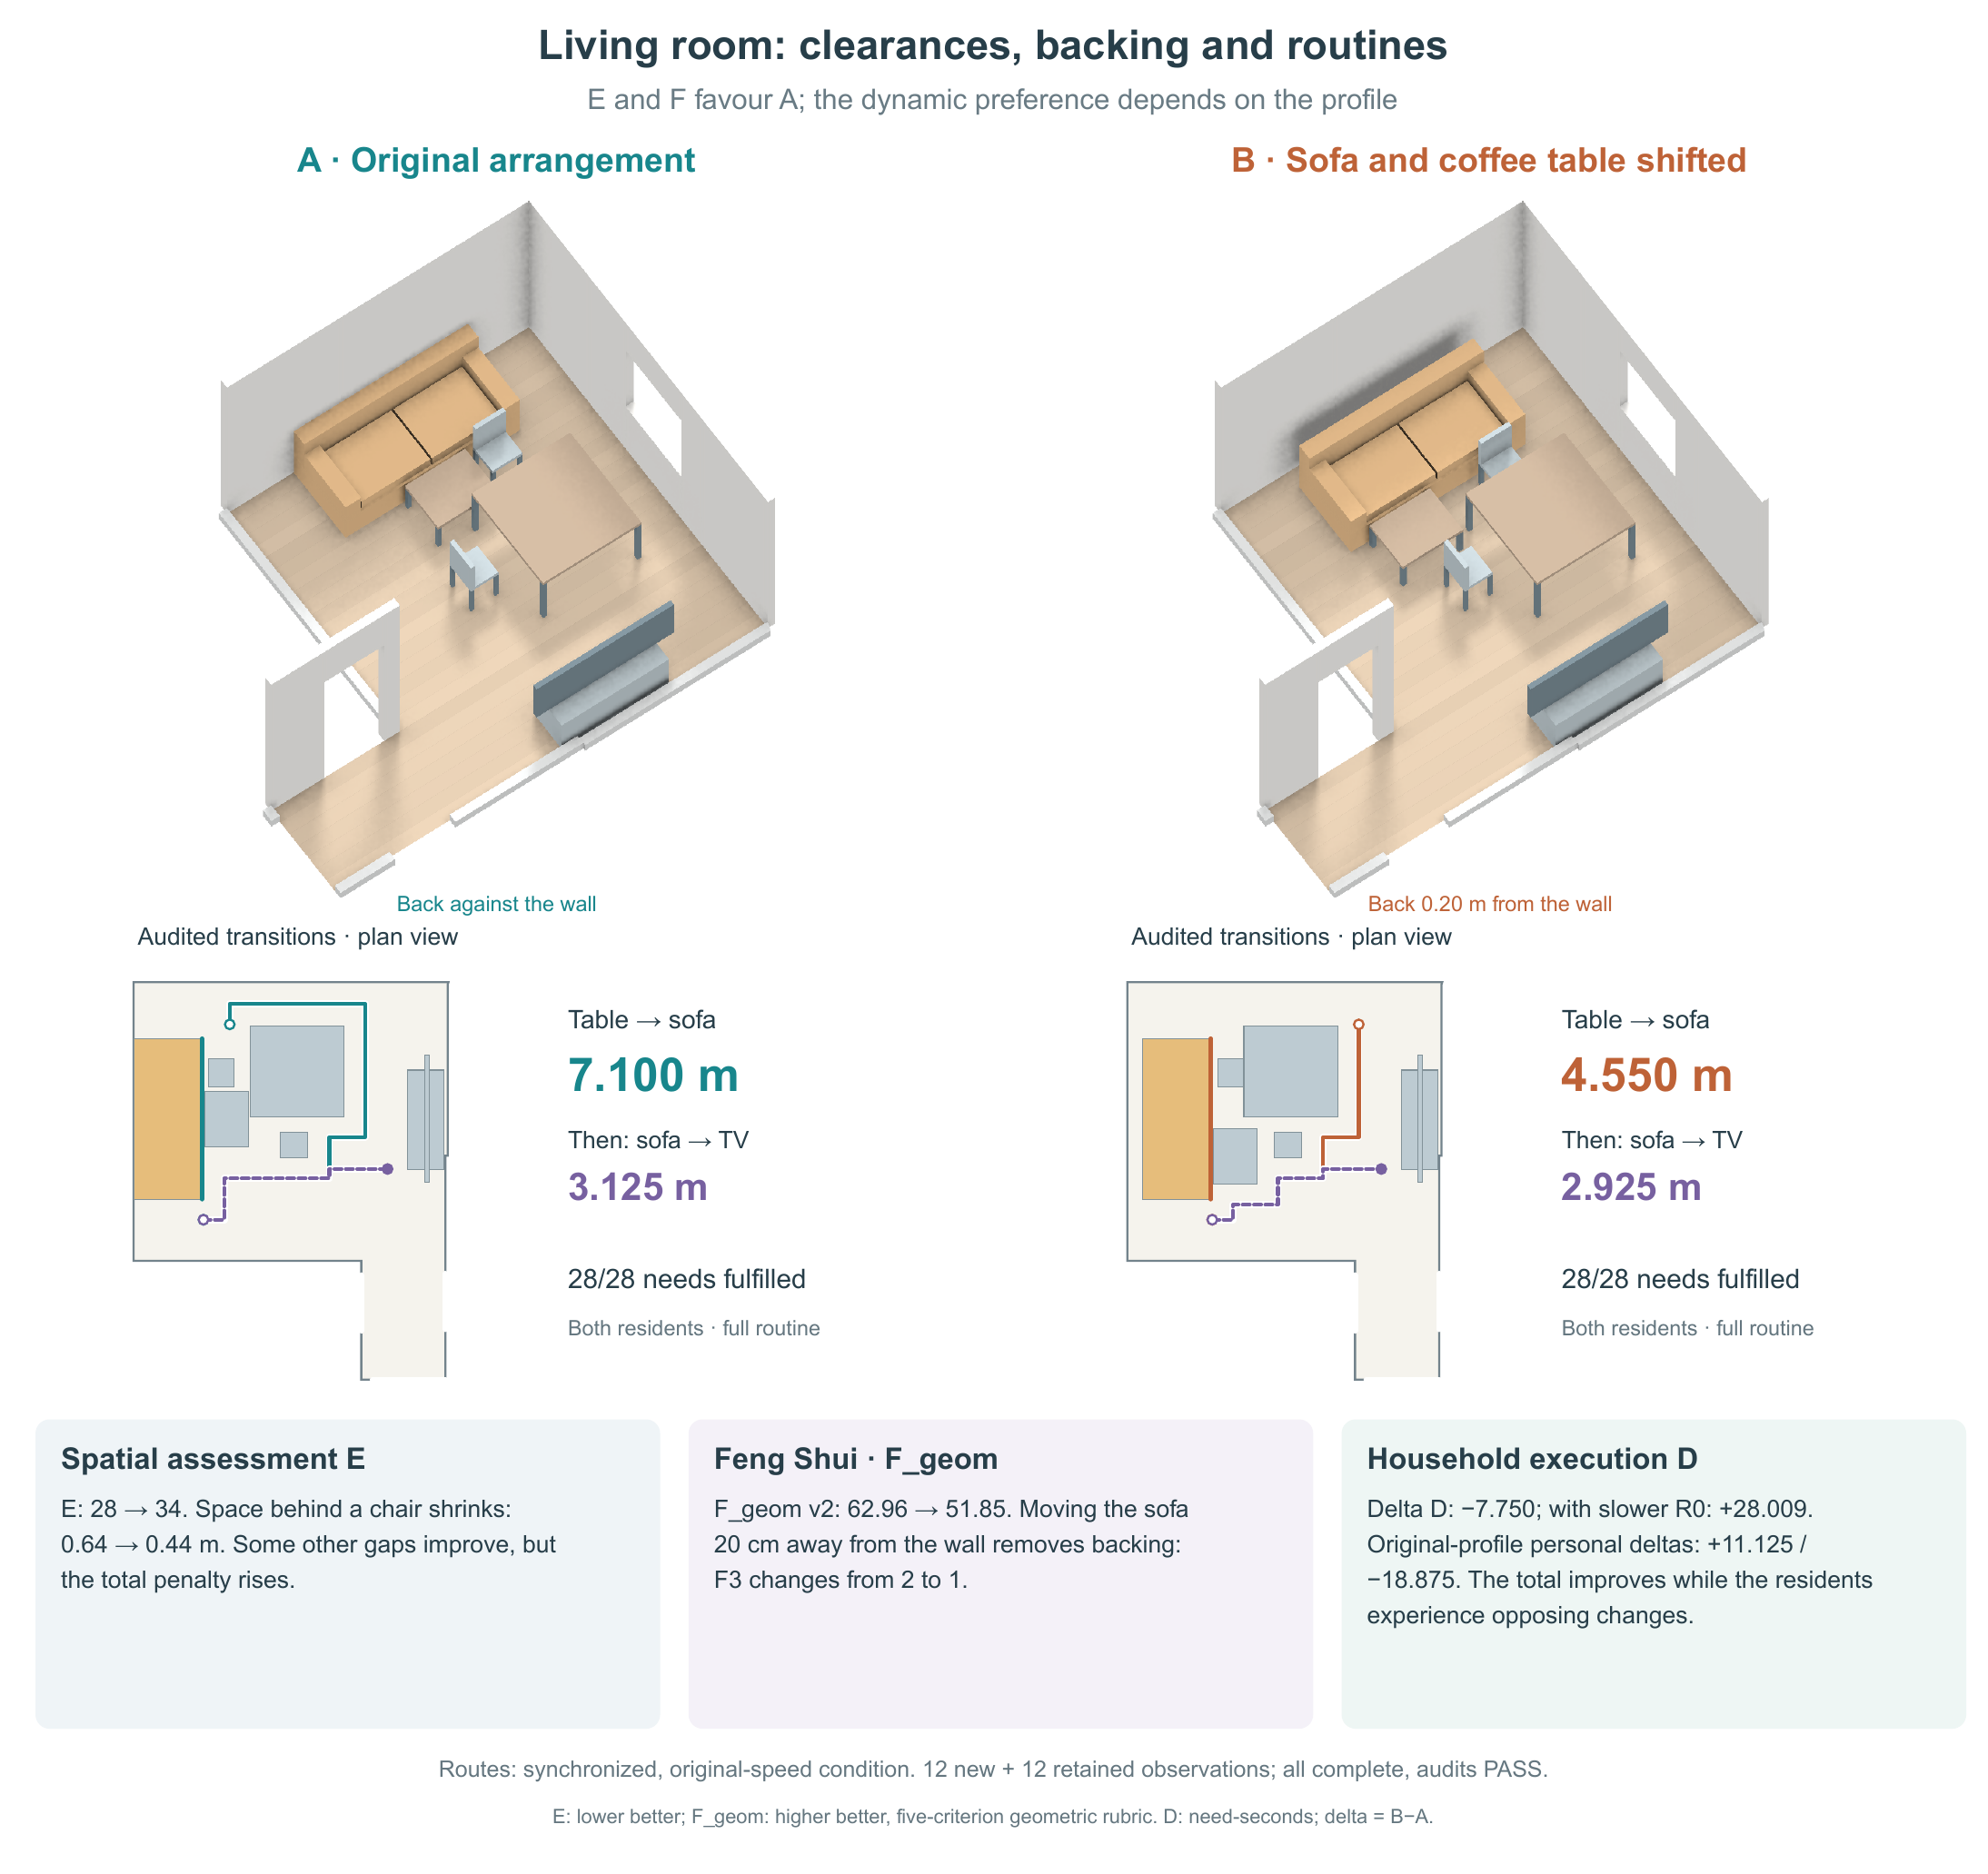}
\caption{\textbf{Static preference and routine efficiency answer different questions.} Exact source footprints and orientation are rendered from a common camera; materials and heights are illustrative. Plan insets show the same audited resident's selected transitions, with full distance-matrix and event-duration checks. Both complete synchronized cases fulfill 28/28 needs and include activities in all six rooms. The living-room intervention changes three objects jointly; D measures their combined arrangement effect.}
\label{fig:efd-sofa-backing}
\end{figure*}
\begin{figure*}[tp]\centering
\includegraphics[width=\textwidth]{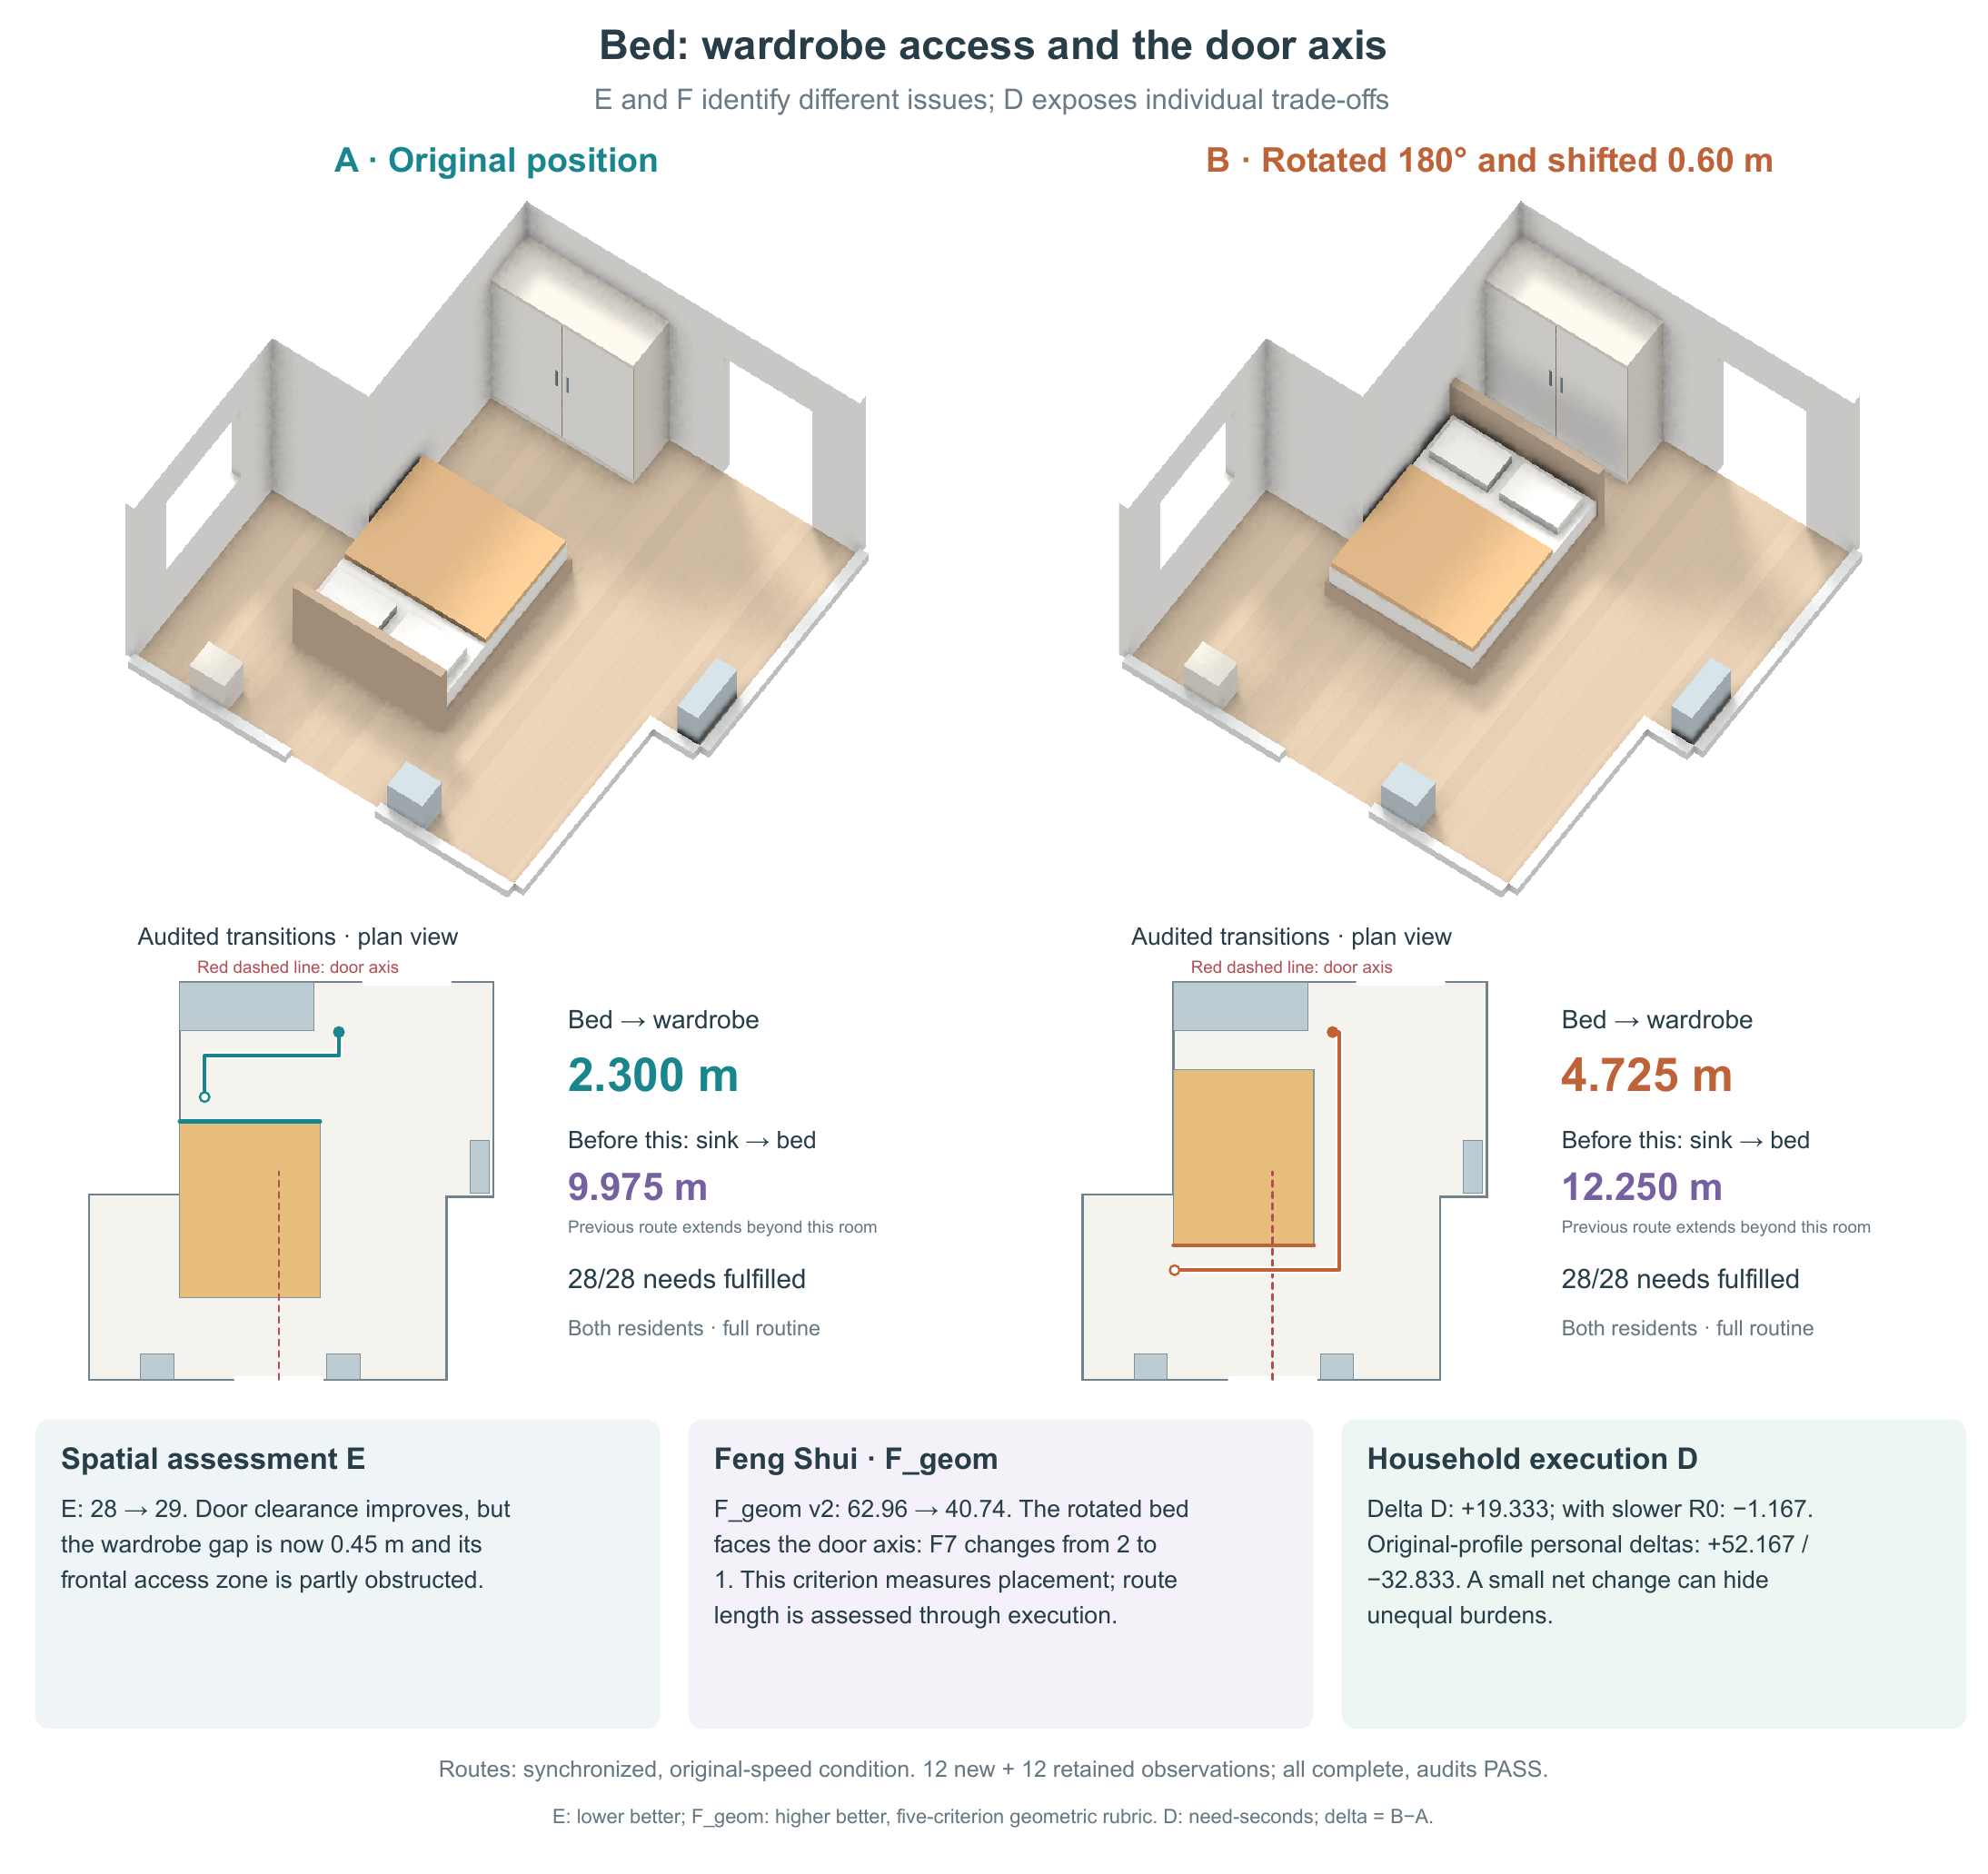}
\caption{\textbf{A directional bed connects placement, access and individual burdens.} Bed facing and location change together; all other furniture remains fixed. The plan view shows the audited bed-to-wardrobe transition; the preceding sink-to-bed distance includes travel outside this room. Both variants complete 28/28 needs in the illustrated condition. The accompanying data retain all six prespecified conditions, including the slower-resident profile; the figure shows the synchronized original-speed condition.}
\label{fig:efd-bed-axis}
\end{figure*}
